# Supplementary material for: Reference CC3 Excitation Energies for Organic Chromophores: Benchmarking TD-DFT, BSE/$GW$ and Wave Function Methods
Source: arXiv:2407.09060 ancillary file (2024-08-26)
Supplement: Supplementary file 1 [file ChromCC3-SI.pdf]

# Supporting Information for "Reference CC3 Excitation Energies for Organic Chromophores: Benchmarking TD-DFT, BSE/$GW$ and Wave Function Methods"

Iryna Knysh,[†] Filippo Lipparini,[‡] Aymeric Blondel,[†] Ivan Duchemin,[¶] Xavier Blase,[§] Pierre-François Loos,[*,‖] and Denis Jacquemin[*,†,⊥]

†*Nantes Université, CNRS, CEISAM UMR 6230, F-44000 Nantes, France*

‡*Dipartimento di Chimica e Chimica Industriale, University of Pisa, Via Moruzzi 3, 56124 Pisa, Italy*

¶*Université Grenoble Alpes, CEA, IRIG-MEM-L Sim, 38054 Grenoble, France*

§*Université Grenoble Alpes, CNRS, Institut NEEL, F-38042 Grenoble, France*

‖*Laboratoire de Chimie et Physique Quantiques, Université de Toulouse, CNRS, UPS, France*

⊥*Institut Universitaire de France (IUF), F-75005 Paris, France*

E-mail: loos@irsamc.ups-tlse.fr; Denis.Jacquemin@univ-nantes.fr

# S1 State characteristics

Table S1: ES features: i) single excitation character, $\%T_1$, obtained at CC3/aug-cc-pVDZ level: ii) LR-CCSD/aug-cc-pVTZ oscillator strength; iii) state extension determined at ADC(2)/aug-cc-pVTZ level, and iv) change as compared to the corresponding ground state; v) dominant HF/aug-cc-pVTZ contribution(s) as given by EOM-CCSD/aug-cc-pVTZ.

| Compound | State | $\%T_1$ (%) | $f$ | $\langle r^2 \rangle$ (au) | $\Delta\langle r^2 \rangle$ (au) | MO |
|---|---|---|---|---|---|---|
| Anthracene | $^1B_{1u}$ $(\pi \to \pi^\star)$ | 89.8 | 0.074 | 2837 | 3 | 47→53 |
| | $^1B_{2u}$ $(\pi \to \pi^\star)$ | 85.4 | 0.000 | 2836 | 2 | 46→53/47→64 |
| | $^1B_{3g}$ $(\pi \to \pi^\star)$ | 78.5 | | 2838 | 4 | 45→53/47→67 |
| | $^1B_{2g}$ (Ryd) | 92.4 | | 2883 | 49 | 47→48 |
| | $^1B_{1u}$ $(\pi \to \pi^\star)$ | 86.8 | 0.001 | 2841 | 7 | 47→58/47→88/47→66 |
| | $^1B_{3g}$ $(\pi \to \pi^\star)$ | 89.6 | | 2836 | 2 | 47→67/47→84/45→53 |
| | $^1A_g$ $(\pi \to \pi^\star)$ | 75.1 | | 2836 | 2 | 45→64/46→67/43→53/46→84 |
| | $^1B_{3u}$ (Ryd) | 92.3 | 0.002 | 2898 | 64 | 47→50 |
| | $^1A_u$ (Ryd) | 92.1 | | 2929 | 95 | 47→49 |
| | $^1B_{2u}$ $(\pi \to \pi^\star)$ | 89.8 | 2.322 | 2839 | 5 | 47→64/46→53 |
| | $^3B_{1u}$ $(\pi \to \pi^\star)$ | 97.3 | | 2835 | 1 | 47→53 |
| | $^3B_{3g}$ $(\pi \to \pi^\star)$ | 97.6 | | 2836 | 2 | 45→53/47→67/47→84 |
| | $^3B_{2u}$ $(\pi \to \pi^\star)$ | 96.1 | | 2835 | 1 | 46→53/47→64 |
| Anthraquinone | $^1B_{1g}$ $(n \to \pi^\star)$ | 87.1 | | 3266 | 1 | 50→55 |
| | $^1A_u$ $(n \to \pi^\star)$ | 86.4 | | 3266 | 1 | 49→55/50→61 |
| | $^1A_g$ $(\pi \to \pi^\star)$ | 85.5 | | 3262 | -3 | 54→55/51→61 |
| | $^1B_{2u}$ $(\pi \to \pi^\star)$ | 85.3 | 0.056 | 3263 | -2 | 52→55/53→61 |
| | $^1B_{3g}$ $(\pi \to \pi^\star)$ | 88.1 | | 3259 | -6 | 53→55 |
| | $^1B_{1u}$ $(\pi \to \pi^\star)$ | 87.7 | 0.196 | 3262 | -3 | 51→55/54→61 |
| | $^1B_{2u}$ $(\pi \to \pi^\star)$ | 87.0 | 0.853 | 3265 | 0 | 53→61/52→55 |
| | $^3B_{1g}$ $(n \to \pi^\star)$ | 96.3 | | 3266 | 1 | 50→55/49→61 |
| | $^3A_u$ $(n \to \pi^\star)$ | 96.3 | | 3265 | 0 | 49→55/50→61 |
| | $^3B_{1u}$ $(\pi \to \pi^\star)$ | 97.7 | | 3265 | 0 | 51→55/54→61/53→70 |
| | $^3B_{3g}$ $(\pi \to \pi^\star)$ | 97.4 | | 3263 | -2 | 53→55/52→61/51→70 |
| | $^3A_g$ $(\pi \to \pi^\star)$ | 96.6 | | 3261 | -4 | 54→55 |
| Aza-BODIPY | $^1B_2$ $(\pi \to \pi^\star)$ | 84.3 | 0.481 | 2269 | 0 | 49→50/48→50 |
| | $^1B_2$ $(\pi \to \pi^\star)$ | 79.9 | 0.205 | 2269 | 0 | 48→50/49→50 |
| | $^1A_1$ $(\pi \to \pi^\star)$ | 75.4 | 0.040 | 2267 | -2 | 47→50 |
| | $^1B_1$ $(n \to \pi^\star)$ | 88.8 | 0.002 | 2274 | 5 | 45→50 |
| | $^3B_2$ $(\pi \to \pi^\star)$ | 97.5 | | 2269 | 0 | 49→50 |
| | $^3B_2$ $(\pi \to \pi^\star)$ | 95.5 | | 2268 | -1 | 48→50 |
| | $^3A_1$ $(\pi \to \pi^\star)$ | 95.3 | | 2269 | 0 | 47→50 |
| | $^3B_1$ $(n \to \pi^\star)$ | 96.8 | | 2274 | 5 | 45→50 |
| Azobenzene | $^1B_g$ $(n \to \pi^\star)$ | 90.6 | | 3898 | 9 | 44→54 |
| | $^1B_u$ $(\pi \to \pi^\star)$ | 88.7 | 0.727 | 3879 | -10 | 48→54 |
| | $^1A_g$ $(\pi \to \pi^\star)$ | 84.4 | | 3882 | -7 | 46→54 |
| | $^1B_u$ $(\pi \to \pi^\star)$ | 85.1 | 0.066 | 3882 | -7 | 47→54 |
| | $^1A_g$ $(\pi \to \pi^\star)$ | 82.8 | | 3877 | -12 | 45→54 |
| | $^3B_g$ $(n \to \pi^\star)$ | 97.7 | | 3896 | 7 | 44→54/44→96 |
| | $^3B_u$ $(\pi \to \pi^\star)$ | 97.3 | | 3884 | -5 | 48→54 |
| | $^3A_g$ $(\pi \to \pi^\star)$ | 97.7 | | 3886 | -3 | 45→54/48→88 |
| | $^3B_u$ $(\pi \to \pi^\star)$ | 96.3 | | 3882 | -7 | 47→54/46→64/46→73 |
| | $^3A_g$ $(\pi \to \pi^\star)$ | 96.2 | | 3883 | -6 | 46→54 |
| BODIPY | $^1B_2$ $(\pi \to \pi^\star)$ | 85.5 | 0.524 | 2321 | -1 | 49→50 |
| | $^1B_2$ $(\pi \to \pi^\star)$ | 81.8 | 0.161 | 2321 | -1 | 48→50 |
| | $^1A_1$ $(\pi \to \pi^\star)$ | 79.1 | 0.044 | 2320 | -2 | 47→50 |
| | $^3B_2$ $(\pi \to \pi^\star)$ | 97.4 | | 2321 | -1 | 49→50 |
| | $^3B_2$ $(\pi \to \pi^\star)$ | 96.0 | | 2321 | -1 | 48→50 |
| | $^3A_1$ $(\pi \to \pi^\star)$ | 96.0 | | 2322 | 0 | 47→50/46→50 |
| Coumarin | $^1A'$ $(\pi \to \pi^\star)$ | 86.3 | 0.100 | 1587 | 1 | 38→44/37→44 |
| | $^1A''$ $(n \to \pi^\star)$ | 85.3 | 0.000 | 1578 | -8 | 35→44/35→60 |
| | $^1A'$ $(\pi \to \pi^\star)$ | 88.1 | 0.197 | 1586 | 0 | 37→44/38→44/38→50 |
| | $^3A'$ $(\pi \to \pi^\star)$ | 97.7 | | 1585 | -1 | 38→44 |
| | $^3A'$ $(\pi \to \pi^\star)$ | 97.2 | | 1588 | 2 | 37→44/37→50/37→52/38→44 |
| | $^3A''$ $(n \to \pi^\star)$ | 95.5 | | 1578 | -8 | 35→44/35→60 |

Table S2: ES features. See caption of Table S1 for more details.

| Compound | State | $\%T_1$ (%) | $f$ | $\langle r^2 \rangle$ (au) | $\Delta\langle r^2 \rangle$ (au) | MO |
|---|---|---|---|---|---|---|
| Cyclazine | $^1A_2'$ $(\pi \to \pi^\star)$ | 87.2 | | 1947 | -4 | 44→51 |
| | $^1E'$ $(\pi \to \pi^\star)$ | 84.3 | 0.458 | 1952 | 1 | 44→56/44→67/44→61 & sym |
| | $^1A_1''$ (Ryd) | 91.2 | | 1994 | 43 | 44→45 |
| | $^1E''$ (Ryd) | 91.2 | | 2032 | 81 | 44→47 & sym |
| | $^3A_2'$ $(\pi \to \pi^\star)$ | 96.1 | | 1947 | -4 | 44→51 |
| | $^3E'$ $(\pi \to \pi^\star)$ | 96.4 | | 1949 | -2 | 44→56/44→67/44→61 & sym |
| | $^3A_1''$ (Ryd) | 96.8 | | 1993 | 42 | 44→45/44→70 |
| | $^3E''$ (Ryd) | 96.8 | | 2031 | 80 | 44→47 & sym |
| Heptazine | $^1A_2'$ $(\pi \to \pi^\star)$ | 86.3 | | 1707 | -1 | 44→45 |
| | $^1A_1''$ $(n \to \pi^\star)$ | 85.9 | | 1705 | -2 | 41→45 |
| | $^1E''$ $(n \to \pi^\star)$ | 86.7 | | 1705 | -2 | 43→45 & sym |
| | $^1E'$ $(\pi \to \pi^\star)$ | 84.4 | 0.550 | 1708 | 0 | 44→51/44→56 & sym |
| | $^3A_2'$ $(\pi \to \pi^\star)$ | 95.7 | | 1707 | -1 | 44→45 |
| | $^3E''(\pi \to \pi^\star)$ | 96.1 | | 1708 | 0 | 44→51/44→56 & sym |
| | $^3A_1''$ $(n \to \pi^\star)$ | 94.8 | | 1705 | -2 | 41→45 |
| | $^3E''$ $(n \to \pi^\star)$ | 95.0 | | 1705 | -2 | 43→45 & sym |
| Naphthalimide | $^1B_2$ $(\pi \to \pi^\star)$ | 85.5 | 0.018 | 2629 | 2 | 50→53/51→63 |
| | $^1B_1$ $(n \to \pi^\star)$ | 84.5 | 0.000 | 2623 | -4 | 47→53 |
| | $^1A_1$ $(\pi \to \pi^\star)$ | 88.8 | 0.218 | 2628 | 1 | 51→53 |
| | $^1A_2$ $(n \to \pi^\star)$ | 85.2 | | 2623 | -4 | 46→53 |
| | $^3A_1$ $(\pi \to \pi^\star)$ | 97.3 | | 2628 | 1 | 51→53 |
| | $^3B_2$ $(\pi \to \pi^\star)$ | 96.7 | | 2628 | 1 | 50→53 |
| | $^3B_1$ $(n \to \pi^\star)$ | 95.1 | | 2623 | -4 | 47→53 |
| | $^3B_2$ $(\pi \to \pi^\star)$ | 97.2 | | 2627 | 0 | 49→53/51→63/50→53/51→68 |
| | $^3A_2$ $(n \to \pi^\star)$ | 95.6 | | 2623 | -4 | 46→53 |
| Naphthoquinone | $^1B_1$ $(n \to \pi^\star)$ | 86.1 | 0.000 | 1764 | -2 | 38→42 |
| | $^1A_2$ $(n \to \pi^\star)$ | 85.1 | | 1764 | -2 | 37→42 |
| | $^1A_1$ $(\pi \to \pi^\star)$ | 85.7 | 0.040 | 1768 | 2 | 41→42 |
| | $^1B_2$ $(\pi \to \pi^\star)$ | 88.0 | 0.023 | 1768 | 2 | 40→42 |
| | $^1A_2$ $(n \to \pi^\star)$ | 80.3 | | 1765 | -1 | 38→49/38→50/37→42 |
| | $^1A_1$ $(\pi \to \pi^\star)$ | 86.2 | 0.193 | 1769 | 3 | 40→49/41→42/40→50/41→56 |
| | $^1B_2$ $(\pi \to \pi^\star)$ | 88.3 | 0.322 | 1765 | -1 | 39→42 |
| | $^3B_1$ $(n \to \pi^\star)$ | 96.2 | | 1764 | -2 | 38→42 |
| | $^3A_2$ $(n \to \pi^\star)$ | 96.1 | | 1763 | -3 | 37→42 |
| | $^3B_2$ $(\pi \to \pi^\star)$ | 97.7 | | 1765 | -1 | 39→42/40→42 |
| | $^3B_2$ $(\pi \to \pi^\star)$ | 97.6 | | 1767 | 1 | 40→42/39→42 |
| | $^3A_1$ $(\pi \to \pi^\star)$ | 96.4 | | 1767 | 1 | 41→42 |
| Phenazine | $^1B_{1u}$ $(n \to \pi^\star)$ | 87.6 | 0.002 | 2688 | 7 | 44→48 |
| | $^1B_{3u}$ $(\pi \to \pi^\star)$ | 88.1 | 0.050 | 2676 | -5 | 47→48 |
| | $^1B_{2u}$ $(\pi \to \pi^\star)$ | 85.5 | 0.146 | 2681 | 0 | 46→48/47→59 |
| | $^1B_{1g}$ $(\pi \to \pi^\star)$ | 82.4 | | 2676 | -5 | 45→48 |
| | $^1B_{2g}$ $(n \to \pi^\star)$ | 77.6 | | 2690 | 9 | 41→48 |
| | $^1A_u$ $(\pi \to \pi^\star)$ | 85.8 | | 2691 | 10 | 44→59/44→67 |
| | $^3B_{3u}$ $(\pi \to \pi^\star)$ | 97.1 | | 2680 | -1 | 47→48 |
| | $^3B_{1u}$ $(n \to \pi^\star)$ | 96.4 | | 2686 | 5 | 44→48 |
| | $^3B_{2u}$ $(\pi \to \pi^\star)$ | 96.7 | | 2679 | -2 | 46→48 |
| | $^3B_{1g}$ $(\pi \to \pi^\star)$ | 97.4 | | 2681 | 0 | 45→48/47→65/47→82 |
| Phthalimide | $^1B_1$ $(n \to \pi^\star)$ | 87.9 | 0.000 | 1489 | -3 | 35→42 |
| | $^1A_1$ $(\pi \to \pi^\star)$ | 86.1 | 0.013 | 1494 | 2 | 38→42/37→46 |
| | $^1A_2$ $(n \to \pi^\star)$ | 87.3 | | 1488 | -4 | 34→42 |
| | $^1B_2$ $(\pi \to \pi^\star)$ | 88.8 | 0.000 | 1493 | 1 | 37→42/36→42 |
| | $^1B_2$ $(\pi \to \pi^\star)$ | 87.4 | 0.197 | 1492 | 0 | 36→42/37→42/38→46 |
| | $^1A_2$ $(n \to \pi^\star)$ | 81.8 | | 1491 | -1 | 35→46/35→45/34→42 |
| | $^1A_1$ $(\pi \to \pi^\star)$ | 89.1 | 0.744 | 1495 | 3 | 37→46/38→42/37→45 |
| | $^3B_2$ $(\pi \to \pi^\star)$ | 98.0 | | 1493 | 1 | 37→42/38→46 |
| | $^3B_1$ $(n \to \pi^\star)$ | 96.3 | | 1488 | -4 | 35→42 |
| | $^3A_1$ $(\pi \to \pi^\star)$ | 96.8 | | 1493 | 1 | 38→42/37→46 |
| | $^3B_2$ $(\pi \to \pi^\star)$ | 97.0 | | 1491 | -1 | 38→46/37→42/38→45 |
| | $^3A_2$ $(n \to \pi^\star)$ | 96.4 | | 1489 | -3 | 34→42 |
| | $^3B_2$ $(\pi \to \pi^\star)$ | 96.8 | | 1492 | -2 | 36→42 |
| Tolan | $^1B_{2u}$ $(\pi \to \pi^\star)$ | 85.6 | 0.000 | 4471 | 3 | 46→56/47→62/47→84 |
| | $^1B_{3g}$ $(\pi \to \pi^\star)$ | 85.4 | | 4471 | 3 | 45→56/47→65/47→71 |
| | $^1B_{1u}$ $(\pi \to \pi^\star)$ | 91.4 | 1.005 | 4474 | 6 | 47→56 |
| | $^1A_u$ $(\pi \to \pi^\star)$ | 90.8 | | 4487 | 19 | 43→56 |
| | $^1B_{3u}$ (Ryd) | 92.8 | 0.002 | 4503 | 35 | 47→48/47→51 |
| | $^3B_{1u}$ $(\pi \to \pi^\star)$ | 97.6 | | 4471 | 3 | 47→56 |
| | $^3A_g$ $(\pi \to \pi^\star)$ | 98.2 | | 4469 | 1 | 45→84/44→56/47→73/47→87 |

# S2 Data for defining the TBE

Table S3: VTEs computed with various methods and three basis sets. All values are in eV.

| Compound | State | CCSD | | | CCSDR(3) | | CC3 | | | CCSDT |
|---|---|---|---|---|---|---|---|---|---|---|
| | | Pop | AVDZ | AVTZ | AVDZ | AVTZ | Pop | AVDZ | AVTZ | Pop |
| Anthracene | $^1B_{1u}$ $(\pi \rightarrow \pi^\star)$ | 4.193 | 4.010 | 3.979 | 3.858 | 3.839 | 3.980 | 3.795 | 3.757 | |
| | $^1B_{2u}$ $(\pi \rightarrow \pi^\star)$ | 3.984 | 3.940 | 3.931 | 3.896 | 3.895 | 3.844 | 3.805 | 3.782 | |
| | $^1B_{3g}$ $(\pi \rightarrow \pi^\star)$ | 5.744 | 5.611 | 5.602 | 5.317 | 5.296 | 5.157 | 5.043 | 5.012 | |
| | $^1B_{2g}$ (Ryd) | 5.444 | 5.039 | 5.123 | 5.027 | 5.107 | 5.323 | 4.998 | | |
| | $^1B_{1u}$ $(\pi \rightarrow \pi^\star)$ | 5.653 | 5.499 | 5.504 | 5.398 | 5.407 | 5.432 | 5.298 | 5.284 | |
| | $^1B_{3g}$ $(\pi \rightarrow \pi^\star)$ | 5.648 | 5.504 | 5.485 | 5.345 | 5.342 | 5.498 | 5.335 | | |
| | $^1A_g$ $(\pi \rightarrow \pi^\star)$ | 5.752 | 5.709 | 5.704 | 5.558 | 5.554 | 5.360 | 5.343 | 5.319 | |
| | $^1B_{3u}$ (Ryd) | 5.558 | 5.330 | 5.423 | 5.322 | 5.408 | 5.417 | 5.293 | | |
| | $^1A_u$ (Ryd) | 5.765 | 5.422 | 5.511 | 5.402 | 5.483 | 5.633 | 5.370 | | |
| | $^1B_{2u}$ $(\pi \rightarrow \pi^\star)$ | 5.829 | 5.722 | 5.702 | 5.554 | 5.533 | 5.622 | 5.514 | 5.476 | |
| | $^3B_{1u}$ $(\pi \rightarrow \pi^\star)$ | 2.235 | 2.224 | 2.217 | | | 2.317 | 2.294 | | |
| | $^3B_{3g}$ $(\pi \rightarrow \pi^\star)$ | 3.660 | 3.640 | 3.620 | | | 3.695 | 3.675 | | |
| | $^3B_{2u}$ $(\pi \rightarrow \pi^\star)$ | 3.903 | 3.838 | 3.808 | | | 3.808 | 3.738 | | |
| Anthraquinone | $^1B_{1g}$ $(n \rightarrow \pi^\star)$ | 3.516 | 3.465 | 3.485 | 3.337 | 3.343 | 3.293 | 3.220 | | |
| | $^1A_u$ $(n \rightarrow \pi^\star)$ | 3.731 | 3.683 | 3.701 | 3.572 | 3.574 | 3.536 | 3.464 | | |
| | $^1A_g$ $(\pi \rightarrow \pi^\star)$ | 4.511 | 4.483 | 4.472 | 4.435 | 4.328 | 4.242 | 4.211 | | |
| | $^1B_{2u}$ $(\pi \rightarrow \pi^\star)$ | 4.504 | 4.477 | 4.462 | 4.346 | 4.336 | 4.251 | 4.229 | | |
| | $^1B_{3g}$ $(\pi \rightarrow \pi^\star)$ | 4.732 | 4.656 | 4.627 | 4.471 | 4.455 | 4.400 | 4.337 | | |
| | $^1B_{1u}$ $(\pi \rightarrow \pi^\star)$ | 5.452 | 5.372 | 5.344 | 5.218 | 5.196 | 5.192 | 5.123 | | |
| | $^1B_{2u}$ $(\pi \rightarrow \pi^\star)$ | 5.868 | 5.745 | 5.734 | 5.522 | 5.510 | 5.537 | 5.418 | | |
| | $^3B_{1g}$ $(n \rightarrow \pi^\star)$ | 3.190 | 3.139 | 3.165 | | | 3.059 | 2.984 | | |
| | $^3A_u$ $(n \rightarrow \pi^\star)$ | 3.407 | 3.360 | 3.384 | | | 3.311 | 3.238 | | |
| | $^3B_{1u}$ $(\pi \rightarrow \pi^\star)$ | 3.354 | 3.361 | 3.347 | | | 3.454 | 3.457 | | |
| | $^3B_{3g}$ $(\pi \rightarrow \pi^\star)$ | 3.489 | 3.488 | 3.466 | | | 3.520 | 3.520 | | |
| | $^3A_g$ $(\pi \rightarrow \pi^\star)$ | 3.901 | 3.866 | 3.840 | | | 3.802 | 3.766 | | |
| Aza-BODIPY | $^1B_2$ $(\pi \rightarrow \pi^\star)$ | 2.642 | 2.629 | 2.634 | | | 2.531 | 2.525 | 2.518 | 2.525 |
| | $^1B_2$ $(\pi \rightarrow \pi^\star)$ | 3.877 | 3.824 | 3.823 | | | 3.469 | 3.419 | 3.398 | 3.528 |
| | $^1A_1$ $(\pi \rightarrow \pi^\star)$ | 3.957 | 3.932 | 3.942 | | | 3.446 | 3.427 | 3.407 | 3.502 |
| | $^1B_1$ $(n \rightarrow \pi^\star)$ | 4.161 | 4.093 | 4.078 | | | 3.988 | 3.914 | 3.875 | 3.994 |
| | $^3B_2$ $(\pi \rightarrow \pi^\star)$ | 1.253 | 1.236 | 1.198 | | | 1.378 | 1.367 | | |
| | $^3B_2$ $(\pi \rightarrow \pi^\star)$ | 2.893 | 2.879 | 2.887 | | | 2.779 | 2.766 | | |
| | $^3A_1$ $(\pi \rightarrow \pi^\star)$ | 3.158 | 3.153 | 3.158 | | | 3.028 | 3.022 | | |
| | $^3B_1$ $(n \rightarrow \pi^\star)$ | 3.543 | 3.487 | 3.496 | | | 3.490 | 3.426 | | |
| Azobenzene | $^1B_g$ $(n \rightarrow \pi^\star)$ | 3.102 | 3.024 | 2.987 | 2.956 | 2.922 | 3.004 | 2.917 | 2.871 | |
| | $^1B_u$ $(\pi \rightarrow \pi^\star)$ | 4.572 | 4.488 | 4.460 | 4.336 | 4.315 | 4.348 | 4.271 | 4.231 | |
| | $^1A_g$ $(\pi \rightarrow \pi^\star)$ | 4.766 | 4.732 | 4.722 | 4.582 | 4.572 | 4.506 | 4.472 | 4.439 | |
| | $^1B_u$ $(\pi \rightarrow \pi^\star)$ | 4.793 | 4.750 | 4.734 | 4.589 | 4.576 | 4.526 | 4.482 | 4.446 | |
| | $^1A_g$ $(\pi \rightarrow \pi^\star)$ | 5.745 | 5.660 | 5.639 | 5.415 | 5.400 | 5.287 | 5.224 | 5.185 | |
| | $^3B_g$ $(n \rightarrow \pi^\star)$ | 2.392 | 2.329 | 2.317 | | | 2.369 | 2.298 | | |
| | $^3B_u$ $(\pi \rightarrow \pi^\star)$ | 2.796 | 2.783 | 2.771 | | | 2.827 | 2.812 | | |
| | $^3A_g$ $(\pi \rightarrow \pi^\star)$ | 3.853 | 3.853 | 3.833 | | | 3.946 | 3.941 | | |
| | $^3B_u$ $(\pi \rightarrow \pi^\star)$ | 4.434 | 4.383 | 4.359 | | | 4.292 | 4.242 | | |
| | $^3A_g$ $(\pi \rightarrow \pi^\star)$ | 4.523 | 4.470 | 4.444 | | | 4.351 | 4.305 | | |
| BODIPY | $^1B_2$ $(\pi \rightarrow \pi^\star)$ | 2.902 | 2.899 | 2.908 | | | 2.785 | 2.788 | 2.781 | 2.775 |
| | $^1B_2$ $(\pi \rightarrow \pi^\star)$ | 4.215 | 4.165 | 4.175 | | | 3.822 | 3.776 | 3.760 | 3.866 |
| | $^1A_1$ $(\pi \rightarrow \pi^\star)$ | 4.348 | 4.320 | 4.336 | | | 3.900 | 3.875 | 3.861 | 3.940 |
| | $^3B_2$ $(\pi \rightarrow \pi^\star)$ | 1.827 | 1.815 | 1.794 | | | 1.892 | 1.883 | | |
| | $^3B_2$ $(\pi \rightarrow \pi^\star)$ | 3.212 | 3.201 | 3.214 | | | 3.110 | 3.097 | | |
| | $^3A_1$ $(\pi \rightarrow \pi^\star)$ | 3.427 | 3.422 | 3.433 | | | 3.335 | 3.328 | | |
| Coumarin | $^1A'$ $(\pi \rightarrow \pi^\star)$ | 4.594 | 4.529 | 4.530 | | | 4.398 | 4.329 | 4.307 | |
| | $^1A''$ $(n \rightarrow \pi^\star)$ | 5.161 | 5.118 | 5.133 | | | 4.901 | 4.821 | 4.796 | |
| | $^1A'$ $(\pi \rightarrow \pi^\star)$ | 5.322 | 5.197 | 5.173 | | | 5.132 | 5.015 | 4.980 | |
| | $^3A'$ $(\pi \rightarrow \pi^\star)$ | 3.228 | 3.213 | 3.199 | | | 3.301 | 3.278 | | |
| | $^3A'$ $(\pi \rightarrow \pi^\star)$ | 4.165 | 4.139 | 4.127 | | | 4.161 | 4.121 | | |
| | $^3A''$ $(n \rightarrow \pi^\star)$ | 4.878 | 4.836 | 4.856 | | | 4.714 | 4.635 | | |

Table S4: Data used to define the TBEs. See the caption of Table S3 for more details.

| | | CCSD | | | CCSDR(3) | | CC3 | | | CCSDT |
|---|---|---|---|---|---|---|---|---|---|---|
| Compound | State | Pop | AVDZ | AVTZ | AVDZ | AVTZ | Pop | AVDZ | AVTZ | Pop |
| Cyclazine | $^1A_2'$ $(\pi \to \pi^\star)$ | 1.073 | 1.092 | 1.090 | | | 0.974 | 0.990 | 0.978 | 0.975 |
| | $^1E'$ $(\pi \to \pi^\star)$ | 3.300 | 3.205 | 3.225 | | | 3.089 | 3.007 | 3.002 | 3.105 |
| | $^1A_1''$ (Ryd) | 3.297 | 3.087 | 3.203 | | | 3.204 | 3.070 | 3.163 | 3.204 |
| | $^1E''$ (Ryd) | 3.855 | 3.603 | 3.717 | | | 3.750 | 3.592 | 3.679 | 3.762 |
| | $^3A_2'$ $(\pi \to \pi^\star)$ | 1.185 | 1.165 | 1.154 | | | 1.142 | 1.121 | | |
| | $^3E'$ $(\pi \to \pi^\star)$ | 2.228 | 2.191 | 2.195 | | | 2.182 | 2.150 | | |
| | $^3A_1''$ (Ryd) | 3.263 | 3.061 | 3.179 | | | 3.179 | 3.051 | | |
| | $^3E''$ (Ryd) | 3.827 | 3.584 | 3.700 | | | 3.728 | 3.577 | | |
| Heptazine | $^1A_2'$ $(\pi \to \pi^\star)$ | 2.829 | 2.901 | 2.953 | | | 2.633 | 2.693 | 2.708 | 2.642 |
| | $^1A_1''$ $(n \to \pi^\star)$ | 4.303 | 4.303 | 4.333 | | | 3.973 | 3.969 | 3.958 | 4.014 |
| | $^1E''$ $(n \to \pi^\star)$ | 4.390 | 4.377 | 4.394 | | | 4.110 | 4.097 | 4.073 | 4.145 |
| | $^1E'$ $(\pi \to \pi^\star)$ | 4.827 | 4.751 | 4.789 | | | 4.521 | 4.455 | 4.452 | 4.547 |
| | $^3A_2'$ $(\pi \to \pi^\star)$ | 3.017 | 3.049 | 3.087 | | | 2.873 | 2.898 | | |
| | $^3E''(\pi \to \pi^\star)$ | 3.757 | 3.752 | 3.781 | | | 3.627 | 3.620 | | |
| | $^3A_1''$ $(n \to \pi^\star)$ | 4.271 | 4.266 | 4.295 | | | 3.972 | 3.963 | | |
| | $^3E''$ $(n \to \pi^\star)$ | 4.341 | 4.324 | 4.344 | | | 4.077 | 4.060 | | |
| Naphthalimide | $^1B_2$ $(\pi \to \pi^\star)$ | 4.261 | 4.228 | 4.220 | | | 4.085 | 4.058 | 4.033 | |
| | $^1B_1$ $(n \to \pi^\star)$ | 4.583 | 4.545 | 4.568 | | | 4.246 | 4.156 | 4.145 | |
| | $^1A_1$ $(\pi \to \pi^\star)$ | 4.532 | 4.428 | 4.406 | | | 4.292 | 4.190 | 4.155 | |
| | $^1A_2$ $(n \to \pi^\star)$ | 5.004 | 4.951 | 4.997 | | | 4.741 | 4.654 | 4.632 | |
| | $^3A_1$ $(\pi \to \pi^\star)$ | 2.750 | 2.742 | 2.735 | | | 2.800 | 2.787 | | |
| | $^3B_2$ $(\pi \to \pi^\star)$ | 3.914 | 3.869 | 3.846 | | | 3.851 | 3.808 | | |
| | $^3B_1$ $(n \to \pi^\star)$ | 4.354 | 4.308 | 4.342 | | | 4.114 | 4.026 | | |
| | $^3B_2$ $(\pi \to \pi^\star)$ | 4.200 | 4.155 | 4.132 | | | 4.188 | 4.147 | | |
| | $^3A_2$ $(n \to \pi^\star)$ | 4.751 | 4.700 | 4.718 | | | 4.587 | 4.501 | | |
| Naphthoquinone | $^1B_1$ $(n \to \pi^\star)$ | 3.330 | 3.292 | 3.310 | | | 3.074 | 3.015 | 3.001 | 3.096 |
| | $^1A_2$ $(n \to \pi^\star)$ | 3.526 | 3.491 | 3.513 | | | 3.273 | 3.212 | 3.201 | 3.287 |
| | $^1A_1$ $(\pi \to \pi^\star)$ | 4.431 | 4.406 | 4.391 | | | 4.135 | 4.109 | 4.075 | 4.175 |
| | $^1B_2$ $(\pi \to \pi^\star)$ | 4.717 | 4.641 | 4.611 | | | 4.374 | 4.308 | 4.267 | 4.449 |
| | $^1A_2$ $(n \to \pi^\star)$ | 6.318 | 6.116 | 6.184 | | | 5.501 | 5.301 | 5.293 | 5.644 |
| | $^1A_1$ $(\pi \to \pi^\star)$ | 5.862 | 5.767 | 5.758 | | | 5.568 | 5.474 | 5.439 | 5.587 |
| | $^1B_2$ $(\pi \to \pi^\star)$ | 5.909 | 5.827 | 5.797 | | | 5.625 | 5.543 | 5.497 | 5.676 |
| | $^3B_1$ $(n \to \pi^\star)$ | 2.989 | 2.948 | 2.973 | | | 2.834 | 2.771 | | |
| | $^3A_2$ $(n \to \pi^\star)$ | 3.182 | 3.146 | 3.176 | | | 3.042 | 2.979 | | |
| | $^3B_2$ $(\pi \to \pi^\star)$ | 3.251 | 3.275 | 3.259 | | | 3.317 | 3.332 | | |
| | $^3B_2$ $(\pi \to \pi^\star)$ | 3.485 | 3.484 | 3.457 | | | 3.473 | 3.472 | | |
| | $^3A_1$ $(\pi \to \pi^\star)$ | 3.961 | 3.932 | 3.902 | | | 3.818 | 3.790 | | |
| Phenazine | $^1B_{1u}$ $(n \to \pi^\star)$ | 3.789 | 3.671 | 3.661 | | | 3.536 | 3.410 | 3.374 | |
| | $^1B_{3u}$ $(\pi \to \pi^\star)$ | 4.188 | 4.041 | 4.002 | | | 3.907 | 3.763 | 3.717 | |
| | $^1B_{2u}$ $(\pi \to \pi^\star)$ | 3.973 | 3.923 | 3.909 | | | 3.816 | 3.772 | 3.744 | |
| | $^1B_{1g}$ $(\pi \to \pi^\star)$ | 5.078 | 4.963 | 4.926 | | | 4.658 | 4.547 | 4.497 | |
| | $^1B_{2g}$ $(n \to \pi^\star)$ | 5.452 | 5.359 | 5.334 | | | 4.988 | 4.883 | 4.837 | |
| | $^1A_u$ $(\pi \to \pi^\star)$ | 5.606 | 5.490 | 5.517 | | | 5.264 | 5.138 | 5.115 | |
| | $^3B_{3u}$ $(\pi \to \pi^\star)$ | 2.381 | 2.364 | 2.352 | | | 2.448 | 2.420 | | |
| | $^3B_{1u}$ $(n \to \pi^\star)$ | 3.310 | 3.217 | 3.221 | | | 3.155 | 3.051 | | |
| | $^3B_{2u}$ $(\pi \to \pi^\star)$ | 3.570 | 3.461 | 3.416 | | | 3.518 | 3.421 | | |
| | $^3B_{1g}$ $(\pi \to \pi^\star)$ | 3.594 | 3.572 | 3.546 | | | 3.605 | 3.580 | | |
| Phthalimide | $^1B_1$ $(n \to \pi^\star)$ | 4.459 | 4.429 | 4.451 | | | 4.247 | 4.186 | 4.169 | 4.264 |
| | $^1A_1$ $(\pi \to \pi^\star)$ | 4.831 | 4.810 | 4.797 | | | 4.644 | 4.633 | 4.603 | 4.641 |
| | $^1A_2$ $(n \to \pi^\star)$ | 5.066 | 5.035 | 5.039 | | | 4.876 | 4.821 | 4.791 | 4.880 |
| | $^1B_2$ $(\pi \to \pi^\star)$ | 5.256 | 5.194 | 5.189 | | | 4.962 | 4.912 | 4.889 | 5.015 |
| | $^1B_2$ $(\pi \to \pi^\star)$ | 6.224 | 6.162 | 6.159 | | | 6.001 | 5.931 | 5.902 | 6.020 |
| | $^1A_2$ $(n \to \pi^\star)$ | 6.828 | 6.618 | 6.682 | | | 6.112 | 5.883 | 5.875 | 6.236 |
| | $^1A_1$ $(\pi \to \pi^\star)$ | 6.686 | 6.595 | 6.573 | | | 6.390 | 6.304 | 6.261 | 6.435 |
| | $^3B_2$ $(\pi \to \pi^\star)$ | 3.659 | 3.673 | 3.654 | | | 3.759 | 3.775 | 3.762 | |
| | $^3B_1$ $(n \to \pi^\star)$ | 4.165 | 4.135 | 4.163 | | | 4.024 | 3.964 | 3.957 | |
| | $^3A_1$ $(\pi \to \pi^\star)$ | 4.502 | 4.471 | 4.439 | | | 4.402 | 4.376 | 4.344 | |
| | $^3B_2$ $(\pi \to \pi^\star)$ | 4.649 | 4.598 | 4.581 | | | 4.570 | 4.523 | | |
| | $^3A_2$ $(n \to \pi^\star)$ | 4.758 | 4.727 | 4.737 | | | 4.655 | 4.598 | 4.578 | |
| | $^3B_2$ $(\pi \to \pi^\star)$ | 4.762 | 4.746 | 4.758 | | | 4.687 | 4.654 | | |
| Tolan | $^1B_{2u}$ $(\pi \to \pi^\star)$ | 4.941 | 4.892 | 4.886 | 4.801 | 4.795 | 4.776 | 4.730 | | |
| | $^1B_{3g}$ $(\pi \to \pi^\star)$ | 4.960 | 4.915 | 4.908 | 4.824 | 4.817 | 4.795 | 4.753 | | |
| | $^1B_{1u}$ $(\pi \to \pi^\star)$ | 5.096 | 4.969 | 4.931 | 4.865 | 4.837 | 4.950 | 4.824 | | |
| | $^1A_u$ $(\pi \to \pi^\star)$ | 5.944 | 5.820 | 5.752 | 5.667 | 5.606 | 5.733 | 5.607 | | |
| | $^1B_{3u}$ (Ryd) | 5.915 | 5.611 | 5.709 | 5.539 | 5.629 | 5.742 | 5.508 | | |
| | $^3B_{1u}$ $(\pi \to \pi^\star)$ | 3.223 | 3.206 | 3.197 | | | 3.294 | 3.270 | | |
| | $^3A_g$ $(\pi \to \pi^\star)$ | 3.932 | 3.938 | 3.918 | | | 4.076 | 4.081 | | |

# S3 Raw benchmark data

## S3.1 Wavefunction

Table S5: VTEs (in eV) computed with wave function methods using the aug-cc-pVTZ basis set.

| Compound | State | CIS(D) | CC2 | EOM-MP2 | CCSD | CCSD(T)(a)* | CCSDR(3) | CCSDT-3 | SOS-ADC(2) [TM] | SOS-CC2 | SCS-CC2 | SOS-ADC(2) [QC] | ADC(2) | ADC(3) | ADC(2.5) |
|---|---|---|---|---|---|---|---|---|---|---|---|---|---|---|---|
| Anthracene | $^1B_{1u}$ ($\pi \rightarrow \pi^\star$) | 3.944 | 3.659 | 4.419 | 3.979 | | 3.839 | 3.826 | 3.883 | 3.914 | 3.832 | 3.677 | 3.651 | 3.638 | 3.645 |
| | $^1B_{2u}$ ($\pi \rightarrow \pi^\star$) | 3.946 | 3.904 | 4.313 | 3.931 | | 3.895 | 3.823 | 3.841 | 3.829 | 3.861 | 3.611 | 3.911 | 3.640 | 3.776 |
| | $^1B_{3g}$ ($\pi \rightarrow \pi^\star$) | 5.537 | 5.113 | 5.970 | 5.602 | | 5.296 | 5.193 | 5.490 | 5.488 | 5.350 | 5.255 | 5.146 | 5.009 | 5.078 |
| | $^1B_{2g}$ (Ryd) | 5.092 | 4.969 | 5.467 | 5.123 | | 5.107 | 5.087 | 5.255 | 5.200 | 5.123 | 5.136 | 5.030 | 4.897 | 4.964 |
| | $^1B_{1u}$ ($\pi \rightarrow \pi^\star$) | 5.562 | 5.247 | 6.098 | 5.504 | | 5.407 | 5.368 | 5.534 | 5.514 | 5.426 | 5.357 | 5.284 | 5.236 | 5.260 |
| | $^1B_{3g}$ ($\pi \rightarrow \pi^\star$) | 5.471 | 5.247 | 5.777 | 5.485 | | 5.342 | | 5.384 | 5.403 | 5.365 | 5.186 | 5.237 | 5.206 | 5.222 |
| | $^1A_{g}$ ($\pi \rightarrow \pi^\star$) | 5.646 | 5.607 | 6.080 | 5.704 | | 5.554 | 5.442 | 5.608 | 5.598 | 5.599 | 5.378 | 5.620 | | |
| | $^1B_{3u}$ (Ryd) | 5.362 | 5.248 | 5.773 | 5.423 | | 5.408 | | 5.557 | 5.503 | 5.417 | 5.451 | 5.321 | 5.195 | 5.258 |
| | $^1A_{u}$ (Ryd) | 5.444 | 5.319 | 5.841 | 5.511 | | 5.483 | 5.463 | 5.625 | 5.570 | 5.487 | 5.509 | 5.386 | 5.274 | 5.330 |
| | $^1B_{2u}$ ($\pi \rightarrow \pi^\star$) | 5.470 | 5.372 | 5.849 | 5.702 | | 5.533 | | 5.569 | 5.583 | 5.513 | 5.359 | 5.352 | 5.409 | 5.381 |
| | $^3B_{1u}$ ($\pi \rightarrow \pi^\star$) | 2.646 | 2.390 | 2.710 | 2.217 | | | | 2.506 | 2.509 | 2.470 | 2.343 | 2.405 | 2.024 | 2.215 |
| | $^3B_{3g}$ ($\pi \rightarrow \pi^\star$) | 3.955 | 3.792 | 3.952 | 3.620 | | | | 3.796 | 3.803 | 3.800 | 3.650 | 3.780 | 3.405 | 3.593 |
| | $^3B_{2u}$ ($\pi \rightarrow \pi^\star$) | 4.008 | 3.861 | 4.245 | 3.808 | | | | 3.863 | 3.875 | 3.872 | 3.673 | 3.847 | 3.432 | 3.640 |
| Anthraquinone | $^1B_{1g}$ ($n \rightarrow \pi^\star$) | 3.280 | 3.164 | 3.681 | 3.485 | | 3.343 | | 3.454 | 3.594 | 3.460 | 3.203 | 3.025 | 3.419 | 3.222 |
| | $^1A_{u}$ ($n \rightarrow \pi^\star$) | 3.492 | 3.426 | 3.858 | 3.701 | | 3.574 | | 3.623 | 3.793 | 3.678 | 3.372 | 3.236 | 3.672 | 3.454 |
| | $^1A_{g}$ ($\pi \rightarrow \pi^\star$) | 4.322 | 4.238 | 4.856 | 4.472 | | 4.328 | | 4.316 | 4.325 | 4.310 | 4.075 | 4.229 | 4.196 | 4.213 |
| | $^1B_{2u}$ ($\pi \rightarrow \pi^\star$) | 4.371 | 4.287 | 4.860 | 4.462 | | 4.336 | | 4.335 | 4.329 | 4.328 | 4.100 | 4.308 | 4.172 | 4.240 |
| | $^1B_{3g}$ ($\pi \rightarrow \pi^\star$) | 4.739 | 4.348 | 5.068 | 4.627 | | 4.455 | | 4.629 | 4.608 | 4.526 | 4.407 | 4.400 | 4.209 | 4.305 |
| | $^1B_{1u}$ ($\pi \rightarrow \pi^\star$) | 5.482 | 5.426 | 5.645 | 5.344 | | 5.196 | | 5.188 | 5.269 | 5.216 | 4.964 | 4.994 | 5.029 | 5.012 |
| | $^1B_{2u}$ ($\pi \rightarrow \pi^\star$) | 5.523 | 5.078 | 6.109 | 5.734 | | 5.510 | | 5.691 | 5.671 | 5.585 | 5.466 | 5.452 | 5.385 | 5.419 |
| | $^3B_{1g}$ ($n \rightarrow \pi^\star$) | 3.060 | 2.897 | 3.369 | 3.165 | | | | 3.240 | 3.364 | 3.215 | 3.005 | 2.767 | 3.135 | 2.951 |
| | $^3A_{u}$ ($n \rightarrow \pi^\star$) | 3.272 | 3.159 | 3.553 | 3.384 | | | | 3.418 | 3.571 | 3.438 | 3.185 | 2.983 | 3.398 | 3.191 |
| | $^3B_{1u}$ ($\pi \rightarrow \pi^\star$) | 3.834 | 3.618 | 3.805 | 3.347 | | | | 3.654 | 3.678 | 3.661 | 3.492 | 3.578 | 3.196 | 3.387 |
| | $^3B_{3g}$ ($\pi \rightarrow \pi^\star$) | 3.965 | 3.666 | 3.936 | 3.466 | | | | 3.774 | 3.769 | 3.739 | 3.613 | 3.679 | 3.236 | 3.458 |
| | $^3A_{g}$ ($\pi \rightarrow \pi^\star$) | 4.024 | 3.832 | 4.198 | 3.840 | | | | 3.959 | 4.009 | 3.956 | 3.765 | 3.788 | 3.556 | 3.672 |
| Aza-BODIPY | $^1B_{2}$ ($\pi \rightarrow \pi^\star$) | 2.741 | 2.679 | 3.144 | 2.634 | 2.592 | 2.586 | 2.552 | 2.539 | 2.643 | 2.659 | 2.304 | 2.549 | 2.099 | 2.324 |
| | $^1B_{2}$ ($\pi \rightarrow \pi^\star$) | 3.455 | 3.559 | 4.274 | 3.823 | 3.618 | 3.605 | 3.524 | 3.703 | 3.759 | 3.691 | 3.457 | 3.493 | 3.259 | 3.376 |
| | $^1A_{1}$ ($\pi \rightarrow \pi^\star$) | 3.607 | 3.620 | 4.362 | 3.942 | 3.700 | 3.685 | 3.571 | 3.785 | 3.841 | 3.770 | 3.530 | 3.556 | 3.072 | 3.314 |
| | $^1B_{1}$ ($n \rightarrow \pi^\star$) | 4.159 | 3.825 | 4.493 | 4.078 | 3.985 | 3.983 | 3.945 | 4.244 | 4.216 | 4.088 | 4.004 | 3.844 | 3.892 | 3.868 |
| | $^3B_{2}$ ($\pi \rightarrow \pi^\star$) | 1.627 | 1.519 | 1.817 | 1.198 | | | | 1.508 | 1.521 | 1.520 | 1.327 | 1.486 | 0.867 | 1.177 |
| | $^3B_{2}$ ($\pi \rightarrow \pi^\star$) | 3.130 | 2.886 | 3.341 | 2.887 | | | | 3.069 | 3.116 | 3.041 | 2.856 | 2.829 | 2.527 | 2.678 |
| | $^3A_{1}$ ($\pi \rightarrow \pi^\star$) | 3.441 | 3.156 | 3.599 | 3.158 | | | | 3.314 | 3.357 | 3.293 | 3.104 | 3.098 | 2.774 | 2.936 |
| | $^3B_{1}$ ($n \rightarrow \pi^\star$) | 3.712 | 3.386 | 3.868 | 3.496 | | | | 3.769 | 3.775 | 3.647 | 3.556 | 3.369 | 3.326 | 3.348 |
| Azobenzene | $^1B_{g}$ ($n \rightarrow \pi^\star$) | 3.083 | 2.853 | 3.217 | 2.987 | 2.921 | 2.922 | 2.907 | 3.136 | 3.119 | 3.034 | 2.921 | 2.863 | 2.720 | 2.792 |
| | $^1B_{u}$ ($\pi \rightarrow \pi^\star$) | 4.478 | 4.145 | 4.786 | 4.460 | 4.320 | 4.315 | 4.300 | 4.366 | 4.374 | 4.306 | 4.145 | 4.141 | 4.109 | 4.125 |
| | $^1A_{g}$ ($\pi \rightarrow \pi^\star$) | 4.677 | 4.515 | 5.037 | 4.722 | 4.576 | 4.572 | 4.527 | 4.572 | 4.564 | 4.564 | 4.339 | 4.535 | 4.402 | 4.469 |
| | $^1B_{u}$ ($\pi \rightarrow \pi^\star$) | 4.684 | 4.507 | 5.050 | 4.734 | 4.578 | 4.576 | 4.536 | 4.602 | 4.599 | 4.577 | 4.371 | 4.527 | 4.405 | 4.466 |
| | $^1A_{g}$ ($\pi \rightarrow \pi^\star$) | 5.993 | 5.227 | 5.957 | 5.639 | 5.427 | 5.400 | 5.336 | 5.523 | 5.518 | 5.427 | 5.295 | 5.254 | 4.731 | 4.993 |
| | $^3B_{g}$ ($n \rightarrow \pi^\star$) | 2.465 | 2.265 | 2.517 | 2.317 | | | | 2.564 | 2.565 | 2.465 | 2.379 | 2.248 | 2.063 | 2.156 |
| | $^3B_{u}$ ($\pi \rightarrow \pi^\star$) | 3.306 | 2.953 | 3.240 | 2.771 | | | | 3.097 | 3.097 | 3.052 | 2.930 | 2.964 | 2.497 | 2.731 |
| | $^3A_{g}$ ($\pi \rightarrow \pi^\star$) | 4.316 | 4.077 | 4.226 | 3.833 | | | | 4.103 | 4.100 | 4.097 | 3.958 | 4.077 | 3.664 | 3.871 |
| | $^3B_{u}$ ($\pi \rightarrow \pi^\star$) | 4.615 | 4.302 | 4.658 | 4.359 | | | | 4.451 | 4.455 | 4.416 | 4.268 | 4.311 | 4.013 | 4.162 |
| | $^3A_{g}$ ($\pi \rightarrow \pi^\star$) | 4.595 | 4.377 | 4.746 | 4.444 | | | | 4.518 | 4.523 | 4.483 | 4.330 | 4.382 | 4.064 | 4.223 |
| BODIPY | $^1B_{2}$ ($\pi \rightarrow \pi^\star$) | 2.935 | 2.915 | 3.321 | 2.908 | 2.848 | 2.842 | 2.817 | 2.782 | 2.862 | 2.882 | 2.556 | 2.798 | 2.518 | 2.658 |
| | $^1B_{2}$ ($\pi \rightarrow \pi^\star$) | 3.860 | 3.883 | 4.524 | 4.175 | 3.948 | 3.931 | 3.884 | 4.047 | 4.220 | 4.035 | 3.809 | 3.810 | 3.776 | 3.793 |
| | $^1A_{1}$ ($\pi \rightarrow \pi^\star$) | 4.037 | 4.015 | 4.663 | 4.336 | 4.088 | 4.075 | 4.005 | 4.171 | 4.237 | 4.167 | 3.926 | 3.935 | 3.803 | 3.869 |
| | $^3B_{2}$ ($\pi \rightarrow \pi^\star$) | 2.134 | 2.031 | 2.278 | 1.794 | | | | 2.058 | 2.076 | 2.061 | 1.881 | 1.992 | 1.493 | 1.743 |
| | $^3B_{2}$ ($\pi \rightarrow \pi^\star$) | 3.471 | 3.211 | 3.597 | 3.214 | | | | 3.365 | 3.415 | 3.349 | 3.161 | 3.144 | 2.947 | 3.046 |
| | $^3A_{1}$ ($\pi \rightarrow \pi^\star$) | 3.870 | 3.445 | 3.810 | 3.433 | | | | 3.568 | 3.617 | 3.563 | 3.369 | 3.377 | 3.178 | 3.278 |
| Coumarin | $^1A'$ ($\pi \rightarrow \pi^\star$) | 4.783 | 4.333 | 4.818 | 4.530 | 4.402 | 4.401 | 4.373 | 4.391 | 4.410 | 4.406 | 4.155 | 4.274 | 4.291 | 4.283 |
| | $^1A''$ ($n \rightarrow \pi^\star$) | 4.991 | 4.741 | 5.221 | 5.133 | 4.955 | 4.947 | 4.906 | 5.014 | 5.211 | 5.071 | 4.754 | 4.542 | 5.144 | 4.843 |
| | $^1A'$ ($\pi \rightarrow \pi^\star$) | 4.932 | 5.040 | 5.418 | 5.173 | 5.067 | 5.063 | 5.035 | 5.043 | 5.091 | 5.075 | 4.833 | 4.997 | 4.862 | 4.930 |
| | $^3A'$ ($\pi \rightarrow \pi^\star$) | 3.594 | 3.396 | 3.526 | 3.199 | | | | 3.440 | 3.468 | 3.446 | 3.284 | 3.348 | 3.004 | 3.176 |
| | $^3A'$ ($\pi \rightarrow \pi^\star$) | 4.573 | 4.190 | 4.443 | 4.127 | | | | 4.310 | 4.327 | 4.289 | 4.138 | 4.174 | 3.941 | 4.058 |
| | $^3A''$ ($n \rightarrow \pi^\star$) | 4.800 | 4.539 | 4.961 | 4.856 | | | | 4.843 | 5.024 | 4.874 | 4.600 | 4.347 | 4.891 | 4.619 |
| Cyclazine | $^1A_2'$ ($\pi \rightarrow \pi^\star$) | 1.042 | 1.051 | 1.581 | 1.090 | 1.059 | 1.071 | | 1.121 | 1.137 | 1.110 | 0.893 | 1.001 | | |
| | $^1E'$ ($\pi \rightarrow \pi^\star$) | 3.108 | 3.037 | 3.590 | 3.225 | 3.131 | 3.155 | | 3.162 | 3.224 | 3.162 | 2.945 | 2.928 | | |
| | $^1A_1''$ (Ryd) | 3.282 | 3.147 | 3.598 | 3.203 | 3.201 | 3.211 | | 3.457 | 3.381 | 3.303 | 3.331 | 3.203 | | |
| | $^1E''$ (Ryd) | 3.766 | 3.652 | 4.113 | 3.717 | 3.721 | 3.731 | | 3.960 | 3.882 | 3.803 | 3.840 | 3.710 | | |
| | $^3A_2'$ ($\pi \rightarrow \pi^\star$) | 1.319 | 1.181 | 1.628 | 1.154 | | | | 1.394 | 1.407 | 1.330 | 1.188 | 1.138 | | |
| | $^3E'$ ($\pi \rightarrow \pi^\star$) | 2.382 | 2.236 | 2.635 | 2.195 | | | | 2.399 | 2.402 | 2.347 | 2.210 | 2.198 | | |
| | $^3A_1''$ (Ryd) | 3.275 | 3.138 | 3.573 | 3.1[illegible] | | | | 3.456 | 3.381 | 3.300 | 3.334 | 3.192 | | |
| | $^3E''$ (Ryd) | 3.761 | 3.643 | 4.050 | 3.700 | | | | 3.957 | 3.878 | 3.799 | 3.838 | 3.701 | | |

Table S6: VTEs (in eV) computed with wave function methods using the aug-cc-pVTZ basis set.

| Compound | State | CIS(D) | CC2 | EOM-MP2 | CCSD | CCSD(T)(a)$^\star$ | CCSDR(3) | CCSDT-3 | SOS-ADC(2) [TM] | SOS-CC2 | SCS-CC2 | SOS-ADC(2) [QC] | ADC(2) | ADC(3) | ADC(2.5) |
|---|---|---|---|---|---|---|---|---|---|---|---|---|---|---|---|
| Heptazine | $^1A_2'$ $(\pi \rightarrow \pi^\star)$ | 2.659 | 2.767 | 3.376 | 2.953 | 2.820 | 2.834 | 2.799 | 2.893 | 2.933 | 2.993 | 2.628 | 2.675 | 2.820 | 2.748 |
| | $^1A_1''$ $(n \rightarrow \pi^\star)$ | 3.967 | 3.818 | 4.508 | 4.333 | 4.118 | 4.110 | 4.118 | 4.238 | 4.314 | 4.164 | 3.965 | 3.740 | 4.524 | 4.132 |
| | $^1E''$ $(n \rightarrow \pi^\star)$ | 3.983 | 3.958 | 4.574 | 4.394 | 4.214 | 4.207 | 4.215 | 4.310 | 4.398 | 4.268 | 4.045 | 3.856 | 4.518 | 4.187 |
| | $^1E'$ $(\pi \rightarrow \pi^\star)$ | 4.366 | 4.476 | 5.143 | 4.789 | 4.610 | 4.595 | 4.578 | 4.655 | 4.751 | 4.665 | 4.390 | 4.326 | 4.615 | 4.471 |
| | $^3A_2'$ $(\pi \rightarrow \pi^\star)$ | 3.178 | 3.006 | 3.491 | 3.087 | | | | 3.345 | 3.382 | 3.256 | 3.109 | 2.921 | | |
| | $^3E''(\pi \rightarrow \pi^\star)$ | 3.932 | 3.747 | 4.217 | 3.781 | | | | 4.022 | 4.042 | 3.945 | 3.797 | 3.683 | | |
| | $^3A_1''$ $(n \rightarrow \pi^\star)$ | 4.139 | 3.814 | 4.473 | 4.295 | | | | 4.285 | 4.356 | 4.188 | 4.024 | 3.740 | | |
| | $^3E''$ $(n \rightarrow \pi^\star)$ | 4.094 | 3.927 | 4.530 | 4.344 | | | | 4.343 | 4.423 | 4.271 | 4.089 | 3.834 | | |
| Naphthalimide | $^1B_2$ $(\pi \rightarrow \pi^\star)$ | 4.206 | 4.162 | 4.663 | 4.220 | 4.148 | 4.151 | 4.089 | 4.113 | 4.115 | 4.134 | 3.880 | 4.160 | 3.932 | 4.046 |
| | $^1B_1$ $(n \rightarrow \pi^\star)$ | 4.290 | 4.044 | 4.706 | 4.568 | 4.369 | 4.348 | 4.295 | 4.422 | 4.606 | 4.434 | 4.152 | 3.863 | 4.633 | 4.248 |
| | $^1A_1$ $(\pi \rightarrow \pi^\star)$ | 4.432 | 4.127 | 4.749 | 4.406 | 4.267 | 4.257 | 4.237 | 4.291 | 4.350 | 4.281 | 4.071 | 4.078 | 4.003 | 4.041 |
| | $^1A_2$ $(n \rightarrow \pi^\star)$ | 4.810 | 4.581 | 5.091 | 4.997 | 4.812 | 4.794 | 4.751 | 4.827 | 5.017 | 4.883 | 4.567 | 4.378 | 4.998 | 4.688 |
| | $^3A_1$ $(\pi \rightarrow \pi^\star)$ | 3.194 | 2.920 | 3.215 | 2.735 | | | | 3.016 | 3.027 | 2.993 | 2.846 | 2.907 | 2.517 | 2.712 |
| | $^3B_2$ $(\pi \rightarrow \pi^\star)$ | 4.187 | 3.924 | 4.244 | 3.846 | | | | 3.963 | 3.983 | 3.967 | 3.779 | 3.897 | 3.529 | 3.713 |
| | $^3B_1$ $(n \rightarrow \pi^\star)$ | 4.197 | 3.894 | 4.496 | 4.342 | | | | 4.301 | 4.469 | 4.289 | 4.045 | 3.723 | 4.426 | 4.075 |
| | $^3B_2$ $(\pi \rightarrow \pi^\star)$ | 4.314 | 4.275 | 4.499 | 4.132 | | | | 4.276 | 4.295 | 4.290 | 4.111 | 4.240 | 3.875 | 4.058 |
| | $^3A_2$ $(n \rightarrow \pi^\star)$ | 4.567 | 4.395 | 4.856 | 4.718 | | | | 4.683 | 4.857 | 4.711 | 4.439 | 4.203 | 4.775 | 4.489 |
| Naphthoquinone | $^1B_1$ $(n \rightarrow \pi^\star)$ | 3.154 | 2.990 | 3.459 | 3.310 | 3.157 | 3.144 | 3.097 | 3.330 | 3.453 | 3.308 | 3.082 | 2.872 | 3.169 | 3.021 |
| | $^1A_2$ $(n \rightarrow \pi^\star)$ | 3.352 | 3.204 | 3.632 | 3.513 | 3.363 | 3.349 | 3.298 | 3.479 | 3.633 | 3.499 | 3.228 | 3.043 | 3.411 | 3.227 |
| | $^1A_1$ $(\pi \rightarrow \pi^\star)$ | 4.238 | 4.140 | 4.760 | 4.391 | 4.237 | 4.228 | 4.175 | 4.284 | 4.284 | 4.254 | 4.045 | 4.154 | 4.064 | 4.109 |
| | $^1B_2$ $(\pi \rightarrow \pi^\star)$ | 4.697 | 4.316 | 4.969 | 4.611 | 4.417 | 4.411 | 4.369 | 4.667 | 4.648 | 4.543 | 4.445 | 4.369 | 4.151 | 4.260 |
| | $^1A_2$ $(n \rightarrow \pi^\star)$ | 5.984 | 5.155 | 6.349 | 6.184 | 5.658 | 5.636 | 5.590 | 6.066 | 6.118 | 5.791 | 5.769 | 5.124 | 5.905 | 5.515 |
| | $^1A_1$ $(\pi \rightarrow \pi^\star)$ | 5.572 | 5.533 | 6.047 | 5.758 | 5.544 | 5.543 | 5.531 | 5.698 | 5.705 | 5.635 | 5.469 | 5.535 | 5.385 | 5.460 |
| | $^1B_2$ $(\pi \rightarrow \pi^\star)$ | 5.794 | 5.522 | 5.964 | 5.797 | 5.605 | 5.582 | 5.585 | 5.736 | 5.832 | 5.736 | 5.515 | 5.419 | 5.394 | 5.407 |
| | $^3B_1$ $(n \rightarrow \pi^\star)$ | 2.903 | 2.700 | 3.128 | 2.973 | | | | 3.092 | 3.202 | 3.041 | 2.862 | 2.591 | 2.885 | 2.738 |
| | $^3A_2$ $(n \rightarrow \pi^\star)$ | 3.102 | 2.922 | 3.307 | 3.176 | | | | 3.253 | 3.391 | 3.241 | 3.021 | 2.773 | 3.135 | 2.954 |
| | $^3B_2$ $(\pi \rightarrow \pi^\star)$ | 3.644 | 3.478 | 3.589 | 3.259 | | | | 3.539 | 3.563 | 3.538 | 3.384 | 3.440 | 3.053 | 3.247 |
| | $^3B_2$ $(\pi \rightarrow \pi^\star)$ | 3.883 | 3.588 | 3.836 | 3.457 | | | | 3.748 | 3.741 | 3.696 | 3.594 | 3.607 | 3.171 | 3.389 |
| | $^3A_1$ $(\pi \rightarrow \pi^\star)$ | 4.109 | 3.850 | 4.242 | 3.902 | | | | 4.043 | 4.078 | 4.012 | 3.848 | 3.833 | 3.571 | 3.702 |
| Phenazine | $^1B_{1u}$ $(n \rightarrow \pi^\star)$ | 3.591 | 3.247 | 4.114 | 3.661 | 3.514 | 3.515 | 3.473 | 3.787 | 3.748 | 3.586 | 3.537 | 3.294 | 3.466 | 3.380 |
| | $^1B_{3u}$ $(\pi \rightarrow \pi^\star)$ | 3.994 | 3.656 | 4.422 | 4.002 | 3.839 | 3.834 | 3.810 | 3.900 | 3.929 | 3.841 | 3.672 | 3.656 | 3.604 | 3.630 |
| | $^1B_{2u}$ $(\pi \rightarrow \pi^\star)$ | 3.946 | 3.869 | 4.487 | 3.909 | 3.863 | 3.868 | 3.791 | 3.812 | 3.802 | 3.825 | 3.569 | 3.888 | 3.543 | 3.716 |
| | $^1B_{1g}$ $(\pi \rightarrow \pi^\star)$ | 4.880 | 4.540 | 5.355 | 4.926 | 4.705 | 4.696 | 4.639 | 4.797 | 4.795 | 4.711 | 4.559 | 4.571 | 4.407 | 4.489 |
| | $^1B_{2g}$ $(n \rightarrow \pi^\star)$ | 5.458 | 4.917 | 5.725 | 5.334 | 5.128 | 5.112 | 5.006 | 5.395 | 5.376 | 5.230 | 5.139 | 4.947 | 4.826 | 4.887 |
| | $^1A_u$ $(\pi \rightarrow \pi^\star)$ | 5.019 | 4.943 | 5.914 | 5.517 | 5.270 | 5.274 | 5.271 | 5.479 | 5.449 | 5.281 | 5.209 | 4.960 | 5.537 | 5.249 |
| | $^3B_{3u}$ $(\pi \rightarrow \pi^\star)$ | 2.845 | 2.540 | 2.913 | 2.352 | | | | 2.648 | 2.653 | 2.617 | 2.470 | 2.551 | 2.115 | 2.333 |
| | $^3B_{1u}$ $(n \rightarrow \pi^\star)$ | 3.309 | 2.930 | 3.649 | 3.221 | | | | 3.450 | 3.420 | 3.260 | 3.222 | 2.966 | 3.044 | 3.005 |
| | $^3B_{2u}$ $(\pi \rightarrow \pi^\star)$ | 3.686 | 3.530 | 3.973 | 3.416 | | | | 3.536 | 3.538 | 3.536 | 3.338 | 3.534 | 3.014 | 3.274 |
| | $^3B_{1g}$ $(\pi \rightarrow \pi^\star)$ | 3.887 | 3.678 | 3.909 | 3.546 | | | | 3.718 | 3.724 | 3.711 | 3.559 | 3.673 | 3.299 | 3.486 |
| Phthalimide | $^1B_1$ $(n \rightarrow \pi^\star)$ | 4.231 | 4.094 | 4.603 | 4.451 | 4.301 | 4.289 | 4.263 | 4.377 | 4.537 | 4.397 | 4.119 | 3.930 | 4.475 | 4.203 |
| | $^1A_1$ $(\pi \rightarrow \pi^\star)$ | 4.804 | 4.741 | 5.142 | 4.797 | 4.703 | 4.705 | 4.658 | 4.644 | 4.637 | 4.677 | 4.411 | 4.749 | 4.553 | 4.651 |
| | $^1A_2$ $(n \rightarrow \pi^\star)$ | 4.853 | 4.791 | 5.158 | 5.039 | 4.913 | 4.904 | 4.873 | 4.942 | 5.122 | 4.792 | 4.693 | 4.589 | 5.025 | 4.807 |
| | $^1B_2$ $(\pi \rightarrow \pi^\star)$ | 5.532 | 4.946 | 5.530 | 5.189 | 5.015 | 5.013 | 4.982 | 5.181 | 5.172 | 5.103 | 4.953 | 4.959 | 4.864 | 4.912 |
| | $^1B_2$ $(\pi \rightarrow \pi^\star)$ | 5.907 | 5.896 | 6.345 | 6.159 | 6.005 | 5.988 | 5.983 | 5.958 | 6.089 | 6.030 | 5.716 | 5.743 | 5.991 | 5.867 |
| | $^1A_2$ $(n \rightarrow \pi^\star)$ | 6.956 | 5.678 | 6.843 | 6.682 | 6.190 | 6.178 | 6.142 | 6.510 | 6.599 | 6.290 | 6.206 | 5.606 | 6.797 | 6.202 |
| | $^1A_1$ $(\pi \rightarrow \pi^\star)$ | 6.833 | 6.312 | 6.848 | 6.573 | 6.371 | 6.346 | 6.359 | 6.506 | 6.518 | 6.449 | 6.292 | 6.304 | 6.236 | 6.270 |
| | $^3B_2$ $(\pi \rightarrow \pi^\star)$ | 4.053 | 3.955 | 4.086 | 3.654 | | | | 3.974 | 3.974 | 3.971 | 3.830 | 3.952 | 3.501 | 3.727 |
| | $^3B_1$ $(n \rightarrow \pi^\star)$ | 4.152 | 3.860 | 4.329 | 4.163 | | | | 4.196 | 4.342 | 4.187 | 3.955 | 3.710 | 4.199 | 3.955 |
| | $^3A_1$ $(\pi \rightarrow \pi^\star)$ | 4.629 | 4.518 | 4.760 | 4.439 | | | | 4.544 | 4.565 | 4.555 | 4.362 | 4.497 | 4.115 | 4.306 |
| | $^3B_2$ $(\pi \rightarrow \pi^\star)$ | 4.761 | 4.656 | 4.891 | 4.581 | | | | 4.683 | 4.693 | 4.695 | 4.511 | 4.594 | 4.272 | 4.433 |
| | $^3A_2$ $(n \rightarrow \pi^\star)$ | 4.642 | 4.536 | 4.870 | 4.737 | | | | 4.750 | 4.914 | 4.792 | 4.518 | 4.347 | 4.748 | 4.548 |
| | $^3B_2$ $(\pi \rightarrow \pi^\star)$ | 5.077 | 4.781 | 5.055 | 4.758 | | | | 4.942 | 5.017 | 4.929 | 4.730 | 4.735 | 4.603 | 4.669 |
| Tolan | $^1B_{2u}$ $(\pi \rightarrow \pi^\star)$ | 4.926 | 4.862 | 5.197 | 4.886 | 4.792 | 4.795 | | 4.739 | 4.731 | 4.780 | 4.517 | 4.871 | 4.622 | 4.747 |
| | $^1B_{3g}$ $(\pi \rightarrow \pi^\star)$ | 4.941 | 4.886 | 5.218 | 4.908 | 4.814 | 4.817 | | 4.756 | 4.747 | 4.799 | 4.531 | 4.894 | 4.645 | 4.770 |
| | $^1B_{1u}$ $(\pi \rightarrow \pi^\star)$ | 5.019 | 4.767 | 5.231 | 4.931 | 4.838 | 4.837 | | 4.884 | 4.916 | 4.870 | 4.692 | 4.736 | 4.586 | 4.661 |
| | $^1A_u$ $(\pi \rightarrow \pi^\star)$ | 6.000 | 5.643 | 6.012 | 5.752 | 5.606 | 5.606 | | 5.944 | 5.959 | 5.857 | 5.759 | 5.644 | 5.350 | 5.497 |
| | $^1B_{3u}$ (Ryd) | 5.702 | 5.581 | 6.023 | 5.709 | 5.621 | 5.629 | | 5.878 | 5.814 | 5.737 | 5.759 | 5.648 | 5.425 | 5.537 |
| | $^3B_{1u}$ $(\pi \rightarrow \pi^\star)$ | 3.687 | 3.461 | 3.645 | 3.197 | | | | 3.515 | 3.523 | 3.505 | 3.367 | 3.456 | 2.991 | 3.224 |
| | $^3A_g$ $(\pi \rightarrow \pi^\star)$ | 4.393 | 4.253 | 4.315 | 3.918 | | | | 4.203 | 4.201 | 4.219 | 4.074 | 4.247 | 3.810 | 4.029 |

## S3.2 TD-DFT

Table S7: VTEs (in eV) computed with TD-DFT using the aug-cc-pVTZ basis set.

| Compound | State | TPSSh | $\tau$-HCTHHyb | B3LYP | PBE0 | cSCAN0 | M06 | cM06 | SOGGA11-X | BMK | MN15 | M08-HX | M06-2X | cM06-2X |
|---|---|---|---|---|---|---|---|---|---|---|---|---|---|---|
| Anthracene | $^1B_{1u}$ $(\pi \to \pi^\star)$ | 3.136 | 3.138 | 3.197 | 3.279 | 3.285 | 3.193 | 3.208 | 3.454 | 3.485 | 3.392 | 3.540 | 3.545 | 3.567 |
| | $^1B_{2u}$ $(\pi \to \pi^\star)$ | 3.846 | 3.845 | 3.878 | 3.955 | 4.049 | 3.830 | 3.833 | 4.098 | 4.100 | 3.980 | 4.106 | 4.095 | 4.097 |
| | $^1B_{3g}$ $(\pi \to \pi^\star)$ | 4.789 | 4.770 | 4.816 | 4.925 | 4.960 | 4.759 | 4.787 | 5.107 | 5.147 | 5.014 | 5.129 | 5.160 | 5.198 |
| | $^1B_{2g}$ (Ryd) | 4.737 | 4.889 | 4.682 | 4.934 | 5.276 | 3.958 | 4.012 | 4.867 | 5.238 | 5.590 | 4.479 | 4.967 | 5.016 |
| | $^1B_{1u}$ $(\pi \to \pi^\star)$ | 4.945 | 4.967 | 4.961 | 5.142 | 5.328 | 4.627 | 4.714 | 5.313 | 5.501 | 5.417 | 5.014 | 5.349 | 5.398 |
| | $^1B_{3g}$ $(\pi \to \pi^\star)$ | 4.336 | 4.387 | 4.507 | 4.686 | 4.842 | 4.603 | 4.615 | 5.142 | 5.164 | 5.046 | 5.268 | 5.318 | 5.330 |
| | $^1A_g$ $(\pi \to \pi^\star)$ | 5.479 | 5.478 | 5.528 | 5.649 | 5.802 | 5.474 | 5.478 | 5.891 | 5.897 | 5.741 | 5.909 | 5.906 | 5.910 |
| | $^1B_{3u}$ (Ryd) | 4.964 | 5.126 | 4.918 | 5.168 | 5.538 | 4.143 | 4.179 | 5.083 | 5.454 | 5.885 | 4.709 | 5.212 | 5.240 |
| | $^1A_u$ (Ryd) | 4.926 | 5.099 | 4.895 | 5.168 | 5.549 | 4.171 | 4.211 | 5.121 | 5.478 | 5.897 | 4.789 | 5.287 | 5.322 |
| | $^1B_{2u}$ $(\pi \to \pi^\star)$ | 5.158 | 5.131 | 5.162 | 5.247 | 5.314 | 5.098 | 5.148 | 5.398 | 5.397 | 5.258 | 5.355 | 5.367 | 5.438 |
| | $^3B_{1u}$ $(\pi \to \pi^\star)$ | 1.773 | 1.857 | 1.847 | 1.701 | | 1.756 | 1.765 | 1.851 | 2.011 | 1.886 | 2.180 | 2.186 | 2.204 |
| | $^3B_{3g}$ $(\pi \to \pi^\star)$ | 3.245 | 3.319 | 3.313 | 3.214 | | 3.219 | 3.240 | 3.415 | 3.550 | 3.392 | 3.668 | 3.678 | 3.714 |
| | $^3B_{2u}$ $(\pi \to \pi^\star)$ | 3.465 | 3.477 | 3.503 | 3.518 | | 3.456 | 3.488 | 3.699 | 3.744 | 3.593 | 3.772 | 3.768 | 3.817 |
| Anthraquinone | $^1B_{1g}$ $(n \to \pi^\star)$ | 2.763 | 2.810 | 2.938 | 3.003 | 3.096 | 3.032 | 3.042 | 3.357 | 3.181 | 2.997 | 3.223 | 3.182 | 3.393 |
| | $^1A_u$ $(n \to \pi^\star)$ | 3.075 | 3.117 | 3.233 | 3.306 | 3.385 | 3.324 | 3.331 | 3.635 | 3.469 | 3.264 | 3.489 | 3.451 | 3.681 |
| | $^1A_g$ $(\pi \to \pi^\star)$ | 3.725 | 3.767 | 3.862 | 4.006 | | 3.959 | 3.964 | 4.329 | 4.338 | 4.236 | 4.478 | 4.469 | 4.477 |
| | $^1B_{2u}$ $(\pi \to \pi^\star)$ | 3.737 | 3.772 | 3.867 | 4.011 | 4.117 | 3.945 | 3.950 | 4.333 | 4.342 | 4.246 | 4.481 | 4.472 | 4.479 |
| | $^1B_{3g}$ $(\pi \to \pi^\star)$ | 3.602 | 3.619 | 3.704 | 3.838 | 3.904 | 3.768 | 3.784 | 4.131 | 4.145 | 4.041 | 4.295 | 4.281 | 4.307 |
| | $^1B_{1u}$ $(\pi \to \pi^\star)$ | 4.384 | 4.429 | 4.526 | 4.665 | 4.758 | 4.605 | 4.618 | 4.954 | 4.976 | 4.874 | 5.075 | 5.073 | 5.096 |
| | $^1B_{2u}$ $(\pi \to \pi^\star)$ | 4.920 | 4.943 | 5.025 | 5.164 | 5.296 | 5.059 | 5.079 | 5.468 | 5.470 | 5.313 | 5.522 | 5.528 | 5.560 |
| | $^3B_{1g}$ $(n \to \pi^\star)$ | 2.320 | 2.419 | 2.509 | 2.518 | | 2.746 | 2.755 | 2.891 | 2.747 | 2.766 | 2.898 | 2.824 | 3.018 |
| | $^3A_u$ $(n \to \pi^\star)$ | 2.618 | 2.712 | 2.787 | 2.800 | | 3.025 | 3.032 | 3.154 | 3.016 | 3.014 | 3.146 | 3.073 | 3.282 |
| | $^3B_{1u}$ $(\pi \to \pi^\star)$ | 2.861 | 2.946 | 2.925 | 2.807 | | 2.954 | 2.968 | 2.971 | 3.125 | 3.023 | 3.307 | 3.256 | 3.282 |
| | $^3B_{3g}$ $(\pi \to \pi^\star)$ | 2.919 | 2.983 | 3.004 | 2.943 | | 2.962 | 2.974 | 3.164 | 3.290 | 3.153 | 3.502 | 3.469 | 3.492 |
| | $^3A_g$ $(\pi \to \pi^\star)$ | 2.997 | 3.045 | 3.091 | 3.134 | | 3.197 | 3.210 | 3.371 | 3.442 | 3.381 | 3.604 | 3.555 | 3.581 |
| Aza-BODIPY | $^1B_2$ $(\pi \to \pi^\star)$ | 2.847 | 2.829 | 2.839 | 2.867 | 2.893 | 2.794 | 2.812 | 2.871 | 2.880 | 2.782 | 2.833 | 2.807 | 2.834 |
| | $^1B_2$ $(\pi \to \pi^\star)$ | 3.303 | 3.304 | 3.350 | 3.430 | 3.488 | 3.380 | 3.394 | 3.651 | 3.650 | 3.553 | 3.697 | 3.715 | 3.739 |
| | $^1A_1$ $(\pi \to \pi^\star)$ | 3.343 | 3.373 | 3.455 | 3.564 | 3.670 | 3.529 | 3.543 | 3.861 | 3.851 | 3.754 | 3.911 | 3.938 | 3.960 |
| | $^1B_1$ $(n \to \pi^\star)$ | 3.540 | 3.530 | 3.612 | 3.665 | 3.761 | 3.548 | 3.572 | 3.965 | 3.750 | 3.556 | 3.735 | 3.679 | 3.897 |
| | $^3B_2$ $(\pi \to \pi^\star)$ | 1.131 | 1.144 | 1.063 | 0.876 | | 0.924 | 0.929 | 0.695 | 0.882 | 0.849 | 0.883 | 0.774 | 0.782 |
| | $^3B_2$ $(\pi \to \pi^\star)$ | 2.347 | 2.407 | 2.440 | 2.437 | | 2.510 | 2.526 | 2.664 | 2.719 | 2.664 | 2.818 | 2.826 | 2.849 |
| | $^3A_1$ $(\pi \to \pi^\star)$ | 2.567 | 2.632 | 2.671 | 2.671 | | 2.729 | 2.742 | 2.918 | 2.976 | 2.920 | 3.073 | 3.083 | 3.106 |
| | $^3B_1$ $(n \to \pi^\star)$ | 2.931 | 2.988 | 3.022 | 3.012 | | 3.128 | 3.151 | 3.323 | 3.163 | 3.152 | 3.229 | 3.188 | 3.389 |
| Azobenzene | $^1B_g$ $(n \to \pi^\star)$ | 2.570 | 2.552 | 2.623 | 2.636 | 2.628 | 2.506 | 2.547 | 2.847 | 2.660 | 2.486 | 2.615 | 2.521 | 2.822 |
| | $^1B_u$ $(\pi \to \pi^\star)$ | 3.661 | 3.650 | 3.698 | 3.805 | 3.817 | 3.688 | 3.711 | 3.989 | 4.017 | 3.919 | 4.098 | 4.085 | 4.121 |
| | $^1A_g$ $(\pi \to \pi^\star)$ | 3.919 | 3.956 | 4.071 | 4.236 | 4.353 | 4.130 | 4.135 | 4.611 | 4.627 | 4.528 | 4.752 | 4.755 | 4.761 |
| | $^1B_u$ $(\pi \to \pi^\star)$ | 3.922 | 3.957 | 4.068 | 4.231 | 4.350 | 4.124 | 4.130 | 4.600 | 4.616 | 4.517 | 4.737 | 4.742 | 4.747 |
| | $^1A_g$ $(\pi \to \pi^\star)$ | 4.614 | 4.656 | 4.758 | 4.925 | 5.016 | 4.773 | 4.787 | 5.266 | 5.297 | 5.191 | 5.407 | 5.415 | 5.434 |
| | $^3B_g$ $(n \to \pi^\star)$ | 1.755 | 1.869 | 1.862 | 1.786 | | 2.001 | 2.035 | 2.041 | 1.943 | 2.013 | 2.040 | 1.943 | 2.188 |
| | $^3B_u$ $(\pi \to \pi^\star)$ | 2.209 | 2.268 | 2.251 | 2.151 | | 2.190 | 2.202 | 2.285 | 2.465 | 2.377 | 2.697 | 2.672 | 2.699 |
| | $^3A_g$ $(\pi \to \pi^\star)$ | 3.380 | 3.449 | 3.483 | 3.408 | | 3.410 | 3.424 | 3.641 | 3.797 | 3.618 | 3.980 | 3.973 | 3.999 |
| | $^3B_u$ $(\pi \to \pi^\star)$ | 3.457 | 3.506 | 3.589 | 3.672 | | 3.621 | 3.635 | 3.999 | 4.063 | 3.967 | 4.205 | 4.192 | 4.217 |
| | $^3A_g$ $(\pi \to \pi^\star)$ | 3.559 | 3.621 | 3.673 | 3.733 | | 3.677 | 3.691 | 4.062 | 4.122 | 4.026 | 4.258 | 4.244 | 4.269 |
| BODIPY | $^1B_2$ $(\pi \to \pi^\star)$ | 3.134 | 3.110 | 3.114 | 3.148 | 3.191 | 3.062 | 3.084 | 3.174 | 3.161 | 3.066 | 3.114 | 3.100 | 3.131 |
| | $^1B_2$ $(\pi \to \pi^\star)$ | 3.564 | 3.577 | 3.640 | 3.739 | 3.834 | 3.700 | 3.714 | 4.006 | 3.988 | 3.885 | 4.037 | 4.065 | 4.087 |
| | $^1A_1$ $(\pi \to \pi^\star)$ | 3.666 | 3.699 | 3.785 | 3.904 | 4.035 | 3.872 | 3.884 | 4.226 | 4.202 | 4.101 | 4.257 | 4.293 | 4.313 |
| | $^3B_2$ $(\pi \to \pi^\star)$ | 1.602 | 1.637 | 1.591 | 1.498 | 0.340 | 1.536 | 1.547 | 1.494 | 1.566 | 1.537 | 1.590 | 1.532 | 1.549 |
| | $^3B_2$ $(\pi \to \pi^\star)$ | 2.657 | 2.720 | 2.754 | 2.759 | 2.324 | 2.837 | 2.850 | 2.990 | 3.044 | 2.987 | 3.115 | 3.159 | 3.181 |
| | $^3A_1$ $(\pi \to \pi^\star)$ | 2.854 | 2.922 | 2.960 | 2.960 | 2.289 | 3.033 | 3.046 | 3.214 | 3.269 | 3.206 | 3.367 | 3.384 | 3.406 |
| Coumarin | $^1A'$ $(\pi \to \pi^\star)$ | 4.098 | 4.109 | 4.170 | 4.272 | 4.381 | 4.200 | 4.213 | 4.491 | 4.486 | 4.360 | 4.495 | 4.508 | 4.530 |
| | $^1A''$ $(n \to \pi^\star)$ | 4.222 | 4.285 | 4.440 | 4.564 | 4.720 | 4.576 | 4.587 | 5.018 | 4.862 | 4.606 | 4.870 | 4.875 | 5.072 |
| | $^1A'$ $(\pi \to \pi^\star)$ | 4.561 | 4.560 | 4.620 | 4.743 | 4.806 | 4.619 | 4.640 | 4.977 | 5.002 | 4.859 | 5.050 | 5.049 | 5.074 |
| | $^3A'$ $(\pi \to \pi^\star)$ | 2.782 | 2.851 | 2.836 | 2.729 | | 2.812 | 2.830 | 2.906 | 3.027 | 2.902 | 3.146 | 3.129 | 3.163 |
| | $^3A'$ $(\pi \to \pi^\star)$ | 3.495 | 3.561 | 3.598 | 3.583 | | 3.619 | 3.634 | 3.849 | 3.929 | 3.818 | 4.055 | 4.052 | 4.076 |
| | $^3A''$ $(n \to \pi^\star)$ | 3.890 | 3.982 | 4.094 | 4.161 | | 4.339 | 4.348 | 4.605 | 4.465 | 4.380 | 4.556 | 4.527 | 4.717 |
| Cyclazine | $^1A'_2$ $(\pi \to \pi^\star)$ | 1.272 | 1.241 | 1.238 | 1.266 | 1.342 | 1.236 | 1.265 | 1.324 | 1.313 | 1.195 | 1.306 | 1.267 | 1.306 |
| | $^1E'$ $(\pi \to \pi^\star)$ | 3.124 | 3.117 | 3.124 | 3.206 | 3.325 | 3.074 | 3.106 | 3.325 | 3.353 | 3.246 | 3.241 | 3.305 | 3.332 |
| | $^1A''_1$ (Ryd) | 3.204 | 3.336 | 3.115 | 3.325 | 3.673 | 2.481 | 2.553 | 3.209 | 3.562 | 3.903 | 2.734 | 3.240 | 3.296 |
| | $^1E''$ (Ryd) | 3.558 | 3.726 | 3.494 | 3.717 | 4.110 | 2.761 | 2.826 | 3.570 | 3.895 | 4.385 | 3.131 | 3.660 | 3.706 |
| | $^3A'_2$ $(\pi \to \pi^\star)$ | 1.058 | 1.054 | 1.036 | 1.028 | 0.974 | 1.084 | 1.110 | 1.104 | 1.109 | 1.044 | 1.149 | 1.076 | 1.109 |
| | $^3E'$ $(\pi \to \pi^\star)$ | 1.996 | 2.035 | 2.010 | 1.976 | 1.722 | 2.012 | 2.026 | 2.106 | 2.148 | 2.070 | 2.183 | 2.164 | 2.184 |
| | $^3A''_1$ (Ryd) | 3.124 | 3.301 | 3.106 | 3.297 | 3.630 | 2.445 | 2.514 | 3.271 | 3.537 | 3.869 | 2.787 | 3.228 | 3.283 |
| | $^3E''$ (Ryd) | 3.547 | 3.674 | 3.492 | 3.697 | 4.083 | 2.729 | 2.786 | 3.633 | 3.857 | 4.365 | 3.205 | 3.632 | 3.677 |

Table S8: VTEs (in eV) computed with TD-DFT using the aug-cc-pVTZ basis set.

| Compound | State | TPSSh | τ-HCTHHyb | B3LYP | PBE0 | cSCAN0 | M06 | cM06 | SOGGA11-X | BMK | MN15 | M08-HX | M06-2X | cM06-2X |
|---|---|---|---|---|---|---|---|---|---|---|---|---|---|---|
| Heptazine | $^1A_2'$ ($\pi\to\pi^\star$) | 2.900 | 2.896 | 2.923 | 3.022 | 3.206 | 3.008 | 3.032 | 3.271 | 3.107 | 2.978 | 3.153 | 3.170 | 3.207 |
| | $^1A_1''$ ($n\to\pi^\star$) | 3.531 | 3.575 | 3.735 | 3.897 | 4.170 | 3.763 | 3.784 | 4.474 | 4.234 | 4.045 | 4.440 | 4.366 | 4.453 |
| | $^1E''$ ($n\to\pi^\star$) | 3.611 | 3.666 | 3.821 | 3.947 | 4.200 | 3.779 | 3.801 | 4.480 | 4.257 | 4.090 | 4.416 | 4.344 | 4.432 |
| | $^1E'$ ($\pi\to\pi^\star$) | 4.457 | 4.479 | 4.539 | 4.668 | 4.862 | 4.636 | 4.651 | 4.965 | 4.866 | 4.717 | 4.898 | 4.919 | 4.944 |
| | $^3A_2'$ ($\pi\to\pi^\star$) | 2.678 | 2.699 | 2.704 | 2.769 | 2.847 | 2.836 | 2.859 | 3.024 | 2.880 | 2.805 | 2.965 | 2.952 | 2.988 |
| | $^3E''(\pi\to\pi^\star)$ | 3.318 | 3.359 | 3.361 | 3.395 | 3.374 | 3.499 | 3.515 | 3.642 | 3.558 | 3.507 | 3.656 | 3.640 | 3.668 |
| | $^3A_1''$ ($n\to\pi^\star$) | 3.421 | 3.478 | 3.621 | 3.750 | 3.937 | 3.694 | 3.715 | 4.317 | 4.094 | 3.981 | 4.309 | 4.238 | 4.335 |
| | $^3E''$ ($n\to\pi^\star$) | 3.474 | 3.550 | 3.686 | 3.784 | 3.959 | 3.699 | 3.721 | 4.322 | 4.110 | 4.303 | 4.298 | 4.223 | 4.316 |
| Naphthalimide | $^1B_2$ ($\pi\to\pi^\star$) | 4.019 | 4.030 | 4.078 | 4.176 | 4.280 | 4.064 | 4.068 | 4.364 | 4.359 | 4.243 | 4.388 | 4.382 | 4.387 |
| | $^1B_1$ ($n\to\pi^\star$) | 3.417 | 3.524 | 3.713 | 3.853 | 4.024 | 3.871 | 3.876 | 4.385 | 4.237 | 4.037 | 4.324 | 4.314 | 4.485 |
| | $^1A_1$ ($\pi\to\pi^\star$) | 3.668 | 3.674 | 3.730 | 3.830 | 3.871 | 3.746 | 3.761 | 4.031 | 4.045 | 3.946 | 4.105 | 4.110 | 4.132 |
| | $^1A_2$ ($n\to\pi^\star$) | 3.978 | 4.068 | 4.241 | 4.364 | 4.537 | 4.382 | 4.389 | 4.846 | 4.676 | 4.434 | 4.703 | 4.695 | 4.876 |
| | $^3A_1$ ($\pi\to\pi^\star$) | 2.307 | 2.381 | 2.374 | 2.267 | | 2.330 | 2.341 | 2.436 | 2.564 | 2.447 | 2.718 | 2.708 | 2.729 |
| | $^3B_2$ ($\pi\to\pi^\star$) | 3.327 | 3.367 | 3.389 | 3.394 | | 3.394 | 3.411 | 3.594 | 3.649 | 3.553 | 3.740 | 3.711 | 3.738 |
| | $^3B_1$ ($n\to\pi^\star$) | 3.167 | 3.294 | 3.444 | 3.534 | | 3.686 | 3.691 | 4.044 | 3.906 | 3.855 | 4.058 | 4.014 | 4.182 |
| | $^3B_2$ ($\pi\to\pi^\star$) | 3.704 | 3.763 | 3.770 | 3.734 | | 3.741 | 3.763 | 3.936 | 4.024 | 3.877 | 4.118 | 4.088 | 4.125 |
| | $^3A_2$ ($n\to\pi^\star$) | 3.699 | 3.805 | 3.933 | 4.002 | | 4.167 | 4.174 | 4.468 | 4.313 | 4.229 | 4.417 | 4.376 | 4.554 |
| Naphthoquinone | $^1B_1$ ($n\to\pi^\star$) | 2.540 | 2.571 | 2.703 | 2.758 | 2.844 | 2.787 | 2.800 | 3.120 | 2.943 | 2.763 | 2.979 | 2.950 | 3.170 |
| | $^1A_2$ ($n\to\pi^\star$) | 2.785 | 2.822 | 2.947 | 3.022 | 3.095 | 3.046 | 3.054 | 3.371 | 3.213 | 3.014 | 3.248 | 3.216 | 3.458 |
| | $^1A_1$ ($\pi\to\pi^\star$) | 3.460 | 3.497 | 3.601 | 3.756 | 3.869 | 3.716 | 3.721 | 4.117 | 4.124 | 4.035 | 4.293 | 4.290 | 4.297 |
| | $^1B_2$ ($\pi\to\pi^\star$) | 3.474 | 3.490 | 3.583 | 3.721 | 3.798 | 3.664 | 3.682 | 4.036 | 4.044 | 3.949 | 4.199 | 4.190 | 4.218 |
| | $^1A_2$ ($n\to\pi^\star$) | 4.493 | 4.607 | 4.862 | 5.051 | 5.327 | 5.036 | 5.050 | 5.851 | 5.711 | 5.518 | 5.946 | 5.958 | 6.021 |
| | $^1A_1$ ($\pi\to\pi^\star$) | 5.288 | 5.286 | 5.334 | 5.454 | 5.600 | 5.307 | 5.317 | 5.701 | 5.702 | 5.536 | 5.717 | 5.726 | 5.744 |
| | $^1B_2$ ($\pi\to\pi^\star$) | 4.777 | 4.794 | 4.877 | 4.998 | 5.104 | 4.944 | 4.968 | 5.272 | 5.280 | 5.171 | 5.356 | 5.352 | 5.389 |
| | $^3B_1$ ($n\to\pi^\star$) | 2.048 | 2.143 | 2.239 | 2.238 | | 2.480 | 2.491 | 2.626 | 2.486 | 2.519 | 2.639 | 2.577 | 2.776 |
| | $^3A_2$ ($n\to\pi^\star$) | 2.288 | 2.389 | 2.473 | 2.488 | | 2.730 | 2.737 | 2.863 | 2.738 | 2.747 | 2.884 | 2.820 | 3.038 |
| | $^3B_2$ ($\pi\to\pi^\star$) | 2.634 | 2.724 | 2.695 | 2.547 | | 2.774 | 2.795 | 2.705 | 2.875 | 2.815 | 3.046 | 3.000 | 3.036 |
| | $^3B_2$ ($\pi\to\pi^\star$) | 2.763 | 2.830 | 2.859 | 2.809 | | 2.849 | 2.866 | 3.049 | 3.162 | 3.051 | 3.365 | 3.336 | 3.365 |
| | $^3A_1$ ($\pi\to\pi^\star$) | 2.887 | 2.934 | 3.001 | 3.074 | | 3.108 | 3.119 | 3.358 | 3.418 | 3.362 | 3.607 | 3.567 | 3.588 |
| Phenazine | $^1B_{1u}$ ($n\to\pi^\star$) | 2.942 | 2.975 | 3.112 | 3.148 | | 3.093 | 3.112 | 3.502 | 3.322 | 3.189 | 3.349 | 3.292 | 3.472 |
| | $^1B_{3u}$ ($\pi\to\pi^\star$) | 3.084 | 3.094 | 3.162 | 3.256 | | 3.180 | 3.194 | 3.463 | 3.503 | 3.400 | 3.601 | 3.586 | 3.606 |
| | $^1B_{2u}$ ($\pi\to\pi^\star$) | 3.829 | 3.825 | 3.857 | 3.927 | | 3.802 | 3.807 | 4.050 | 4.071 | 3.946 | 4.086 | 4.063 | 4.069 |
| | $^1B_{1g}$ ($\pi\to\pi^\star$) | 3.915 | 3.942 | 4.042 | 4.176 | | 4.076 | 4.091 | 4.501 | 4.543 | 4.419 | 4.656 | 4.651 | 4.675 |
| | $^1B_{2g}$ ($n\to\pi^\star$) | 4.558 | 4.566 | 4.689 | 4.812 | | 4.712 | 4.730 | 5.255 | 5.048 | 4.775 | 5.107 | 5.053 | 5.294 |
| | $^1A_u$ ($\pi\to\pi^\star$) | 4.651 | 4.706 | 4.889 | 4.992 | | 4.885 | 4.911 | 5.552 | 5.320 | 5.172 | 5.430 | 5.375 | 5.462 |
| | $^3B_{3u}$ ($\pi\to\pi^\star$) | 1.855 | 1.929 | 1.914 | 1.787 | | 1.865 | 1.874 | 1.901 | 2.085 | 1.988 | 2.301 | 2.275 | 2.292 |
| | $^3B_{1u}$ ($n\to\pi^\star$) | 2.455 | 2.544 | 2.635 | 2.618 | | 2.761 | 2.779 | 2.973 | 2.844 | 2.881 | 2.953 | 2.895 | 3.068 |
| | $^3B_{2u}$ ($\pi\to\pi^\star$) | 3.016 | 3.027 | 3.039 | 3.030 | | 2.974 | 2.989 | 3.140 | 3.227 | 3.121 | 3.285 | 3.227 | 3.250 |
| | $^3B_{1g}$ ($\pi\to\pi^\star$) | 3.071 | 3.138 | 3.155 | 3.082 | | 3.078 | 3.096 | 3.292 | 3.429 | 3.290 | 3.558 | 3.559 | 3.591 |
| Phthalimide | $^1B_1$ ($n\to\pi^\star$) | 3.613 | 3.669 | 3.801 | 3.891 | 4.026 | 3.902 | 3.909 | 4.290 | 4.121 | 3.906 | 4.163 | 4.131 | 4.333 |
| | $^1A_1$ ($\pi\to\pi^\star$) | 4.537 | 4.545 | 4.601 | 4.717 | 4.839 | 4.598 | 4.603 | 4.946 | 4.938 | 4.810 | 4.997 | 4.985 | 4.990 |
| | $^1A_2$ ($n\to\pi^\star$) | 4.283 | 4.324 | 4.445 | 4.534 | 4.662 | 4.530 | 4.541 | 4.909 | 4.733 | 4.474 | 4.728 | 4.706 | 4.922 |
| | $^1B_2$ ($\pi\to\pi^\star$) | 4.384 | 4.396 | 4.470 | 4.590 | 4.678 | 4.514 | 4.535 | 4.866 | 4.834 | 4.725 | 4.916 | 4.925 | 4.960 |
| | $^1B_2$ ($\pi\to\pi^\star$) | 5.399 | 5.453 | 5.545 | 5.682 | 5.819 | 5.659 | 5.680 | 5.995 | 5.981 | 5.842 | 5.994 | 6.024 | 6.055 |
| | $^1A_2$ ($n\to\pi^\star$) | 4.784 | 4.931 | 5.199 | 5.418 | 5.701 | 5.393 | 5.403 | 6.249 | 6.159 | 5.956 | 6.415 | 6.420 | 6.481 |
| | $^1A_1$ ($\pi\to\pi^\star$) | 5.984 | 5.911 | 5.977 | 6.096 | 6.223 | 5.935 | 5.970 | 6.319 | 6.305 | 6.138 | 6.290 | 6.303 | 6.353 |
| | $^3B_2$ ($\pi\to\pi^\star$) | 3.251 | 3.341 | 3.330 | 3.203 | | 3.243 | 3.256 | 3.413 | 3.573 | 3.412 | 3.785 | 3.757 | 3.784 |
| | $^3B_1$ ($n\to\pi^\star$) | 3.204 | 3.306 | 3.405 | 3.443 | | 3.637 | 3.645 | 3.858 | 3.712 | 3.687 | 3.850 | 3.784 | 3.974 |
| | $^3A_1$ ($\pi\to\pi^\star$) | 3.797 | 3.828 | 3.863 | 3.905 | | 3.880 | 3.910 | 4.141 | 4.188 | 4.090 | 4.309 | 4.263 | 4.296 |
| | $^3B_2$ ($\pi\to\pi^\star$) | 3.868 | 3.951 | 3.987 | 3.990 | | 4.192 | 4.221 | 4.289 | 4.276 | 4.256 | 4.326 | 4.311 | 4.352 |
| | $^3A_2$ ($n\to\pi^\star$) | 3.856 | 3.942 | 4.026 | 4.060 | | 4.248 | 4.258 | 4.455 | 4.303 | 4.235 | 4.397 | 4.343 | 4.548 |
| | $^3B_2$ ($\pi\to\pi^\star$) | 4.210 | 4.257 | 4.276 | 4.263 | | 4.312 | 4.337 | 4.505 | 4.591 | 4.414 | 4.651 | 4.666 | 4.717 |
| Tolan | $^1B_{2u}$ ($\pi\to\pi^\star$) | 4.526 | 4.547 | 4.621 | 4.760 | 4.900 | 4.638 | 4.647 | 5.018 | 5.030 | 4.905 | 5.030 | 5.061 | 5.067 |
| | $^1B_{3g}$ ($\pi\to\pi^\star$) | 4.560 | 4.582 | 4.661 | 4.797 | 4.936 | 4.683 | 4.689 | 5.057 | 5.063 | 4.936 | 5.082 | 5.098 | 5.103 |
| | $^1B_{1u}$ ($\pi\to\pi^\star$) | 4.080 | 4.069 | 4.118 | 4.213 | 4.190 | 4.088 | 4.113 | 4.376 | 4.409 | 4.293 | 4.488 | 4.483 | 4.524 |
| | $^1A_u$ ($\pi\to\pi^\star$) | 4.671 | 4.662 | 4.756 | 4.847 | 4.877 | 4.748 | 4.789 | 5.098 | 5.006 | 4.837 | 4.970 | 4.944 | 5.163 |
| | $^1B_{3u}$ (Ryd) | 5.147 | 5.294 | 5.117 | 5.381 | 5.755 | 4.436 | 4.471 | 5.384 | 5.746 | 6.039 | 4.955 | 5.470 | 5.511 |
| | $^3B_{1u}$ ($\pi\to\pi^\star$) | 2.654 | 2.728 | 2.740 | 2.627 | | 2.698 | 2.715 | 2.842 | 2.959 | 2.811 | 3.149 | 3.150 | 3.185 |
| | $^3A_g$ ($\pi\to\pi^\star$) | 3.646 | 3.759 | 3.727 | 3.565 | | 3.582 | 3.595 | 3.781 | 3.973 | 3.764 | 4.163 | 4.168 | 4.194 |

Table S9: VTEs (in eV) computed with TD-DFT using the aug-cc-pVTZ basis set.

| Compound | State | M06-SX | cM06-SX | CAM-BLYP | tCAM-B3LYP | mCAM-B3LYP | rCAM-B3LYP | ωB97X-D | ωB97M-V | ωB97X | ωB97 | LC-ωPBE | M11 |
|---|---|---|---|---|---|---|---|---|---|---|---|---|---|
| Anthracene | $^1B_{1u}$ ($\pi \to \pi^\star$) | 3.379 | 3.372 | 3.520 | 3.300 | 3.333 | 3.733 | 3.558 | 3.626 | 3.690 | 3.762 | 3.786 | 3.685 |
| | $^1B_{2u}$ ($\pi \to \pi^\star$) | 4.081 | 4.080 | 4.057 | 3.903 | 3.957 | 4.114 | 4.077 | 4.096 | 4.121 | 4.140 | 4.135 | 4.191 |
| | $^1B_{3g}$ ($\pi \to \pi^\star$) | 4.900 | 4.898 | 5.119 | 4.811 | 4.834 | 5.297 | 5.154 | 5.708 | 5.287 | 5.364 | 5.391 | 5.251 |
| | $^1B_{2g}$ (Ryd) | 5.401 | 5.394 | 5.073 | 4.668 | 4.815 | 5.252 | 5.334 | 4.886 | 5.611 | 5.717 | 5.736 | 4.644 |
| | $^1B_{1u}$ ($\pi \to \pi^\star$) | 5.462 | 5.452 | 5.378 | 4.963 | 5.128 | 5.637 | 5.534 | 5.307 | 5.735 | 5.847 | 5.886 | 5.205 |
| | $^1B_{3g}$ ($\pi \to \pi^\star$) | 5.079 | 5.066 | 5.330 | 4.860 | 4.944 | 6.175 | 5.456 | 5.189 | 5.837 | 6.061 | 6.067 | 5.780 |
| | $^1A_g$ ($\pi \to \pi^\star$) | 5.851 | 5.850 | 5.839 | 5.519 | 5.650 | 6.078 | 5.846 | 5.926 | 5.999 | 6.100 | 6.093 | 6.056 |
| | $^1B_{3u}$ (Ryd) | 5.599 | 5.595 | 5.346 | 4.935 | 5.058 | 5.596 | 5.622 | 5.211 | 5.987 | 6.081 | 6.039 | 4.889 |
| | $^1A_u$ (Ryd) | 5.591 | 5.586 | 5.404 | 5.021 | 5.076 | 5.673 | 5.711 | 5.315 | 6.056 | 6.151 | 6.132 | 5.031 |
| | $^1B_{2u}$ ($\pi \to \pi^\star$) | 5.375 | 5.353 | 5.383 | 5.189 | 5.251 | 5.566 | 5.414 | 5.413 | 5.505 | 5.560 | 5.568 | 5.445 |
| | $^3B_{1u}$ ($\pi \to \pi^\star$) | 1.952 | 1.946 | 1.647 | 1.960 | 1.772 | | 1.782 | 1.954 | 1.564 | 1.373 | 0.973 | 1.751 |
| | $^3B_{3g}$ ($\pi \to \pi^\star$) | 3.499 | 3.488 | 3.236 | 3.399 | 3.274 | | 3.342 | 3.487 | 3.249 | 3.180 | 2.973 | 3.365 |
| | $^3B_{2u}$ ($\pi \to \pi^\star$) | 3.697 | 3.680 | 3.642 | 3.567 | 3.559 | | 3.700 | 3.765 | 3.737 | 3.753 | 3.677 | 3.759 |
| Anthraquinone | $^1B_{1g}$ ($n \to \pi^\star$) | 3.056 | 3.035 | 3.316 | 2.900 | 3.104 | 3.749 | 3.288 | 3.416 | 3.442 | 3.510 | 3.449 | 3.174 |
| | $^1A_u$ ($n \to \pi^\star$) | 3.397 | 3.372 | 3.579 | 3.201 | 3.387 | 3.947 | 3.555 | 3.670 | 3.690 | 3.754 | 3.692 | 3.431 |
| | $^1A_g$ ($\pi \to \pi^\star$) | 4.189 | 4.186 | 4.386 | 3.969 | 4.086 | 4.740 | 4.414 | 4.579 | 4.630 | 4.744 | 4.742 | 4.686 |
| | $^1B_{2u}$ ($\pi \to \pi^\star$) | 4.200 | 4.197 | 4.371 | 3.953 | 4.083 | 4.703 | 4.387 | 4.556 | 4.601 | 4.715 | 4.710 | 4.658 |
| | $^1B_{3g}$ ($\pi \to \pi^\star$) | 4.004 | 3.996 | 4.171 | 3.779 | 3.897 | 4.529 | 4.197 | 4.370 | 4.423 | 4.555 | 4.563 | 4.459 |
| | $^1B_{1u}$ ($\pi \to \pi^\star$) | 4.832 | 4.826 | 5.014 | 4.672 | 4.745 | 5.202 | 5.050 | 5.150 | 5.214 | 5.293 | 5.312 | 5.237 |
| | $^1B_{2u}$ ($\pi \to \pi^\star$) | 5.356 | 5.347 | 5.499 | 5.134 | 5.227 | 5.895 | 5.551 | 5.651 | 5.740 | 5.852 | 5.855 | 5.748 |
| | $^3B_{1g}$ ($n \to \pi^\star$) | 2.703 | 2.684 | 2.821 | 2.483 | 2.643 | 3.142 | 2.829 | 3.045 | 2.962 | 3.031 | 2.883 | 2.794 |
| | $^3A_u$ ($n \to \pi^\star$) | 3.023 | 3.000 | 3.068 | 2.765 | 2.907 | 3.333 | 3.081 | 3.286 | 3.199 | 3.267 | 3.116 | 3.047 |
| | $^3B_{1u}$ ($\pi \to \pi^\star$) | 3.091 | 3.083 | 2.828 | 3.063 | 2.889 | 1.837 | 2.957 | 3.142 | 2.835 | 2.741 | 2.480 | 3.022 |
| | $^3B_{3g}$ ($\pi \to \pi^\star$) | 3.222 | 3.216 | 2.996 | 3.104 | 3.011 | 2.094 | 3.115 | 3.315 | 3.011 | 2.903 | 2.656 | 3.182 |
| | $^3A_g$ ($\pi \to \pi^\star$) | 3.351 | 3.344 | 3.386 | 3.206 | 3.217 | 3.447 | 3.447 | 3.624 | 3.571 | 3.653 | 3.580 | 3.654 |
| Aza-BODIPY | $^1B_2$ ($\pi \to \pi^\star$) | 2.912 | 2.903 | 2.799 | 2.803 | 2.835 | 2.645 | 2.801 | | 2.727 | 2.671 | 2.682 | 2.763 |
| | $^1B_2$ ($\pi \to \pi^\star$) | 3.559 | 3.552 | 3.628 | 3.334 | 3.452 | 3.986 | 3.641 | | 3.814 | 3.924 | 3.925 | 3.828 |
| | $^1A_1$ ($\pi \to \pi^\star$) | 3.732 | 3.725 | 3.863 | 3.482 | 3.616 | 4.270 | 3.870 | | 4.077 | 4.198 | 4.188 | 4.082 |
| | $^1B_1$ ($n \to \pi^\star$) | 3.733 | 3.709 | 3.835 | 3.463 | 3.707 | 4.196 | 3.779 | | 3.905 | 3.979 | 3.917 | 3.617 |
| | $^3B_2$ ($\pi \to \pi^\star$) | 1.032 | 1.028 | | 0.976 | 0.811 | | | | | | | |
| | $^3B_2$ ($\pi \to \pi^\star$) | 2.661 | 2.654 | | 2.491 | 2.497 | | | | | | | |
| | $^3A_1$ ($\pi \to \pi^\star$) | 2.909 | 2.903 | | 2.726 | 2.734 | | | | | | | |
| | $^3B_1$ ($n \to \pi^\star$) | 3.235 | 3.212 | | 2.894 | 3.076 | | | | | | | |
| Azobenzene | $^1B_g$ ($n \to \pi^\star$) | 2.660 | 2.624 | 2.786 | 2.557 | 2.700 | 3.041 | 2.752 | 2.820 | 2.834 | 2.880 | 2.808 | 2.511 |
| | $^1B_u$ ($\pi \to \pi^\star$) | 3.930 | 3.919 | 4.008 | 3.748 | 3.824 | 4.252 | 4.044 | 4.137 | 4.188 | 4.283 | 4.316 | 4.220 |
| | $^1A_g$ ($\pi \to \pi^\star$) | 4.451 | 4.448 | 4.670 | 4.207 | 4.331 | 5.034 | 4.700 | 4.878 | 4.920 | 5.027 | 5.027 | 4.988 |
| | $^1B_u$ ($\pi \to \pi^\star$) | 4.446 | 4.444 | 4.656 | 4.193 | 4.322 | 5.019 | 4.686 | 4.862 | 4.906 | 5.014 | 5.015 | 4.974 |
| | $^1A_g$ ($\pi \to \pi^\star$) | 5.110 | 5.106 | 5.338 | 4.983 | 5.017 | 5.594 | 5.407 | 5.519 | 5.580 | 5.666 | 5.701 | 5.620 |
| | $^3B_g$ ($n \to \pi^\star$) | 2.051 | 2.020 | 1.927 | 1.837 | 1.891 | 1.946 | 1.977 | 2.192 | 2.031 | 2.084 | 1.844 | 1.845 |
| | $^3B_u$ ($\pi \to \pi^\star$) | 2.417 | 2.410 | 2.150 | 2.367 | 2.211 | 0.934 | 2.283 | 2.496 | 2.186 | 2.121 | 1.882 | 2.375 |
| | $^3A_g$ ($\pi \to \pi^\star$) | 3.724 | 3.717 | 3.431 | 3.619 | 3.482 | 2.443 | 3.578 | 3.774 | 3.428 | 3.297 | 3.025 | 3.597 |
| | $^3B_u$ ($\pi \to \pi^\star$) | 3.932 | 3.925 | 3.977 | 3.703 | 3.766 | 3.490 | 4.047 | 4.243 | 4.129 | 4.387 | 4.301 | 4.232 |
| | $^3A_g$ ($\pi \to \pi^\star$) | 3.993 | 3.986 | 4.058 | 3.795 | 3.826 | 4.271 | 4.111 | 4.307 | 4.268 | 4.351 | 4.279 | 4.316 |
| BODIPY | $^1B_2$ ($\pi \to \pi^\star$) | 3.205 | 3.194 | 3.104 | 3.083 | 3.116 | 3.020 | 3.110 | 3.045 | 3.073 | 3.044 | 3.043 | 3.086 |
| | $^1B_2$ ($\pi \to \pi^\star$) | 3.894 | 3.887 | 4.009 | 3.644 | 3.779 | 4.399 | 4.012 | 4.150 | 4.220 | 4.351 | 4.343 | 4.218 |
| | $^1A_1$ ($\pi \to \pi^\star$) | 4.087 | 4.081 | 4.239 | 3.826 | 3.965 | 4.670 | 4.246 | 4.411 | 4.478 | 4.617 | 4.600 | 4.467 |
| | $^3B_2$ ($\pi \to \pi^\star$) | 1.655 | 1.648 | 1.298 | 1.557 | 1.479 | | 1.343 | 1.318 | 1.120 | 0.943 | 0.701 | 1.263 |
| | $^3B_2$ ($\pi \to \pi^\star$) | 2.994 | 2.987 | 2.928 | 2.813 | 2.821 | | 2.985 | 3.151 | 3.058 | 3.101 | 2.980 | 3.133 |
| | $^3A_1$ ($\pi \to \pi^\star$) | 3.212 | 3.205 | 3.122 | 3.021 | 3.025 | | 3.175 | 3.355 | 3.226 | 3.247 | 3.102 | 3.303 |
| Coumarin | $^1A'$ ($\pi \to \pi^\star$) | 4.431 | 4.424 | 4.463 | 4.164 | 4.295 | 4.655 | 4.471 | 4.530 | 4.592 | 4.658 | 4.663 | 4.601 |
| | $^1A''$ ($n \to \pi^\star$) | 4.743 | 4.723 | 4.937 | 4.384 | 4.656 | 5.400 | 4.908 | 5.078 | 5.112 | 5.212 | 5.148 | 4.869 |
| | $^1A'$ ($\pi \to \pi^\star$) | 4.907 | 4.898 | 4.974 | 4.668 | 4.771 | 5.144 | 5.001 | 5.074 | 5.134 | 5.201 | 5.216 | 5.175 |
| | $^3A'$ ($\pi \to \pi^\star$) | 3.004 | 2.994 | 2.727 | 2.918 | 2.789 | 1.826 | 2.844 | 2.996 | 2.729 | 2.636 | 2.387 | 2.871 |
| | $^3A'$ ($\pi \to \pi^\star$) | 3.865 | 3.857 | 3.707 | 3.658 | 3.653 | 3.202 | 3.794 | 3.964 | 3.773 | 3.733 | 3.535 | 3.880 |
| | $^3A''$ ($n \to \pi^\star$) | 4.434 | 4.414 | 4.494 | 4.051 | 4.267 | 4.831 | 4.502 | 4.741 | 4.674 | 4.770 | 4.625 | 4.508 |
| Cyclazine | $^1A'_2$ ($\pi \to \pi^\star$) | 1.332 | 1.318 | 1.270 | 1.197 | 1.247 | 1.366 | 1.286 | 1.291 | 1.303 | 1.315 | 1.303 | 1.352 |
| | $^1E'$ ($\pi \to \pi^\star$) | 3.343 | 3.336 | 3.319 | 3.117 | 3.202 | 3.526 | 3.365 | 3.338 | 3.453 | 3.509 | 3.514 | 3.367 |
| | $^1A''_1$ (Ryd) | 3.752 | 3.743 | 3.375 | 3.054 | 3.192 | 3.531 | 3.646 | 3.139 | 3.849 | 3.928 | 3.940 | 2.909 |
| | $^1E''$ (Ryd) | 4.110 | 4.104 | 3.833 | 3.539 | 3.602 | 4.056 | 4.118 | 3.679 | 4.423 | 4.473 | 4.427 | 3.313 |
| | $^3A'_2$ ($\pi \to \pi^\star$) | 1.154 | 1.143 | 1.013 | 1.002 | 1.024 | 0.973 | 1.051 | 1.082 | 1.028 | 1.009 | 0.927 | 1.100 |
| | $^3E'$ ($\pi \to \pi^\star$) | 2.184 | 2.178 | 1.963 | 1.996 | 1.988 | 1.770 | 2.030 | 2.080 | 1.991 | 1.976 | 1.829 | 2.071 |
| | $^3A''_1$ (Ryd) | 3.734 | 3.726 | 3.364 | 3.052 | 3.189 | 3.523 | 3.629 | 3.182 | 3.843 | 3.908 | 3.908 | 2.964 |
| | $^3E''$ (Ryd) | 4.071 | 4.066 | 3.830 | 3.542 | 3.605 | 4.055 | 4.074 | 3.707 | 4.368 | 4.418 | 4.402 | 3.397 |

Table S10: VTEs (in eV) computed with TD-DFT using the aug-cc-pVTZ basis set.

| Compound | State | M06-SX | cM06-SX | CAM-BLYP | tCAM-B3LYP | mCAM-B3LYP | rCAM-B3LYP | ωB97X-D | ωB97M-V | ωB97X | ωB97 | LC-ωPBE | M11 |
|---|---|---|---|---|---|---|---|---|---|---|---|---|---|
| Heptazine | $^1A_2'$ $(\pi \to \pi^\star)$ | 3.174 | 3.162 | 3.141 | 2.871 | 3.008 | 3.427 | 3.164 | 3.229 | 3.279 | 3.344 | 3.289 | 3.254 |
| | $^1A_1''$ $(n \to \pi^\star)$ | 4.146 | 4.137 | 4.233 | 3.557 | 3.952 | 4.841 | 4.212 | 4.379 | 4.409 | 4.492 | 4.412 | 4.370 |
| | $^1E''$ $(n \to \pi^\star)$ | 4.158 | 4.149 | 4.279 | 3.683 | 4.021 | 4.829 | 4.244 | 4.396 | 4.429 | 4.504 | 4.416 | 4.358 |
| | $^1E'$ $(\pi \to \pi^\star)$ | 4.860 | 4.852 | 4.889 | 4.518 | 4.684 | 5.218 | 4.908 | 4.983 | 5.070 | 5.163 | 5.131 | 5.022 |
| | $^3A_2'$ $(\pi \to \pi^\star)$ | 2.974 | 2.961 | 2.873 | 2.661 | 2.770 | 3.075 | 2.916 | 3.003 | 3.003 | 3.051 | 2.952 | 2.991 |
| | $^3E''(\pi \to \pi^\star)$ | 3.648 | 3.640 | 3.486 | 3.352 | 3.408 | 3.556 | 3.545 | 3.653 | 3.616 | 3.674 | 3.548 | 3.627 |
| | $^3A_1''$ $(n \to \pi^\star)$ | 4.044 | 4.034 | 4.074 | 3.451 | 3.817 | 4.615 | 4.069 | 4.274 | 4.256 | 4.341 | 4.216 | 4.204 |
| | $^3E''$ $(n \to \pi^\star)$ | 4.048 | 4.039 | 4.111 | 3.553 | 3.871 | 4.607 | 4.094 | 4.289 | 4.271 | 4.348 | 4.214 | 4.197 |
| Naphthalimide | $^1B_2$ $(\pi \to \pi^\star)$ | 4.326 | 4.324 | 4.320 | 4.085 | 4.183 | 4.437 | 4.331 | 4.385 | 4.418 | 4.464 | 4.458 | 4.479 |
| | $^1B_1$ $(n \to \pi^\star)$ | 4.053 | 4.037 | 4.337 | 3.727 | 3.987 | 4.886 | 4.320 | 4.517 | 4.547 | 4.649 | 4.583 | 4.347 |
| | $^1A_1$ $(\pi \to \pi^\star)$ | 3.961 | 3.954 | 4.057 | 3.782 | 3.865 | 4.264 | 4.083 | 4.171 | 4.229 | 4.309 | 4.328 | 4.234 |
| | $^1A_2$ $(n \to \pi^\star)$ | 4.525 | 4.508 | 4.753 | 4.224 | 4.473 | 5.212 | 4.731 | 4.883 | 4.913 | 4.995 | 4.920 | 4.671 |
| | $^3A_1$ $(\pi \to \pi^\star)$ | 2.529 | 2.522 | 2.254 | 2.462 | 2.327 | 1.068 | 2.368 | 2.537 | 2.220 | 2.091 | 1.820 | 2.374 |
| | $^3B_2$ $(\pi \to \pi^\star)$ | 3.618 | 3.610 | 3.503 | 3.445 | 3.440 | 3.180 | 3.567 | 3.681 | 3.577 | 3.569 | 3.439 | 3.654 |
| | $^3B_1$ $(n \to \pi^\star)$ | 3.809 | 3.792 | 3.961 | 3.451 | 3.672 | 4.385 | 3.970 | 4.221 | 4.164 | 4.261 | 4.121 | 4.027 |
| | $^3B_2$ $(\pi \to \pi^\star)$ | 4.001 | 3.990 | 3.800 | 3.819 | 3.776 | 3.648 | 3.870 | 3.990 | 3.864 | 3.864 | 3.755 | 3.951 |
| | $^3A_2$ $(n \to \pi^\star)$ | 4.250 | 4.233 | 4.344 | 3.911 | 4.116 | 4.694 | 4.352 | 4.569 | 4.508 | 4.588 | 4.438 | 4.333 |
| Naphthoquinone | $^1B_1$ $(n \to \pi^\star)$ | 2.813 | 2.790 | 3.087 | 2.650 | 2.869 | 3.576 | 3.045 | 3.198 | 3.222 | 3.309 | 3.241 | 2.926 |
| | $^1A_2$ $(n \to \pi^\star)$ | 3.123 | 3.095 | 3.340 | 2.907 | 3.118 | 3.776 | 3.308 | 3.463 | 3.478 | 3.563 | 3.508 | 3.209 |
| | $^1A_1$ $(\pi \to \pi^\star)$ | 3.958 | 3.956 | 4.184 | 3.680 | 3.844 | 4.623 | 4.194 | 4.421 | 4.471 | 4.619 | 4.615 | 4.516 |
| | $^1B_2$ $(\pi \to \pi^\star)$ | 3.899 | 3.890 | 4.070 | 3.626 | 3.783 | 4.476 | 4.071 | 4.271 | 4.327 | 4.484 | 4.488 | 4.345 |
| | $^1A_2$ $(n \to \pi^\star)$ | 5.300 | 5.295 | 5.826 | 4.806 | 5.249 | 7.000 | 5.790 | 6.156 | 6.251 | 6.463 | 6.423 | 6.176 |
| | $^1A_1$ $(\pi \to \pi^\star)$ | 5.656 | 5.651 | 5.667 | 5.326 | 5.463 | 5.991 | 5.691 | 5.781 | 5.864 | 5.975 | 5.973 | 5.895 |
| | $^1B_2$ $(\pi \to \pi^\star)$ | 5.173 | 5.161 | 5.289 | 4.899 | 5.046 | 5.555 | 5.281 | 5.398 | 5.480 | 5.599 | 5.609 | 5.467 |
| | $^3B_1$ $(n \to \pi^\star)$ | 2.435 | 2.414 | 2.566 | 2.205 | 2.378 | 2.940 | 2.563 | 2.811 | 2.720 | 2.808 | 2.653 | 2.534 |
| | $^3A_2$ $(n \to \pi^\star)$ | 2.728 | 2.703 | 2.803 | 2.451 | 2.614 | 3.126 | 2.811 | 3.059 | 2.961 | 3.049 | 2.903 | 2.808 |
| | $^3B_2$ $(\pi \to \pi^\star)$ | 2.843 | 2.832 | 2.588 | 2.826 | 2.645 | 1.715 | 2.699 | 2.897 | 2.621 | 2.585 | 2.334 | 2.779 |
| | $^3B_2$ $(\pi \to \pi^\star)$ | 3.086 | 3.077 | 2.903 | 2.938 | 2.884 | 2.181 | 2.999 | 3.209 | 2.943 | 2.808 | 2.640 | 3.089 |
| | $^3A_1$ $(\pi \to \pi^\star)$ | 3.301 | 3.295 | 3.379 | 3.092 | 3.162 | 3.518 | 3.420 | 3.638 | 3.593 | 3.696 | 3.626 | 3.666 |
| Phenazine | $^1B_{1u}$ $(n \to \pi^\star)$ | 3.190 | 3.172 | 3.465 | 3.007 | 3.262 | 3.967 | 3.390 | 3.549 | 3.574 | 3.661 | 3.607 | 3.314 |
| | $^1B_{3u}$ $(\pi \to \pi^\star)$ | 3.368 | 3.362 | 3.538 | 3.263 | 3.328 | 3.823 | 3.572 | 3.689 | 3.742 | 3.838 | 3.861 | 3.767 |
| | $^1B_{2u}$ $(\pi \to \pi^\star)$ | 4.040 | 4.038 | 4.007 | 3.870 | 3.924 | 4.025 | 4.020 | 4.033 | 4.049 | 4.054 | 4.057 | 4.130 |
| | $^1B_{1g}$ $(\pi \to \pi^\star)$ | 4.348 | 4.341 | 4.597 | 4.203 | 4.272 | 5.037 | 4.640 | 4.830 | 4.882 | 5.012 | 5.024 | 4.906 |
| | $^1B_{2g}$ $(n \to \pi^\star)$ | 4.978 | 4.951 | 5.121 | 4.561 | 4.872 | 5.618 | 5.081 | 5.282 | 5.311 | 5.452 | 5.371 | 5.083 |
| | $^1A_u$ $(\pi \to \pi^\star)$ | 5.148 | 5.141 | 5.427 | 4.745 | 5.113 | 6.147 | 5.361 | 5.556 | 5.612 | 5.707 | 5.632 | 5.439 |
| | $^3B_{3u}$ $(\pi \to \pi^\star)$ | 2.024 | 2.019 | 1.750 | 2.046 | 1.856 | | 1.889 | 2.066 | 1.709 | 1.561 | 1.240 | 1.920 |
| | $^3B_{1u}$ $(n \to \pi^\star)$ | 2.797 | 2.780 | 2.905 | 2.557 | 2.749 | | 2.880 | 3.132 | 3.031 | 3.116 | 2.970 | 2.842 |
| | $^3B_{2u}$ $(\pi \to \pi^\star)$ | 3.201 | 3.194 | 3.062 | 3.068 | 3.051 | | 3.104 | 3.150 | 3.068 | 3.030 | 2.962 | 3.177 |
| | $^3B_{1g}$ $(\pi \to \pi^\star)$ | 3.350 | 3.341 | 3.149 | 3.263 | 3.154 | | 3.248 | 3.412 | 3.176 | 3.112 | 2.912 | 3.292 |
| Phthalimide | $^1B_1$ $(n \to \pi^\star)$ | 4.030 | 4.008 | 4.229 | 3.746 | 3.985 | 4.707 | 4.201 | 4.360 | 4.387 | 4.475 | 4.413 | 4.132 |
| | $^1A_1$ $(\pi \to \pi^\star)$ | 4.897 | 4.895 | 4.884 | 4.572 | 4.719 | 5.043 | 4.884 | 4.970 | 5.008 | 5.077 | 5.069 | 5.077 |
| | $^1A_2$ $(n \to \pi^\star)$ | 4.665 | 4.641 | 4.817 | 4.391 | 4.608 | 5.214 | 4.793 | 4.925 | 4.949 | 5.023 | 4.950 | 4.666 |
| | $^1B_2$ $(\pi \to \pi^\star)$ | 4.770 | 4.759 | 4.797 | 4.425 | 4.604 | 5.043 | 4.794 | 4.906 | 4.956 | 5.052 | 5.047 | 4.943 |
| | $^1B_2$ $(\pi \to \pi^\star)$ | 5.888 | 5.879 | 5.957 | 5.542 | 5.724 | 6.206 | 5.956 | 6.033 | 6.115 | 6.199 | 6.209 | 6.096 |
| | $^1A_2$ $(n \to \pi^\star)$ | 5.738 | 5.734 | 6.255 | 5.168 | 5.623 | 7.360 | 6.219 | 6.602 | 6.694 | 6.892 | 6.863 | 6.642 |
| | $^1A_1$ $(\pi \to \pi^\star)$ | 6.293 | 6.276 | 6.251 | 5.936 | 6.087 | 6.482 | 6.267 | 6.301 | 6.401 | 6.489 | 6.491 | 6.370 |
| | $^3B_2$ $(\pi \to \pi^\star)$ | 3.531 | 3.524 | 3.193 | 3.441 | 3.271 | 2.167 | 3.333 | 3.537 | 3.178 | 3.049 | 2.780 | 3.361 |
| | $^3B_1$ $(n \to \pi^\star)$ | 3.696 | 3.675 | 3.770 | 3.362 | 3.560 | 4.145 | 3.775 | 4.014 | 3.940 | 4.029 | 3.888 | 3.766 |
| | $^3A_1$ $(\pi \to \pi^\star)$ | 4.145 | 4.134 | 4.068 | 3.886 | 3.945 | 4.113 | 4.109 | 4.251 | 4.204 | 4.264 | 4.189 | 4.258 |
| | $^3B_2$ $(\pi \to \pi^\star)$ | 4.281 | 4.268 | 4.201 | 3.998 | 4.072 | 4.279 | 4.237 | 4.401 | 4.354 | 4.445 | 4.329 | 4.379 |
| | $^3A_2$ $(n \to \pi^\star)$ | 4.312 | 4.290 | 4.336 | 3.986 | 4.159 | 4.635 | 4.347 | 4.565 | 4.484 | 4.560 | 4.405 | 4.283 |
| | $^3B_2$ $(\pi \to \pi^\star)$ | 4.532 | 4.517 | 4.398 | 4.327 | 4.314 | 4.399 | 4.456 | 4.582 | 4.513 | 4.560 | 4.470 | 4.555 |
| Tolan | $^1B_{2u}$ $(\pi \to \pi^\star)$ | 4.948 | 4.945 | 5.008 | 4.720 | 4.800 | 5.166 | 5.048 | 5.087 | 5.152 | 5.206 | 5.207 | 5.204 |
| | $^1B_{3g}$ $(\pi \to \pi^\star)$ | 4.979 | 4.977 | 5.043 | 4.766 | 4.839 | 5.191 | 5.078 | 5.123 | 5.178 | 5.229 | 5.228 | 5.241 |
| | $^1B_{1u}$ $(\pi \to \pi^\star)$ | 4.307 | 4.294 | 4.413 | 4.221 | 4.240 | 4.541 | 4.458 | 4.504 | 4.573 | 4.634 | 4.664 | 4.604 |
| | $^1A_u$ $(\pi \to \pi^\star)$ | 4.933 | 4.909 | 5.128 | 4.800 | 4.915 | 5.385 | 5.126 | 5.199 | 5.304 | 5.391 | 5.368 | 5.027 |
| | $^1B_{3u}$ (Ryd) | 5.868 | 5.860 | 5.562 | 5.057 | 5.279 | 5.823 | 5.801 | 5.360 | 6.105 | 6.255 | 6.276 | 5.162 |
| | $^3B_{1u}$ $(\pi \to \pi^\star)$ | 2.904 | 2.894 | 2.662 | 2.866 | 2.708 | 1.641 | 2.790 | 2.995 | 2.672 | 2.561 | 2.289 | 2.811 |
| | $^3A_g$ $(\pi \to \pi^\star)$ | 3.920 | 3.913 | 3.529 | 3.869 | 3.635 | 2.461 | 3.689 | 3.884 | 3.502 | 3.356 | 3.072 | 3.694 |

Table S11: VTEs (in eV) computed with TD-DFT using the aug-cc-pVTZ basis set.

| Compound | State | B2PLYP | PBE0-DH | PBE-QIDH | ωB2PLYP | RSH-0DH | RSX-QIDH | ωB97X-2 | SOS-ωB88PP86 | SOS-ωPBEPP86 | cLH12ct-SsirPW92 | cLH14t-calPBE | cLH20t |
|---|---|---|---|---|---|---|---|---|---|---|---|---|---|
| Anthracene | $^1B_{1u}$ ($\pi \to \pi^\star$) | 3.397 | 3.464 | 3.578 | 3.701 | 3.772 | 3.743 | 3.612 | 3.565 | 3.525 | 3.376 | 3.269 | 3.374 |
| | $^1B_{2u}$ ($\pi \to \pi^\star$) | 3.785 | 3.985 | 3.902 | 3.977 | 4.152 | 4.005 | 3.288 | 3.574 | 3.472 | 4.030 | 3.932 | 3.992 |
| | $^1B_{3g}$ ($\pi \to \pi^\star$) | 4.751 | 5.064 | 5.199 | 5.293 | 5.413 | 5.366 | 4.500 | 5.153 | 5.123 | 5.048 | 4.917 | 5.015 |
| | $^1B_{2g}$ (Ryd) | 4.816 | 5.150 | 5.219 | 5.228 | 5.677 | 5.496 | 5.190 | 5.316 | 5.397 | 5.424 | 5.171 | 4.999 |
| | $^1B_{1u}$ ($\pi \to \pi^\star$) | 5.158 | 5.390 | 5.508 | 5.568 | 5.870 | 5.759 | 5.399 | 5.547 | 5.563 | 5.398 | 5.175 | 5.249 |
| | $^1B_{3g}$ ($\pi \to \pi^\star$) | 4.988 | 5.150 | 5.205 | 5.711 | 6.062 | 5.789 | 5.107 | 5.359 | 5.284 | 4.881 | 4.648 | 4.899 |
| | $^1A_g$ ($\pi \to \pi^\star$) | 5.474 | 5.755 | 5.709 | 5.877 | 6.148 | 5.944 | 4.930 | 5.465 | 5.376 | 5.769 | 5.617 | 5.722 |
| | $^1B_{3u}$ (Ryd) | 5.065 | 5.397 | 5.482 | 5.553 | 5.984 | 5.795 | 5.495 | 5.635 | 5.721 | 5.718 | 5.467 | 5.287 |
| | $^1A_u$ (Ryd) | 5.091 | 5.436 | 5.539 | 5.639 | 6.075 | 5.880 | 5.556 | 5.707 | 5.786 | 5.712 | 5.460 | 5.315 |
| | $^1B_{2u}$ ($\pi \to \pi^\star$) | 5.199 | 5.352 | 5.371 | 5.470 | 5.615 | 5.528 | 5.018 | 5.325 | 5.289 | 5.332 | 5.236 | 5.302 |
| | $^3B_{1u}$ ($\pi \to \pi^\star$) | | | | | | | | | | 2.115 | 1.856 | 2.060 |
| | $^3B_{3g}$ ($\pi \to \pi^\star$) | | | | | | | | | | 3.621 | 3.342 | 3.553 |
| | $^3B_{2u}$ ($\pi \to \pi^\star$) | | | | | | | | | | 3.703 | 3.553 | 3.677 |
| Anthraquinone | $^1B_{1g}$ ($n \to \pi^\star$) | 3.043 | 3.240 | 3.309 | 3.454 | 3.619 | 3.523 | 2.521 | 3.257 | 3.214 | 3.065 | 2.962 | 3.134 |
| | $^1A_u$ ($n \to \pi^\star$) | 3.297 | 3.505 | 3.551 | 3.680 | 3.852 | 3.749 | 2.757 | 3.472 | 3.427 | 3.399 | 3.286 | 3.455 |
| | $^1A_g$ ($\pi \to \pi^\star$) | 4.005 | 4.252 | 4.290 | 4.505 | 4.745 | 4.558 | 3.633 | 4.125 | 4.038 | 4.117 | 3.941 | 4.118 |
| | $^1B_{2u}$ ($\pi \to \pi^\star$) | 4.042 | 4.270 | 4.314 | 4.501 | 4.726 | 4.557 | 3.685 | 4.118 | 4.031 | 4.115 | 3.943 | 4.118 |
| | $^1B_{3g}$ ($\pi \to \pi^\star$) | 4.034 | 4.151 | 4.343 | 4.499 | 4.624 | 4.592 | 4.289 | 4.325 | 4.288 | 3.932 | 3.778 | 3.943 |
| | $^1B_{1u}$ ($\pi \to \pi^\star$) | 4.815 | 4.941 | 5.092 | 5.219 | 5.322 | 5.283 | 5.085 | 5.033 | 4.991 | 4.778 | 4.610 | 4.774 |
| | $^1B_{2u}$ ($\pi \to \pi^\star$) | 5.169 | 5.404 | 5.482 | 5.692 | 5.918 | 5.780 | 4.943 | 5.431 | 5.379 | 5.295 | 5.122 | 5.281 |
| | $^3B_{1g}$ ($n \to \pi^\star$) | | | | | | | | | | 2.730 | 2.528 | 2.783 |
| | $^3A_u$ ($n \to \pi^\star$) | | | | | | | | | | 3.047 | 2.830 | 3.085 |
| | $^3B_{1u}$ ($\pi \to \pi^\star$) | | | | | | | | | | 3.214 | 2.940 | 3.126 |
| | $^3B_{3g}$ ($\pi \to \pi^\star$) | | | | | | | | | | 3.293 | 3.034 | 3.251 |
| | $^3A_g$ ($\pi \to \pi^\star$) | | | | | | | | | | 3.341 | 3.139 | 3.307 |
| Aza-BODIPY | $^1B_2$ ($\pi \to \pi^\star$) | 2.746 | 2.815 | 2.739 | 2.659 | 2.699 | 2.670 | 2.511 | 2.479 | 2.418 | 2.884 | 2.861 | 2.862 |
| | $^1B_2$ ($\pi \to \pi^\star$) | 3.350 | 3.568 | 3.580 | 3.766 | 3.988 | 3.830 | 2.897 | 3.486 | 3.420 | 3.509 | 3.406 | 3.514 |
| | $^1A_1$ ($\pi \to \pi^\star$) | 3.477 | 3.744 | 3.767 | 4.009 | 4.263 | 4.077 | 2.980 | 3.675 | 3.602 | 3.666 | 3.531 | 3.687 |
| | $^1B_1$ ($n \to \pi^\star$) | 3.728 | 3.864 | 3.949 | 3.994 | 4.105 | 4.078 | 3.389 | 3.876 | 3.852 | 3.805 | 3.706 | 3.843 |
| | $^3B_2$ ($\pi \to \pi^\star$) | | | | | | | | | | 1.088 | 1.011 | 1.019 |
| | $^3B_2$ ($\pi \to \pi^\star$) | | | | | | | | | | 2.673 | 2.479 | 2.658 |
| | $^3A_1$ ($\pi \to \pi^\star$) | | | | | | | | | | 2.916 | 2.716 | 2.905 |
| | $^3B_1$ ($n \to \pi^\star$) | | | | | | | | | | 3.327 | 3.119 | 3.341 |
| Azobenzene | $^1B_g$ ($n \to \pi^\star$) | 2.742 | 2.782 | 2.848 | 2.886 | 2.911 | 2.911 | 2.591 | 2.787 | 2.756 | 2.773 | 2.714 | 2.827 |
| | $^1B_u$ ($\pi \to \pi^\star$) | 3.898 | 4.000 | 4.136 | 4.234 | 4.344 | 4.321 | 4.132 | 4.124 | 4.096 | 3.889 | 3.774 | 3.888 |
| | $^1A_g$ ($\pi \to \pi^\star$) | 4.255 | 4.528 | 4.582 | 4.799 | 5.054 | 4.862 | 3.869 | 4.371 | 4.281 | 4.373 | 4.170 | 4.390 |
| | $^1B_u$ ($\pi \to \pi^\star$) | 4.241 | 4.516 | 4.569 | 4.786 | 5.040 | 4.851 | 3.873 | 4.360 | 4.271 | 4.367 | 4.167 | 4.383 |
| | $^1A_g$ ($\pi \to \pi^\star$) | 5.026 | 5.219 | 5.435 | 5.603 | 5.737 | 5.706 | 5.465 | 5.412 | 5.382 | 5.068 | 4.872 | 5.075 |
| | $^3B_g$ ($n \to \pi^\star$) | | | | | | | | | | 2.146 | 1.942 | 2.167 |
| | $^3B_u$ ($\pi \to \pi^\star$) | | | | | | | | | | 2.537 | 2.284 | 2.478 |
| | $^3A_g$ ($\pi \to \pi^\star$) | | | | | | | | | | 3.815 | 3.525 | 3.770 |
| | $^3B_u$ ($\pi \to \pi^\star$) | | | | | | | | | | 3.893 | 3.666 | 3.891 |
| | $^3A_g$ ($\pi \to \pi^\star$) | | | | | | | | | | 3.979 | 3.738 | 3.961 |
| BODIPY | $^1B_2$ ($\pi \to \pi^\star$) | 2.985 | 3.095 | 3.009 | 2.981 | 3.062 | 2.998 | 2.664 | 2.755 | 2.688 | 3.178 | 3.148 | 3.152 |
| | $^1B_2$ ($\pi \to \pi^\star$) | 3.679 | 3.917 | 3.948 | 4.160 | 4.399 | 4.230 | 3.249 | 3.870 | 3.807 | 3.847 | 3.718 | 3.851 |
| | $^1A_1$ ($\pi \to \pi^\star$) | 3.833 | 4.110 | 4.146 | 4.403 | 4.667 | 4.475 | 3.362 | 4.069 | 4.001 | 4.032 | 3.878 | 4.045 |
| | $^3B_2$ ($\pi \to \pi^\star$) | | | | | | | | | | 1.683 | 1.584 | 1.635 |
| | $^3B_2$ ($\pi \to \pi^\star$) | | | | | | | | | | 3.014 | 2.806 | 2.990 |
| | $^3A_1$ ($\pi \to \pi^\star$) | | | | | | | | | | 3.230 | 3.015 | 3.210 |
| Coumarin | $^1A'$ ($\pi \to \pi^\star$) | 4.246 | 4.418 | 4.483 | 4.565 | 4.718 | 4.647 | 4.129 | 4.341 | 4.300 | 4.386 | 4.256 | 4.370 |
| | $^1A''$ ($n \to \pi^\star$) | 4.574 | 4.852 | 4.950 | 5.111 | 5.338 | 5.219 | 4.045 | 4.863 | 4.823 | 4.766 | 4.570 | 4.813 |
| | $^1A'$ ($\pi \to \pi^\star$) | 4.733 | 4.924 | 4.926 | 5.040 | 5.230 | 5.088 | 4.417 | 4.708 | 4.626 | 4.866 | 4.718 | 4.845 |
| | $^3A'$ ($\pi \to \pi^\star$) | | | | | | | | | | 3.122 | 2.859 | 3.055 |
| | $^3A'$ ($\pi \to \pi^\star$) | | | | | | | | | | 3.904 | 3.653 | 3.864 |
| | $^3A''$ ($n \to \pi^\star$) | | | | | | | | | | 4.476 | 4.206 | 4.500 |
| Cyclazine | $^1A'_2$ ($\pi \to \pi^\star$) | 1.124 | 1.246 | 1.184 | 1.218 | 1.335 | 1.246 | 0.732 | 0.973 | 0.893 | 1.279 | 1.246 | 1.262 |
| | $^1E'$ ($\pi \to \pi^\star$) | 3.054 | 3.254 | 3.204 | 3.300 | 3.501 | 3.352 | 2.651 | 3.106 | 3.047 | 3.295 | 3.197 | 3.246 |
| | $^1A''_1$ (Ryd) | 3.150 | 3.469 | 3.496 | 3.461 | 3.900 | 3.727 | 3.374 | 3.564 | 3.635 | 3.740 | 3.532 | 3.352 |
| | $^1E''$ (Ryd) | 3.571 | 3.892 | 3.945 | 3.995 | 4.400 | 4.222 | 3.926 | 4.080 | 4.161 | 4.187 | 4.000 | 3.801 |
| | $^3A'_2$ ($\pi \to \pi^\star$) | | | | | | | | | | 1.114 | 1.036 | 1.083 |
| | $^3E'$ ($\pi \to \pi^\star$) | | | | | | | | | | 2.192 | 2.028 | 2.127 |
| | $^3A''_1$ (Ryd) | | | | | | | | | | 3.824 | 3.524 | 3.367 |
| | $^3E''$ (Ryd) | | | | | | | | | | 4.276 | 3.997 | 3.822 |

Table S12: VTEs (in eV) computed with TD-DFT using the aug-cc-pVTZ basis set.

| Compound | State | B2PLYP | PBE0-DH | PBE-QIDH | $\omega$B2PLYP | RSH-0DH | RSX-QIDH | $\omega$B97X-2 | SOS-$\omega$B88PP86 | SOS-$\omega$PBEPP86 | cLH12ct-SsirPW92 | cLH14t-calPBE | cLH20t |
|---|---|---|---|---|---|---|---|---|---|---|---|---|---|
| Heptazine | $^1A_2'$ $(\pi \to \pi^\star)$ | 2.763 | 3.087 | 3.002 | 3.121 | 3.421 | 3.219 | 1.865 | 2.753 | 2.663 | 3.136 | 3.004 | 3.097 |
| | $^1A_1''$ $(n \to \pi^\star)$ | 3.766 | 4.215 | 4.258 | 4.399 | 4.785 | 4.591 | 2.602 | 4.077 | 4.034 | 4.204 | 3.948 | 4.272 |
| | $^1E''$ $(n \to \pi^\star)$ | 3.850 | 4.243 | 4.276 | 4.432 | 4.771 | 4.588 | 2.742 | 4.116 | 4.066 | 4.243 | 4.012 | 4.296 |
| | $^1E'$ $(\pi \to \pi^\star)$ | 4.433 | 4.785 | 4.716 | 4.887 | 5.209 | 4.976 | 3.582 | 4.560 | 4.481 | 4.803 | 4.631 | 4.756 |
| | $^3A_2'$ $(\pi \to \pi^\star)$ | | | | | | | | | | 2.949 | 2.779 | 2.898 |
| | $^3E''(\pi \to \pi^\star)$ | | | | | | | | | | 3.644 | 3.430 | 3.558 |
| | $^3A_1''$ $(n \to \pi^\star)$ | | | | | | | | | | 4.109 | 3.824 | 4.166 |
| | $^3E''$ $(n \to \pi^\star)$ | | | | | | | | | | 4.136 | 3.869 | 4.181 |
| Naphthalimide | $^1B_2$ $(\pi \to \pi^\star)$ | 4.037 | 4.256 | 4.193 | 4.289 | 4.484 | 4.326 | 3.530 | 3.886 | 3.791 | 4.257 | 4.140 | 4.229 |
| | $^1B_1$ $(n \to \pi^\star)$ | 3.874 | 4.208 | 4.326 | 4.542 | 4.811 | 4.662 | 3.221 | 4.277 | 4.235 | 4.055 | 3.837 | 4.135 |
| | $^1A_1$ $(\pi \to \pi^\star)$ | 3.898 | 4.014 | 4.113 | 4.227 | 4.338 | 4.288 | 4.009 | 4.052 | 4.008 | 3.924 | 3.804 | 3.914 |
| | $^1A_2$ $(n \to \pi^\star)$ | 4.393 | 4.678 | 4.767 | 4.923 | 5.160 | 5.037 | 3.740 | 4.680 | 4.639 | 4.526 | 4.341 | 4.589 |
| | $^3A_1$ $(\pi \to \pi^\star)$ | | | | | | | | | | 2.645 | 2.394 | 2.588 |
| | $^3B_2$ $(\pi \to \pi^\star)$ | | | | | | | | | | 3.617 | 3.433 | 3.578 |
| | $^3B_1$ $(n \to \pi^\star)$ | | | | | | | | | | 3.829 | 3.554 | 3.889 |
| | $^3B_2$ $(\pi \to \pi^\star)$ | | | | | | | | | | 4.061 | 3.816 | 3.988 |
| | $^3A_2$ $(n \to \pi^\star)$ | | | | | | | | | | 4.272 | 4.021 | 4.314 |
| Naphthoquinone | $^1B_1$ $(n \to \pi^\star)$ | 2.840 | 3.011 | 3.106 | 3.259 | 3.403 | 3.322 | 2.401 | 3.077 | 3.038 | 2.846 | 2.742 | 2.928 |
| | $^1A_2$ $(n \to \pi^\star)$ | 3.053 | 3.254 | 3.331 | 3.482 | 3.650 | 3.551 | 2.598 | 3.281 | 3.239 | 3.139 | 3.014 | 3.207 |
| | $^1A_1$ $(\pi \to \pi^\star)$ | 3.829 | 4.066 | 4.153 | 4.388 | 4.631 | 4.451 | 3.532 | 4.035 | 3.955 | 3.874 | 3.689 | 3.892 |
| | $^1B_2$ $(\pi \to \pi^\star)$ | 3.954 | 4.067 | 4.281 | 4.439 | 4.570 | 4.540 | 4.196 | 4.296 | 4.267 | 3.824 | 3.664 | 3.845 |
| | $^1A_2$ $(n \to \pi^\star)$ | 4.890 | 5.529 | 5.949 | 6.379 | 6.823 | 6.492 | 3.899 | 6.089 | 5.989 | 5.293 | 5.004 | 5.430 |
| | $^1A_1$ $(\pi \to \pi^\star)$ | 5.328 | 5.593 | 5.603 | 5.786 | 6.034 | 5.874 | 4.942 | 5.457 | 5.395 | 5.582 | 5.429 | 5.543 |
| | $^1B_2$ $(\pi \to \pi^\star)$ | 5.136 | 5.267 | 5.419 | 5.538 | 5.663 | 5.618 | 5.271 | 5.404 | 5.376 | 5.118 | 4.964 | 5.110 |
| | $^3B_1$ $(n \to \pi^\star)$ | | | | | | | | | | 2.483 | 2.270 | 2.548 |
| | $^3A_2$ $(n \to \pi^\star)$ | | | | | | | | | | 2.767 | 2.531 | 2.815 |
| | $^3B_2$ $(\pi \to \pi^\star)$ | | | | | | | | | | 2.986 | 2.699 | 2.892 |
| | $^3B_2$ $(\pi \to \pi^\star)$ | | | | | | | | | | 3.146 | 2.887 | 3.117 |
| | $^3A_1$ $(\pi \to \pi^\star)$ | | | | | | | | | | 3.264 | 3.060 | 3.254 |
| Phenazine | $^1B_{1u}$ $(n \to \pi^\star)$ | 3.229 | 3.387 | 3.479 | 3.641 | 3.778 | 3.694 | 2.753 | 3.457 | 3.419 | 3.260 | 3.162 | 3.326 |
| | $^1B_{3u}$ $(\pi \to \pi^\star)$ | 3.385 | 3.470 | 3.605 | 3.762 | 3.851 | 3.813 | 3.621 | 3.594 | 3.548 | 3.346 | 3.226 | 3.348 |
| | $^1B_{2u}$ $(\pi \to \pi^\star)$ | 3.772 | 3.949 | 3.873 | 3.926 | 4.074 | 3.950 | 3.344 | 3.546 | 3.450 | 3.990 | 3.906 | 3.962 |
| | $^1B_{1g}$ $(\pi \to \pi^\star)$ | 4.280 | 4.463 | 4.613 | 4.880 | 5.050 | 4.947 | 4.361 | 4.626 | 4.575 | 4.293 | 4.125 | 4.309 |
| | $^1B_{2g}$ $(n \to \pi^\star)$ | 4.856 | 5.090 | 5.222 | 5.353 | 5.553 | 5.470 | 4.530 | 5.163 | 5.138 | 5.060 | 4.869 | 5.110 |
| | $^1A_u$ $(\pi \to \pi^\star)$ | 4.888 | 5.304 | 5.324 | 5.598 | 5.955 | 5.911 | 3.628 | 5.257 | 5.203 | 5.217 | 5.014 | 5.276 |
| | $^3B_{3u}$ $(\pi \to \pi^\star)$ | | | | | | | | | | 2.172 | 1.930 | 2.108 |
| | $^3B_{1u}$ $(n \to \pi^\star)$ | | | | | | | | | | 2.876 | 2.688 | 2.921 |
| | $^3B_{2u}$ $(\pi \to \pi^\star)$ | | | | | | | | | | 3.185 | 3.064 | 3.163 |
| | $^3B_{1g}$ $(\pi \to \pi^\star)$ | | | | | | | | | | 3.434 | 3.181 | 3.391 |
| Phthalimide | $^1B_1$ $(n \to \pi^\star)$ | 3.913 | 4.155 | 4.238 | 4.394 | 4.602 | 4.489 | 3.335 | 4.167 | 4.124 | 4.050 | 3.886 | 4.086 |
| | $^1A_1$ $(\pi \to \pi^\star)$ | 4.608 | 4.841 | 4.796 | 4.891 | 5.109 | 4.945 | 4.087 | 4.466 | 4.373 | 4.808 | 4.666 | 4.773 |
| | $^1A_2$ $(n \to \pi^\star)$ | 4.564 | 4.778 | 4.853 | 4.969 | 5.150 | 5.062 | 4.049 | 4.756 | 4.714 | 4.688 | 4.533 | 4.715 |
| | $^1B_2$ $(\pi \to \pi^\star)$ | 4.761 | 4.864 | 5.052 | 5.093 | 5.196 | 5.214 | 4.985 | 4.944 | 4.923 | 4.699 | 4.546 | 4.683 |
| | $^1B_2$ $(\pi \to \pi^\star)$ | 5.677 | 5.912 | 5.992 | 6.099 | 6.314 | 6.202 | 5.325 | 5.872 | 5.838 | 5.840 | 5.652 | 5.808 |
| | $^1A_2$ $(n \to \pi^\star)$ | 5.376 | 5.980 | 6.339 | 6.816 | 7.210 | 7.061 | 5.016 | 6.548 | 6.568 | 5.727 | 5.393 | 5.855 |
| | $^1A_1$ $(\pi \to \pi^\star)$ | 6.066 | 6.262 | 6.301 | 6.388 | 6.579 | 6.479 | 5.807 | 6.196 | 6.159 | 6.220 | 6.077 | 6.177 |
| | $^3B_2$ $(\pi \to \pi^\star)$ | | | | | | | | | | 3.673 | 3.352 | 3.593 |
| | $^3B_1$ $(n \to \pi^\star)$ | | | | | | | | | | 3.735 | 3.480 | 3.755 |
| | $^3A_1$ $(\pi \to \pi^\star)$ | | | | | | | | | | 4.111 | 3.913 | 4.066 |
| | $^3B_2$ $(\pi \to \pi^\star)$ | | | | | | | | | | 4.299 | 4.035 | 4.213 |
| | $^3A_2$ $(n \to \pi^\star)$ | | | | | | | | | | 4.354 | 4.105 | 4.364 |
| | $^3B_2$ $(\pi \to \pi^\star)$ | | | | | | | | | | 4.579 | 4.334 | 4.553 |
| Tolan | $^1B_{2u}$ $(\pi \to \pi^\star)$ | 4.694 | 4.932 | 4.904 | 5.013 | 5.237 | 5.071 | 4.237 | 4.590 | 4.499 | 4.901 | 4.736 | 4.874 |
| | $^1B_{3g}$ $(\pi \to \pi^\star)$ | 4.723 | 4.963 | 4.928 | 5.039 | 5.260 | 5.093 | 4.242 | 4.601 | 4.508 | 4.933 | 4.770 | 4.910 |
| | $^1B_{1u}$ $(\pi \to \pi^\star)$ | 4.405 | 4.431 | 4.603 | 4.670 | 4.706 | 4.742 | 4.483 | 4.593 | 4.572 | 4.316 | 4.207 | 4.308 |
| | $^1A_u$ $(\pi \to \pi^\star)$ | 5.143 | 5.150 | 5.351 | 5.440 | 5.443 | 5.484 | 5.521 | 5.419 | 5.407 | 4.966 | 4.850 | 4.991 |
| | $^1B_{3u}$ (Ryd) | 5.337 | 5.674 | 5.789 | 5.794 | 6.264 | 6.094 | 5.700 | 5.878 | 5.963 | 5.933 | 5.635 | 5.502 |
| | $^3B_{1u}$ $(\pi \to \pi^\star)$ | | | | | | | | | | 3.050 | 2.761 | 2.998 |
| | $^3A_g$ $(\pi \to \pi^\star)$ | | | | | | | | | | 4.121 | 3.748 | 4.014 |

### S3.3 Tamm-Dancoff approximation

Table S13: VTEs (in eV) computed with TDA-DFT using the aug-cc-pVTZ basis set.

| Compound | State | TPSSh | τ-HCTHHyb | B3LYP | PBE0 | cSCAN0 | M06 | cM06 | SOGGA11-X | BMK | MN15 | M08-HX | M06-2X | cM06-2X |
|---|---|---|---|---|---|---|---|---|---|---|---|---|---|---|
| Anthracene | $^1B_{1u}$ ($\pi \rightarrow \pi^\star$) | 3.346 | 3.352 | 3.413 | 3.498 | 3.501 | 3.410 | 3.427 | 3.680 | 3.730 | 3.630 | 3.793 | 3.795 | 3.820 |
| | $^1B_{2u}$ ($\pi \rightarrow \pi^\star$) | 3.861 | 3.860 | 3.896 | 3.977 | 4.078 | 3.863 | 3.865 | 4.143 | 4.147 | 4.025 | 4.164 | 4.155 | 4.157 |
| | $^1B_{3g}$ ($\pi \rightarrow \pi^\star$) | 4.967 | 4.953 | 5.003 | 5.118 | 5.158 | 4.948 | 4.979 | 5.323 | 5.377 | 5.237 | 5.397 | 5.411 | 5.444 |
| | $^1B_{2g}$ (Ryd) | 4.737 | 4.890 | 4.683 | 4.935 | 5.278 | 3.965 | 4.016 | 4.871 | 5.243 | 5.596 | 4.486 | 4.970 | 5.018 |
| | $^1B_{1u}$ ($\pi \rightarrow \pi^\star$) | 4.963 | 4.988 | 4.985 | 5.169 | 5.363 | 4.650 | 4.736 | 5.350 | 5.549 | 5.468 | 5.041 | 5.391 | 5.439 |
| | $^1B_{3g}$ ($\pi \rightarrow \pi^\star$) | 4.340 | 4.390 | 4.511 | 4.690 | 4.849 | 4.608 | 4.621 | 5.138 | 5.166 | 5.050 | 5.236 | 5.304 | 5.320 |
| | $^1A_g$ ($\pi \rightarrow \pi^\star$) | 5.497 | 5.495 | 5.545 | 5.670 | 5.827 | 5.501 | 5.506 | 5.922 | 5.930 | 5.771 | 5.944 | 5.942 | 5.947 |
| | $^1B_{3u}$ (Ryd) | 4.965 | 5.127 | 4.919 | 5.168 | 5.540 | 4.149 | 4.182 | 5.086 | 5.457 | 5.889 | 4.714 | 5.215 | 5.242 |
| | $^1A_u$ (Ryd) | 4.927 | 5.100 | 4.895 | 5.168 | 5.550 | 4.177 | 4.214 | 5.124 | 5.481 | 5.901 | 4.794 | 5.289 | 5.322 |
| | $^1B_{2u}$ ($\pi \rightarrow \pi^\star$) | 5.562 | 5.543 | 5.561 | 5.654 | 5.735 | 5.455 | 5.515 | 5.794 | 5.822 | 5.621 | 5.739 | 5.776 | 5.827 |
| | $^3B_{1u}$ ($\pi \rightarrow \pi^\star$) | 2.057 | 2.091 | 2.107 | 2.084 | 1.628 | 2.099 | 2.117 | 2.246 | 2.311 | 2.212 | 2.406 | 2.409 | 2.437 |
| | $^3B_{3g}$ ($\pi \rightarrow \pi^\star$) | 3.476 | 3.506 | 3.508 | 3.484 | 2.964 | 3.464 | 3.495 | 3.674 | 3.750 | 3.599 | 3.818 | 3.821 | 3.868 |
| | $^3B_{2u}$ ($\pi \rightarrow \pi^\star$) | 3.520 | 3.523 | 3.548 | 3.580 | 3.420 | 3.517 | 3.554 | 3.758 | 3.788 | 3.638 | 3.807 | 3.801 | 3.858 |
| Anthraquinone | $^1B_{1g}$ ($n \rightarrow \pi^\star$) | 2.778 | 2.829 | 2.958 | 3.029 | 3.134 | 3.062 | 3.073 | 3.397 | 3.230 | 3.062 | 3.296 | 3.257 | 3.437 |
| | $^1A_u$ ($n \rightarrow \pi^\star$) | 3.087 | 3.133 | 3.252 | 3.330 | 3.421 | 3.354 | 3.362 | 3.673 | 3.517 | 3.327 | 3.561 | 3.525 | 3.722 |
| | $^1A_g$ ($\pi \rightarrow \pi^\star$) | 3.815 | 3.859 | 3.955 | 4.101 | 4.214 | 4.055 | 4.060 | 4.435 | 4.448 | 4.343 | 4.588 | 4.582 | 4.588 |
| | $^1B_{2u}$ ($\pi \rightarrow \pi^\star$) | 3.787 | 3.824 | 3.920 | 4.067 | 4.179 | 4.005 | 4.009 | 4.402 | 4.414 | 4.315 | 4.558 | 4.550 | 4.555 |
| | $^1B_{3g}$ ($\pi \rightarrow \pi^\star$) | 3.661 | 3.681 | 3.768 | 3.906 | 3.978 | 3.841 | 3.857 | 4.211 | 4.230 | 4.124 | 4.390 | 4.374 | 4.401 |
| | $^1B_{1u}$ ($\pi \rightarrow \pi^\star$) | 4.556 | 4.604 | 4.706 | 4.854 | 4.959 | 4.788 | 4.801 | 5.160 | 5.193 | 5.092 | 5.296 | 5.292 | 5.312 |
| | $^1B_{2u}$ ($\pi \rightarrow \pi^\star$) | 5.001 | 5.029 | 5.113 | 5.259 | 5.400 | 5.159 | 5.177 | 5.587 | 5.596 | 5.441 | 5.664 | 5.672 | 5.696 |
| | $^3B_{1g}$ ($n \rightarrow \pi^\star$) | 2.378 | 2.456 | 2.557 | 2.577 | 2.621 | 2.765 | 2.775 | 2.960 | 2.798 | 2.803 | 2.960 | 2.883 | 3.073 |
| | $^3A_u$ ($n \rightarrow \pi^\star$) | 2.676 | 2.750 | 2.835 | 2.860 | 2.896 | 3.045 | 3.053 | 3.224 | 3.069 | 3.052 | 3.211 | 3.134 | 3.340 |
| | $^3B_{1u}$ ($\pi \rightarrow \pi^\star$) | 3.113 | 3.163 | 3.177 | 3.174 | 2.721 | 3.255 | 3.278 | 3.376 | 3.427 | 3.333 | 3.575 | 3.532 | 3.573 |
| | $^3B_{3g}$ ($\pi \rightarrow \pi^\star$) | 3.090 | 3.120 | 3.162 | 3.197 | 2.724 | 3.187 | 3.206 | 3.435 | 3.493 | 3.373 | 3.656 | 3.624 | 3.655 |
| | $^3A_g$ ($\pi \rightarrow \pi^\star$) | 3.072 | 3.112 | 3.168 | 3.240 | 3.169 | 3.275 | 3.291 | 3.499 | 3.538 | 3.462 | 3.696 | 3.653 | 3.685 |
| Aza-BODIPY | $^1B_2$ ($\pi \rightarrow \pi^\star$) | 3.083 | 3.091 | 3.134 | 3.198 | 3.265 | 3.153 | 3.173 | 3.274 | 3.273 | 3.170 | 2.913 | 3.206 | 3.236 |
| | $^1B_2$ ($\pi \rightarrow \pi^\star$) | 3.872 | 3.833 | 3.812 | 3.835 | 3.833 | 3.740 | 3.761 | 3.912 | 3.933 | 3.837 | 3.949 | 3.958 | 3.983 |
| | $^1A_1$ ($\pi \rightarrow \pi^\star$) | 3.457 | 3.491 | 3.575 | 3.687 | 3.794 | 3.653 | 3.667 | 3.993 | 3.991 | 3.893 | 4.062 | 4.086 | 4.110 |
| | $^1B_1$ ($n \rightarrow \pi^\star$) | 3.572 | 3.569 | 3.655 | 3.714 | 3.822 | 3.603 | 3.626 | 4.027 | 3.827 | 3.646 | 3.846 | 3.790 | 3.965 |
| | $^3B_2$ ($\pi \rightarrow \pi^\star$) | 1.327 | 1.323 | 1.284 | 1.222 | 0.973 | 1.227 | 1.239 | 1.200 | 1.262 | 1.219 | 1.262 | 1.215 | 1.237 |
| | $^3B_2$ ($\pi \rightarrow \pi^\star$) | 2.464 | 2.505 | 2.545 | 2.579 | 2.433 | 2.629 | 2.647 | 2.814 | 2.834 | 2.769 | 2.913 | 2.921 | 2.950 |
| | $^3A_1$ ($\pi \rightarrow \pi^\star$) | 2.678 | 2.724 | 2.769 | 2.807 | 2.650 | 2.844 | 2.862 | 3.060 | 3.083 | 3.018 | 3.160 | 3.170 | 3.198 |
| | $^3B_1$ ($n \rightarrow \pi^\star$) | 3.008 | 3.040 | 3.085 | 3.089 | 3.094 | 3.160 | 3.183 | 3.406 | 3.220 | 3.190 | 3.296 | 3.242 | 3.443 |
| Azobenzene | $^1B_g$ ($n \rightarrow \pi^\star$) | 2.610 | 2.603 | 2.679 | 2.701 | 2.716 | 2.588 | 2.623 | 2.929 | 2.767 | 2.611 | 2.756 | 2.678 | 2.904 |
| | $^1B_u$ ($\pi \rightarrow \pi^\star$) | 3.864 | 3.856 | 3.900 | 4.006 | 4.017 | 3.884 | 3.909 | 4.179 | 4.221 | 4.122 | 4.299 | 4.284 | 4.317 |
| | $^1A_g$ ($\pi \rightarrow \pi^\star$) | 3.966 | 4.004 | 4.120 | 4.287 | 4.408 | 4.185 | 4.190 | 4.671 | 4.689 | 4.588 | 4.816 | 4.821 | 4.826 |
| | $^1B_u$ ($\pi \rightarrow \pi^\star$) | 3.980 | 4.010 | 4.118 | 4.281 | 4.403 | 4.178 | 4.184 | 4.658 | 4.677 | 4.575 | 4.800 | 4.806 | 4.811 |
| | $^1A_g$ ($\pi \rightarrow \pi^\star$) | 4.698 | 4.746 | 4.851 | 5.026 | 5.133 | 4.864 | 4.883 | 5.398 | 5.437 | 5.329 | 5.557 | 5.572 | 5.589 |
| | $^3B_g$ ($n \rightarrow \pi^\star$) | 1.902 | 1.953 | 1.964 | 1.912 | 1.795 | 2.034 | 2.070 | 2.156 | 2.016 | 2.052 | 2.113 | 1.997 | 2.252 |
| | $^3B_u$ ($\pi \rightarrow \pi^\star$) | 2.474 | 2.493 | 2.508 | 2.522 | 2.108 | 2.516 | 2.536 | 2.699 | 2.763 | 2.674 | 2.915 | 2.892 | 2.931 |
| | $^3A_g$ ($\pi \rightarrow \pi^\star$) | 3.487 | 3.530 | 3.603 | 3.669 | 3.113 | 3.629 | 3.648 | 3.938 | 4.013 | 3.871 | 4.144 | 4.130 | 4.165 |
| | $^3B_u$ ($\pi \rightarrow \pi^\star$) | 3.500 | 3.543 | 3.627 | 3.728 | 3.621 | 3.675 | 3.692 | 4.064 | 4.110 | 4.014 | 4.244 | 4.234 | 4.263 |
| | $^3A_g$ ($\pi \rightarrow \pi^\star$) | 3.709 | 3.746 | 3.784 | 3.830 | 3.698 | 3.775 | 3.795 | 4.134 | 4.183 | 4.077 | 4.307 | 4.293 | 4.324 |
| BODIPY | $^1B_2$ ($\pi \rightarrow \pi^\star$) | 3.393 | 3.392 | 3.419 | 3.472 | 3.537 | 3.400 | 3.421 | 3.512 | 3.501 | 3.401 | 3.447 | 3.427 | 3.458 |
| | $^1B_2$ ($\pi \rightarrow \pi^\star$) | 3.931 | 3.910 | 3.925 | 3.989 | 4.047 | 3.921 | 3.939 | 4.194 | 4.191 | 4.090 | 4.234 | 4.257 | 4.280 |
| | $^1A_1$ ($\pi \rightarrow \pi^\star$) | 3.779 | 3.815 | 3.904 | 4.027 | 4.159 | 3.995 | 4.008 | 4.360 | 4.343 | 4.240 | 4.408 | 4.442 | 4.463 |
| | $^3B_2$ ($\pi \rightarrow \pi^\star$) | 1.747 | 1.747 | 1.723 | 1.690 | 1.501 | 1.701 | 1.719 | 1.737 | 1.763 | 1.721 | 1.774 | 1.739 | 1.767 |
| | $^3B_2$ ($\pi \rightarrow \pi^\star$) | 2.773 | 2.816 | 2.858 | 2.899 | 2.776 | 2.955 | 2.971 | 3.150 | 3.160 | 3.091 | 3.241 | 3.255 | 3.282 |
| | $^3A_1$ ($\pi \rightarrow \pi^\star$) | 2.970 | 3.018 | 3.065 | 3.106 | 2.953 | 3.153 | 3.170 | 3.371 | 3.385 | 3.314 | 3.462 | 3.479 | 3.507 |
| Coumarin | $^1A'$ ($\pi \rightarrow \pi^\star$) | 4.232 | 4.245 | 4.310 | 4.420 | 4.545 | 4.347 | 4.357 | 4.660 | 4.660 | 4.533 | 4.676 | 4.689 | 4.706 |
| | $^1A''$ ($n \rightarrow \pi^\star$) | 4.234 | 4.299 | 4.456 | 4.584 | 4.750 | 4.600 | 4.611 | 5.053 | 4.904 | 4.659 | 4.934 | 4.942 | 5.112 |
| | $^1A'$ ($\pi \rightarrow \pi^\star$) | 4.725 | 4.726 | 4.780 | 4.900 | 4.956 | 4.776 | 4.799 | 5.122 | 5.162 | 5.011 | 5.207 | 5.203 | 5.231 |
| | $^3A'$ ($\pi \rightarrow \pi^\star$) | 3.007 | 3.034 | 3.039 | 3.028 | 2.627 | 3.068 | 3.097 | 3.209 | 3.257 | 3.139 | 3.328 | 3.312 | 3.359 |
| | $^3A'$ ($\pi \rightarrow \pi^\star$) | 3.626 | 3.667 | 3.712 | 3.753 | 3.485 | 3.758 | 3.778 | 4.671 | 4.065 | 3.959 | 4.160 | 4.157 | 4.189 |
| | $^3A''$ ($n \rightarrow \pi^\star$) | 3.929 | 4.010 | 4.132 | 4.210 | 4.312 | 4.357 | 4.368 | 4.671 | 4.519 | 4.418 | 4.623 | 4.594 | 4.774 |
| Cyclazine | $^1A'_2$ ($\pi \rightarrow \pi^\star$) | 1.299 | 1.269 | 1.267 | 1.298 | 1.376 | 1.271 | 1.302 | 1.368 | 1.360 | 1.242 | 1.363 | 1.324 | 1.362 |
| | $^1E'$ ($\pi \rightarrow \pi^\star$) | 3.320 | 3.315 | 3.318 | 3.404 | 3.519 | 3.245 | 3.284 | 3.518 | 3.571 | 3.465 | 3.430 | 3.516 | 3.545 |
| | $^1A''_1$ (Ryd) | 3.204 | 3.336 | 3.115 | 3.326 | 3.675 | 2.491 | 2.559 | 3.213 | 3.568 | 3.910 | 2.742 | 3.242 | 3.298 |
| | $^1E''$ (Ryd) | 3.559 | 3.726 | 3.494 | 3.718 | 4.111 | 2.768 | 2.830 | 3.573 | 3.898 | 4.389 | 3.138 | 3.662 | 3.707 |
| | $^3A'_2$ ($\pi \rightarrow \pi^\star$) | 1.095 | 1.081 | 1.071 | 1.079 | 1.090 | 1.120 | 1.150 | 1.170 | 1.165 | 1.089 | 1.198 | 1.138 | 1.175 |
| | $^3E'$ ($\pi \rightarrow \pi^\star$) | 2.115 | 2.134 | 2.121 | 2.126 | 2.096 | 2.142 | 2.161 | 2.267 | 2.281 | 2.197 | 2.288 | 2.278 | 2.305 |
| | $^3A''_1$ (Ryd) | 3.193 | 3.307 | 3.109 | 3.301 | 3.640 | 2.449 | 2.517 | 3.275 | 3.541 | 3.879 | 2.793 | 3.235 | 3.290 |
| | $^3E''$ (Ryd) | 3.549 | 3.679 | 3.494 | 3.700 | 4.091 | 2.726 | 2.788 | 3.637 | 3.860 | 4.371 | 3.212 | 3.638 | 3.683 |

Table S14: VTEs (in eV) computed with TDA-DFT using the aug-cc-pVTZ basis set.

| Compound | State | TPSSh | $\tau$-HCTHHyb | B3LYP | PBE0 | cSCAN0 | M06 | cM06 | SOGGA11-X | BMK | MN15 | M08-HX | M06-2X | cM06-2X |
|---|---|---|---|---|---|---|---|---|---|---|---|---|---|---|
| Heptazine | $^1A_2'$ $(\pi \rightarrow \pi^\star)$ | 2.927 | 2.922 | 2.950 | 3.051 | 3.237 | 3.040 | 3.065 | 3.308 | 3.155 | 3.017 | 3.198 | 3.214 | 3.251 |
| | $^1A_1''$ $(n \rightarrow \pi^\star)$ | 3.535 | 3.580 | 3.742 | 3.905 | 4.183 | 3.773 | 3.795 | 4.490 | 4.252 | 4.065 | 4.468 | 4.394 | 4.470 |
| | $^1E''$ $(n \rightarrow \pi^\star)$ | 3.616 | 3.671 | 3.828 | 3.956 | 4.213 | 3.790 | 3.812 | 4.496 | 4.275 | 4.111 | 4.443 | 4.371 | 4.449 |
| | $^1E'$ $(\pi \rightarrow \pi^\star)$ | 4.631 | 4.656 | 4.719 | 4.854 | 5.043 | 4.819 | 4.836 | 5.160 | 5.079 | 4.930 | 5.119 | 5.137 | 5.163 |
| | $^3A_2'$ $(\pi \rightarrow \pi^\star)$ | 2.705 | 2.712 | 2.731 | 2.807 | 2.921 | 2.864 | 2.888 | 3.074 | 2.922 | 2.838 | 3.002 | 2.997 | 3.037 |
| | $^3E''(\pi \rightarrow \pi^\star)$ | 3.413 | 3.442 | 3.457 | 3.517 | 3.591 | 3.589 | 3.609 | 3.780 | 3.671 | 3.600 | 3.755 | 3.745 | 3.781 |
| | $^3A_1''$ $(n \rightarrow \pi^\star)$ | 3.437 | 3.490 | 3.636 | 3.771 | 3.986 | 3.702 | 3.724 | 4.344 | 4.114 | 3.996 | 4.336 | 4.261 | 4.353 |
| | $^3E''$ $(n \rightarrow \pi^\star)$ | 3.493 | 3.563 | 3.703 | 3.807 | 4.010 | 3.709 | 3.731 | 4.352 | 4.135 | 4.048 | 4.326 | 4.249 | 4.336 |
| Naphthalimide | $^1B_2$ $(\pi \rightarrow \pi^\star)$ | 4.077 | 4.086 | 4.134 | 4.234 | 4.347 | 4.127 | 4.131 | 4.438 | 4.434 | 4.314 | 4.469 | 4.463 | 4.468 |
| | $^1B_1$ $(n \rightarrow \pi^\star)$ | 3.424 | 3.533 | 3.724 | 3.867 | 4.046 | 3.889 | 3.893 | 4.413 | 4.271 | 4.080 | 4.379 | 4.370 | 4.518 |
| | $^1A_1$ $(\pi \rightarrow \pi^\star)$ | 3.871 | 3.880 | 3.935 | 4.038 | 4.078 | 3.951 | 3.951 | 4.242 | 4.273 | 4.170 | 4.338 | 4.340 | 4.363 |
| | $^1A_2$ $(n \rightarrow \pi^\star)$ | 3.986 | 4.078 | 4.253 | 4.380 | 4.561 | 4.402 | 4.410 | 4.875 | 4.711 | 4.479 | 4.757 | 4.751 | 4.909 |
| | $^3A_1$ $(\pi \rightarrow \pi^\star)$ | 2.542 | 2.576 | 2.590 | 2.586 | 2.160 | 2.609 | 2.628 | 2.769 | 2.821 | 2.720 | 2.921 | 2.911 | 2.942 |
| | $^3B_2$ $(\pi \rightarrow \pi^\star)$ | 3.405 | 3.431 | 3.458 | 3.498 | 3.299 | 3.477 | 3.499 | 3.703 | 3.733 | 3.633 | 3.810 | 3.787 | 3.820 |
| | $^3B_1$ $(n \rightarrow \pi^\star)$ | 3.197 | 3.316 | 3.474 | 3.574 | 3.708 | 3.699 | 3.705 | 4.100 | 3.951 | 3.886 | 4.119 | 4.073 | 4.233 |
| | $^3B_2$ $(\pi \rightarrow \pi^\star)$ | 3.821 | 3.884 | 3.908 | 3.917 | 3.586 | 3.919 | 3.949 | 4.125 | 4.176 | 4.021 | 4.250 | 4.222 | 4.270 |
| | $^3A_2$ $(n \rightarrow \pi^\star)$ | 3.731 | 3.828 | 3.965 | 4.043 | 4.169 | 4.181 | 4.189 | 4.523 | 4.357 | 4.260 | 4.474 | 4.431 | 4.601 |
| Naphthoquinone | $^1B_1$ $(n \rightarrow \pi^\star)$ | 2.558 | 2.593 | 2.726 | 2.787 | 2.885 | 2.821 | 2.835 | 3.162 | 2.996 | 2.833 | 3.058 | 3.031 | 3.216 |
| | $^1A_2$ $(n \rightarrow \pi^\star)$ | 2.798 | 2.840 | 2.967 | 3.048 | 3.136 | 3.078 | 3.087 | 3.412 | 3.265 | 3.084 | 3.328 | 3.297 | 3.503 |
| | $^1A_1$ $(\pi \rightarrow \pi^\star)$ | 3.540 | 3.577 | 3.682 | 3.838 | 3.956 | 3.799 | 3.804 | 4.208 | 4.218 | 4.127 | 4.389 | 4.388 | 4.393 |
| | $^1B_2$ $(\pi \rightarrow \pi^\star)$ | 3.546 | 3.564 | 3.660 | 3.801 | 3.883 | 3.748 | 3.766 | 4.127 | 4.141 | 4.045 | 4.306 | 4.295 | 4.323 |
| | $^1A_2$ $(n \rightarrow \pi^\star)$ | 4.497 | 4.612 | 4.867 | 5.056 | 5.336 | 5.043 | 5.059 | 5.859 | 5.721 | 5.529 | 5.956 | 5.972 | 6.029 |
| | $^1A_1$ $(\pi \rightarrow \pi^\star)$ | 5.332 | 5.331 | 5.382 | 5.509 | 5.664 | 5.369 | 5.378 | 5.782 | 5.787 | 5.621 | 5.819 | 5.829 | 5.843 |
| | $^1B_2$ $(\pi \rightarrow \pi^\star)$ | 5.032 | 5.050 | 5.135 | 5.266 | 5.387 | 5.197 | 5.216 | 5.559 | 5.579 | 5.469 | 5.660 | 5.654 | 5.684 |
| | $^3B_1$ $(n \rightarrow \pi^\star)$ | 2.116 | 2.186 | 2.292 | 2.304 | 2.335 | 2.500 | 2.513 | 2.699 | 2.540 | 2.556 | 2.702 | 2.637 | 2.834 |
| | $^3A_2$ $(n \rightarrow \pi^\star)$ | 2.357 | 2.433 | 2.528 | 2.556 | 2.579 | 2.752 | 2.761 | 2.940 | 2.795 | 2.787 | 2.954 | 2.886 | 3.100 |
| | $^3B_2$ $(\pi \rightarrow \pi^\star)$ | 2.890 | 2.929 | 2.968 | 2.976 | 2.556 | 3.045 | 3.065 | 3.172 | 3.236 | 3.152 | 3.361 | 3.322 | 3.379 |
| | $^3B_2$ $(\pi \rightarrow \pi^\star)$ | 2.990 | 3.031 | 3.043 | 3.043 | 2.649 | 3.108 | 3.146 | 3.292 | 3.345 | 3.241 | 3.507 | 3.476 | 3.515 |
| | $^3A_1$ $(\pi \rightarrow \pi^\star)$ | 2.944 | 2.983 | 3.058 | 3.155 | 3.107 | 3.170 | 3.183 | 3.457 | 3.492 | 3.424 | 3.675 | 3.641 | 3.667 |
| Phenazine | $^1B_{1u}$ $(n \rightarrow \pi^\star)$ | 2.967 | 3.005 | 3.145 | 3.186 | 3.291 | 3.138 | 3.155 | 3.553 | 3.384 | 3.262 | 3.435 | 3.380 | 3.526 |
| | $^1B_{3u}$ $(\pi \rightarrow \pi^\star)$ | 3.269 | 3.282 | 3.352 | 3.448 | 3.467 | 3.367 | 3.384 | 3.664 | 3.716 | 3.610 | 3.823 | 3.804 | 3.828 |
| | $^1B_{2u}$ $(\pi \rightarrow \pi^\star)$ | 3.906 | 3.904 | 3.940 | 4.017 | 4.098 | 3.903 | 3.907 | 4.167 | 4.182 | 4.056 | 4.210 | 4.189 | 4.194 |
| | $^1B_{1g}$ $(\pi \rightarrow \pi^\star)$ | 3.969 | 4.001 | 4.105 | 4.245 | 4.325 | 4.150 | 4.165 | 4.589 | 4.637 | 4.512 | 4.767 | 4.761 | 4.783 |
| | $^1B_{2g}$ $(n \rightarrow \pi^\star)$ | 4.588 | 4.603 | 4.730 | 4.860 | 4.988 | 4.768 | 4.785 | 5.319 | 5.126 | 4.866 | 5.217 | 5.164 | 5.362 |
| | $^1A_u$ $(\pi \rightarrow \pi^\star)$ | 4.653 | 4.709 | 4.893 | 4.997 | 5.261 | 4.893 | 4.919 | 5.562 | 5.332 | 5.185 | 5.448 | 5.393 | 5.473 |
| | $^3B_{3u}$ $(\pi \rightarrow \pi^\star)$ | 2.121 | 2.154 | 2.172 | 2.167 | 1.768 | 2.193 | 2.210 | 2.325 | 2.397 | 2.312 | 2.539 | 2.517 | 2.545 |
| | $^3B_{1u}$ $(n \rightarrow \pi^\star)$ | 2.521 | 2.587 | 2.688 | 2.683 | 2.690 | 2.784 | 2.803 | 3.044 | 2.893 | 2.913 | 3.009 | 2.941 | 3.112 |
| | $^3B_{2u}$ $(\pi \rightarrow \pi^\star)$ | 3.074 | 3.077 | 3.094 | 3.108 | 2.943 | 3.048 | 3.066 | 3.234 | 3.305 | 3.193 | 3.354 | 3.309 | 3.337 |
| | $^3B_{1g}$ $(\pi \rightarrow \pi^\star)$ | 3.252 | 3.285 | 3.316 | 3.316 | 2.862 | 3.287 | 3.313 | 3.526 | 3.608 | 3.475 | 3.698 | 3.690 | 3.732 |
| Phthalimide | $^1B_1$ $(n \rightarrow \pi^\star)$ | 3.626 | 3.685 | 3.819 | 3.914 | 4.059 | 3.928 | 3.937 | 4.328 | 4.166 | 3.963 | 4.231 | 4.201 | 4.375 |
| | $^1A_1$ $(\pi \rightarrow \pi^\star)$ | 4.602 | 4.608 | 4.663 | 4.780 | 4.911 | 4.665 | 4.669 | 5.020 | 5.015 | 4.881 | 5.074 | 5.063 | 5.068 |
| | $^1A_2$ $(n \rightarrow \pi^\star)$ | 4.295 | 4.340 | 4.463 | 4.556 | 4.695 | 4.557 | 4.568 | 4.945 | 4.776 | 4.529 | 4.793 | 4.772 | 4.961 |
| | $^1B_2$ $(\pi \rightarrow \pi^\star)$ | 4.477 | 4.492 | 4.569 | 4.692 | 4.793 | 4.627 | 4.648 | 4.984 | 4.954 | 4.843 | 5.044 | 5.052 | 5.088 |
| | $^1B_2$ $(\pi \rightarrow \pi^\star)$ | 5.618 | 5.673 | 5.760 | 5.902 | 6.037 | 5.847 | 5.873 | 6.207 | 6.217 | 6.082 | 6.223 | 6.254 | 6.282 |
| | $^1A_2$ $(n \rightarrow \pi^\star)$ | 4.787 | 4.933 | 5.201 | 5.420 | 5.707 | 5.397 | 5.407 | 6.255 | 6.167 | 5.964 | 6.429 | 6.435 | 6.489 |
| | $^1A_1$ $(\pi \rightarrow \pi^\star)$ | 6.222 | 6.217 | 6.264 | 6.375 | 6.536 | 6.220 | 6.253 | 6.648 | 6.647 | 6.484 | 6.645 | 6.664 | 6.704 |
| | $^3B_2$ $(\pi \rightarrow \pi^\star)$ | 3.522 | 3.561 | 3.574 | 3.563 | 2.920 | 3.561 | 3.584 | 3.779 | 3.851 | 3.709 | 3.996 | 3.967 | 4.007 |
| | $^3B_1$ $(n \rightarrow \pi^\star)$ | 3.252 | 3.340 | 3.448 | 3.497 | 3.587 | 3.656 | 3.665 | 3.925 | 3.766 | 3.725 | 3.918 | 3.851 | 4.034 |
| | $^3A_1$ $(\pi \rightarrow \pi^\star)$ | 3.854 | 3.877 | 3.915 | 3.975 | 3.864 | 3.950 | 3.976 | 4.216 | 4.245 | 4.139 | 4.358 | 4.318 | 4.357 |
| | $^3B_2$ $(\pi \rightarrow \pi^\star)$ | 3.999 | 4.072 | 4.125 | 4.168 | 4.091 | 4.312 | 4.346 | 4.492 | 4.441 | 4.376 | 4.495 | 4.491 | 4.544 |
| | $^3A_2$ $(n \rightarrow \pi^\star)$ | 3.903 | 3.974 | 4.068 | 4.112 | 4.187 | 4.267 | 4.278 | 4.519 | 4.353 | 4.271 | 4.461 | 4.404 | 4.600 |
| | $^3B_2$ $(\pi \rightarrow \pi^\star)$ | 4.350 | 4.380 | 4.399 | 4.395 | 4.237 | 4.434 | 4.466 | 4.634 | 4.694 | 4.518 | 4.742 | 4.750 | 4.808 |
| Tolan | $^1B_{2u}$ $(\pi \rightarrow \pi^\star)$ | 4.539 | 4.561 | 4.636 | 4.778 | 4.923 | 4.664 | 4.673 | 5.052 | 5.065 | 4.938 | 5.071 | 5.103 | 5.110 |
| | $^1B_{3g}$ $(\pi \rightarrow \pi^\star)$ | 4.572 | 4.595 | 4.678 | 4.815 | 4.959 | 4.709 | 4.715 | 5.091 | 5.098 | 4.969 | 5.124 | 5.141 | 5.146 |
| | $^1B_{1u}$ $(\pi \rightarrow \pi^\star)$ | 4.247 | 4.234 | 4.277 | 4.371 | 4.356 | 4.245 | 4.271 | 4.528 | 4.574 | 4.452 | 4.656 | 4.644 | 4.681 |
| | $^1A_u$ $(\pi \rightarrow \pi^\star)$ | 4.674 | 4.666 | 4.762 | 4.856 | 4.909 | 4.770 | 4.809 | 5.126 | 5.038 | 4.876 | 5.033 | 5.012 | 5.187 |
| | $^1B_{3u}$ (Ryd) | 5.148 | 5.294 | 5.118 | 5.382 | 5.757 | 4.441 | 4.474 | 5.388 | 5.752 | 6.045 | 4.960 | 5.472 | 5.513 |
| | $^3B_{1u}$ $(\pi \rightarrow \pi^\star)$ | 2.914 | 2.945 | 2.973 | 2.968 | 2.471 | 3.002 | 3.030 | 3.180 | 3.228 | 3.101 | 3.345 | 3.345 | 3.395 |
| | $^3A_g$ $(\pi \rightarrow \pi^\star)$ | 3.982 | 4.032 | 4.017 | 3.971 | 3.202 | 3.947 | 3.972 | 4.173 | 4.281 | 4.091 | 4.385 | 4.383 | 4.425 |

Table S15: VTEs (in eV) computed with TDA-DFT using the aug-cc-pVTZ basis set.

| Compound | State | M06-SX | cM06-SX | CAM-BLYP | tCAM-B3LYP | mCAM-B3LYP | rCAM-B3LYP | ωB97X-D | ωB97M-V | ωB97X | ωB97 | LC-ωPBE | M11 |
|---|---|---|---|---|---|---|---|---|---|---|---|---|---|
| Anthracene | $^1B_{1u}$ ($\pi\rightarrow\pi^\star$) | 3.598 | 3.593 | 3.771 | 3.551 | 3.563 | 4.041 | 3.823 | 3.904 | 3.968 | 4.046 | 4.076 | 3.982 |
| | $^1B_{2u}$ ($\pi\rightarrow\pi^\star$) | 4.109 | 4.108 | 4.118 | 3.927 | 3.987 | 4.283 | 4.140 | 4.190 | 4.228 | 4.282 | 4.277 | 4.287 |
| | $^1B_{3g}$ ($\pi\rightarrow\pi^\star$) | 4.906 | 4.904 | 5.298 | 4.818 | 4.839 | 5.555 | 5.379 | 5.730 | 5.530 | 5.616 | 5.651 | 5.500 |
| | $^1B_{2g}$ (Ryd) | 5.405 | 5.397 | 5.074 | 4.668 | 4.816 | 5.254 | 5.336 | 4.888 | 5.614 | 5.720 | 5.737 | 4.652 |
| | $^1B_{1u}$ ($\pi\rightarrow\pi^\star$) | 5.496 | 5.487 | 5.422 | 4.988 | 5.159 | 5.705 | 5.586 | 5.347 | 5.814 | 5.942 | 5.978 | 5.238 |
| | $^1B_{3g}$ ($\pi\rightarrow\pi^\star$) | 5.280 | 5.269 | 5.382 | 5.060 | 5.145 | 6.196 | 5.469 | 5.419 | 5.852 | 6.079 | 6.084 | 5.807 |
| | $^1A_g$ ($\pi\rightarrow\pi^\star$) | 5.876 | 5.874 | 5.874 | 5.538 | 5.673 | 6.154 | 5.880 | 5.969 | 6.050 | 6.167 | 6.159 | 6.106 |
| | $^1B_{3u}$ (Ryd) | 5.601 | 5.597 | 5.347 | 4.936 | 5.060 | 5.598 | 5.624 | 5.213 | 5.989 | 6.083 | 6.041 | 4.895 |
| | $^1A_u$ (Ryd) | 5.593 | 5.588 | 5.405 | 5.022 | 5.077 | 5.675 | 5.713 | 5.317 | 6.059 | 6.154 | 6.133 | 5.038 |
| | $^1B_{2u}$ ($\pi\rightarrow\pi^\star$) | 5.797 | 5.780 | 5.764 | 5.547 | 5.640 | 5.928 | 5.788 | 5.768 | 5.880 | 5.943 | 5.956 | 5.819 |
| | $^3B_{1u}$ ($\pi\rightarrow\pi^\star$) | 2.248 | 2.240 | 2.186 | 2.172 | 2.135 | 2.093 | 2.242 | 2.352 | 2.267 | 2.287 | 2.189 | 2.288 |
| | $^3B_{3g}$ ($\pi\rightarrow\pi^\star$) | 3.712 | 3.698 | 3.549 | 3.548 | 3.519 | 3.367 | 3.614 | 3.706 | 3.616 | 3.622 | 3.500 | 3.644 |
| | $^3B_{2u}$ ($\pi\rightarrow\pi^\star$) | 3.743 | 3.725 | 3.713 | 3.607 | 3.615 | 3.784 | 3.766 | 3.820 | 3.826 | 3.860 | 3.803 | 3.821 |
| Anthraquinone | $^1B_{1g}$ ($n\rightarrow\pi^\star$) | 3.090 | 3.071 | 3.347 | 2.920 | 3.128 | 3.791 | 3.320 | 3.453 | 3.479 | 3.550 | 3.490 | 3.260 |
| | $^1A_u$ ($n\rightarrow\pi^\star$) | 3.430 | 3.407 | 3.607 | 3.218 | 3.408 | 3.984 | 3.584 | 3.701 | 3.723 | 3.788 | 3.728 | 3.514 |
| | $^1A_g$ ($\pi\rightarrow\pi^\star$) | 4.289 | 4.288 | 4.497 | 4.065 | 4.185 | 4.899 | 4.525 | 4.701 | 4.758 | 4.889 | 4.887 | 4.817 |
| | $^1B_{2u}$ ($\pi\rightarrow\pi^\star$) | 4.261 | 4.259 | 4.449 | 4.011 | 4.143 | 4.842 | 4.465 | 4.650 | 4.701 | 4.837 | 4.832 | 4.760 |
| | $^1B_{3g}$ ($\pi\rightarrow\pi^\star$) | 4.076 | 4.070 | 4.261 | 3.853 | 3.971 | 4.675 | 4.290 | 4.478 | 4.533 | 4.678 | 4.687 | 4.578 |
| | $^1B_{1u}$ ($\pi\rightarrow\pi^\star$) | 5.030 | 5.026 | 5.235 | 4.878 | 4.945 | 5.455 | 5.282 | 5.382 | 5.452 | 5.535 | 5.561 | 5.491 |
| | $^1B_{2u}$ ($\pi\rightarrow\pi^\star$) | 5.459 | 5.453 | 5.635 | 5.236 | 5.331 | 6.107 | 5.692 | 5.824 | 5.917 | 6.053 | 6.056 | 5.934 |
| | $^3B_{1g}$ ($n\rightarrow\pi^\star$) | 2.737 | 2.718 | 2.882 | 2.520 | 2.697 | 3.258 | 2.879 | 3.085 | 3.017 | 3.086 | 2.952 | 2.841 |
| | $^3A_u$ ($n\rightarrow\pi^\star$) | 3.060 | 3.036 | 3.128 | 2.802 | 2.962 | 3.445 | 3.130 | 3.324 | 3.252 | 3.318 | 3.180 | 3.092 |
| | $^3B_{1u}$ ($\pi\rightarrow\pi^\star$) | 3.388 | 3.376 | 3.300 | 3.257 | 3.228 | 3.153 | 3.366 | 3.502 | 3.404 | 3.431 | 3.306 | 3.474 |
| | $^3B_{3g}$ ($\pi\rightarrow\pi^\star$) | 3.413 | 3.404 | 3.360 | 3.224 | 3.248 | 3.258 | 3.419 | 3.578 | 3.483 | 3.513 | 3.400 | 3.549 |
| | $^3A_g$ ($\pi\rightarrow\pi^\star$) | 3.440 | 3.432 | 3.512 | 3.263 | 3.314 | 3.724 | 3.560 | 3.725 | 3.716 | 3.815 | 3.758 | 3.764 |
| Aza-BODIPY | $^1B_2$ ($\pi\rightarrow\pi^\star$) | 3.286 | 3.278 | 3.181 | 3.117 | 3.190 | 2.995 | 3.179 | 3.073 | 3.090 | 3.029 | 3.044 | 3.139 |
| | $^1B_2$ ($\pi\rightarrow\pi^\star$) | 3.904 | 3.897 | 3.871 | 3.699 | 3.787 | 4.188 | 3.867 | 3.975 | 4.016 | 4.124 | 4.130 | 4.046 |
| | $^1A_1$ ($\pi\rightarrow\pi^\star$) | 3.858 | 3.854 | 4.010 | 3.615 | 3.746 | 4.456 | 4.021 | 4.201 | 4.243 | 4.372 | 4.365 | 4.260 |
| | $^1B_1$ ($n\rightarrow\pi^\star$) | 3.789 | 3.769 | 3.896 | 3.507 | 3.756 | 4.278 | 3.840 | 3.958 | 3.976 | 4.056 | 3.997 | 3.752 |
| | $^3B_2$ ($\pi\rightarrow\pi^\star$) | 1.312 | 1.305 | 1.094 | 1.248 | 1.200 | 0.867 | 1.116 | 1.091 | 1.018 | 0.959 | 0.900 | 1.076 |
| | $^3B_2$ ($\pi\rightarrow\pi^\star$) | 2.772 | 2.764 | 2.758 | 2.571 | 2.627 | 2.902 | 2.790 | 2.935 | 2.896 | 2.965 | 2.892 | 2.922 |
| | $^3A_1$ ($\pi\rightarrow\pi^\star$) | 3.014 | 3.006 | 2.999 | 2.801 | 2.858 | 3.122 | 3.028 | 3.185 | 3.137 | 3.205 | 3.121 | 3.157 |
| | $^3B_1$ ($n\rightarrow\pi^\star$) | 3.280 | 3.256 | 3.232 | 2.946 | 3.149 | 3.474 | 3.213 | 3.411 | 3.307 | 3.380 | 3.232 | 3.087 |
| Azobenzene | $^1B_g$ ($n\rightarrow\pi^\star$) | 2.737 | 2.708 | 2.862 | 2.613 | 2.762 | 3.129 | 2.829 | 2.903 | 2.920 | 2.971 | 2.903 | 2.681 |
| | $^1B_u$ ($\pi\rightarrow\pi^\star$) | 4.133 | 4.123 | 4.195 | 3.929 | 4.019 | 4.453 | 4.229 | 4.319 | 4.374 | 4.474 | 4.512 | 4.425 |
| | $^1A_g$ ($\pi\rightarrow\pi^\star$) | 4.504 | 4.503 | 4.734 | 4.261 | 4.384 | 5.151 | 4.765 | 4.953 | 5.002 | 5.131 | 5.131 | 5.070 |
| | $^1B_u$ ($\pi\rightarrow\pi^\star$) | 4.499 | 4.497 | 4.719 | 4.244 | 4.374 | 5.138 | 4.749 | 4.937 | 4.988 | 5.118 | 5.120 | 5.055 |
| | $^1A_g$ ($\pi\rightarrow\pi^\star$) | 5.219 | 5.216 | 5.495 | 5.099 | 5.133 | 5.830 | 5.578 | 5.708 | 5.778 | 5.880 | 5.920 | 5.828 |
| | $^3B_g$ ($n\rightarrow\pi^\star$) | 2.106 | 2.072 | 2.047 | 1.919 | 2.004 | 2.183 | 2.069 | 2.249 | 2.129 | 2.183 | 1.985 | 1.911 |
| | $^3B_u$ ($\pi\rightarrow\pi^\star$) | 2.711 | 2.700 | 2.641 | 2.575 | 2.560 | 2.578 | 2.707 | 2.855 | 2.767 | 2.814 | 2.734 | 2.820 |
| | $^3A_g$ ($\pi\rightarrow\pi^\star$) | 3.918 | 3.909 | 3.836 | 3.771 | 3.737 | 3.610 | 3.918 | 4.058 | 3.932 | 3.931 | 3.793 | 3.992 |
| | $^3B_u$ ($\pi\rightarrow\pi^\star$) | 3.975 | 3.967 | 4.070 | 3.734 | 3.819 | 4.214 | 4.120 | 4.310 | 4.295 | 4.386 | 4.310 | 4.331 |
| | $^3A_g$ ($\pi\rightarrow\pi^\star$) | 4.074 | 4.065 | 4.125 | 3.883 | 3.902 | 4.392 | 4.173 | 4.358 | 4.345 | 4.445 | 4.379 | 4.373 |
| BODIPY | $^1B_2$ ($\pi\rightarrow\pi^\star$) | 3.548 | 3.539 | 3.415 | 3.386 | 3.442 | 3.298 | 3.416 | 3.327 | 3.359 | 3.328 | 3.330 | 3.387 |
| | $^1B_2$ ($\pi\rightarrow\pi^\star$) | 4.115 | 4.109 | 4.194 | 3.875 | 3.997 | 4.601 | 4.196 | 4.338 | 4.407 | 4.544 | 4.540 | 4.417 |
| | $^1A_1$ ($\pi\rightarrow\pi^\star$) | 4.214 | 4.209 | 4.389 | 3.959 | 4.096 | 4.868 | 4.401 | 4.582 | 4.651 | 4.800 | 4.786 | 4.649 |
| | $^3B_2$ ($\pi\rightarrow\pi^\star$) | 1.808 | 1.799 | 1.645 | 1.706 | 1.684 | 1.542 | 1.673 | 1.679 | 1.639 | 1.621 | 1.550 | 1.669 |
| | $^3B_2$ ($\pi\rightarrow\pi^\star$) | 3.105 | 3.097 | 3.095 | 2.892 | 2.950 | 3.238 | 3.129 | 3.276 | 3.249 | 3.328 | 3.246 | 3.276 |
| | $^3A_1$ ($\pi\rightarrow\pi^\star$) | 3.325 | 3.317 | 3.304 | 3.100 | 3.159 | 3.383 | 3.333 | 3.487 | 3.445 | 3.515 | 3.420 | 3.467 |
| Coumarin | $^1A'$ ($\pi\rightarrow\pi^\star$) | 4.592 | 4.587 | 4.638 | 4.313 | 4.450 | 4.878 | 4.646 | 4.719 | 4.784 | 4.865 | 4.870 | 4.805 |
| | $^1A''$ ($n\rightarrow\pi^\star$) | 4.772 | 4.753 | 4.963 | 4.399 | 4.676 | 5.441 | 4.935 | 5.110 | 5.144 | 5.246 | 5.183 | 4.940 |
| | $^1A'$ ($\pi\rightarrow\pi^\star$) | 5.061 | 5.052 | 5.120 | 4.821 | 4.922 | 5.319 | 5.149 | 5.221 | 5.287 | 5.365 | 5.386 | 5.339 |
| | $^3A'$ ($\pi\rightarrow\pi^\star$) | 3.234 | 3.220 | 3.106 | 3.072 | 3.063 | 2.977 | 3.167 | 3.264 | 3.187 | 3.204 | 3.091 | 3.219 |
| | $^3A'$ ($\pi\rightarrow\pi^\star$) | 3.994 | 3.985 | 3.950 | 3.751 | 3.811 | 3.924 | 3.993 | 4.135 | 4.085 | 4.130 | 4.017 | 4.112 |
| | $^3A''$ ($n\rightarrow\pi^\star$) | 4.467 | 4.448 | 4.550 | 4.079 | 4.313 | 4.943 | 4.548 | 4.779 | 4.726 | 4.821 | 4.688 | 4.560 |
| Cyclazine | $^1A_2'$ ($\pi\rightarrow\pi^\star$) | 1.367 | 1.354 | 1.325 | 1.232 | 1.283 | 1.486 | 1.346 | 1.367 | 1.386 | 1.418 | 1.407 | 1.431 |
| | $^1E'$ ($\pi\rightarrow\pi^\star$) | 3.549 | 3.543 | 3.524 | 3.317 | 3.398 | 3.749 | 3.580 | 3.541 | 3.677 | 3.740 | 3.751 | 3.578 |
| | $^1A_1''$ (Ryd) | 3.756 | 3.746 | 3.376 | 3.055 | 3.193 | 3.533 | 3.648 | 3.151 | 3.853 | 3.931 | 3.942 | 2.919 |
| | $^1E''$ (Ryd) | 4.112 | 4.107 | 3.834 | 3.539 | 3.603 | 4.058 | 4.119 | 3.681 | 4.425 | 4.475 | 4.428 | 3.321 |
| | $^3A_2'$ ($\pi\rightarrow\pi^\star$) | 1.191 | 1.179 | 1.106 | 1.040 | 1.078 | 1.231 | 1.136 | 1.179 | 1.167 | 1.192 | 1.115 | 1.212 |
| | $^3E'$ ($\pi\rightarrow\pi^\star$) | 2.303 | 2.295 | 2.174 | 2.102 | 2.137 | 2.248 | 2.224 | 2.263 | 2.256 | 2.287 | 2.206 | 2.265 |
| | $^3A_1''$ (Ryd) | 3.737 | 3.729 | 3.367 | 3.053 | 3.191 | 3.528 | 3.632 | 3.188 | 3.848 | 3.914 | 3.913 | 2.975 |
| | $^3E''$ (Ryd) | 4.074 | 4.069 | 3.833 | 3.543 | 3.607 | 4.060 | 4.077 | 3.711 | 4.371 | 4.422 | 4.406 | 3.408 |

Table S16: VTEs (in eV) computed with TDA-DFT using the aug-cc-pVTZ basis set.

| Compound | State | M06-SX | cM06-SX | CAM-BLYP | tCAM-B3LYP | mCAM-B3LYP | rCAM-B3LYP | $\omega$B97X-D | $\omega$B97M-V | $\omega$B97X | $\omega$B97 | LC-$\omega$PBE | M11 |
|---|---|---|---|---|---|---|---|---|---|---|---|---|---|
| Heptazine | $^1A_2'$ $(\pi \rightarrow \pi^\star)$ | 3.206 | 3.193 | 3.184 | 2.901 | 3.040 | 3.507 | 3.207 | 3.283 | 3.337 | 3.416 | 3.362 | 3.312 |
| | $^1A_1''$ $(n \rightarrow \pi^\star)$ | 4.158 | 4.149 | 4.247 | 3.563 | 3.961 | 4.871 | 4.225 | 4.397 | 4.428 | 4.514 | 4.434 | 4.403 |
| | $^1E''$ $(n \rightarrow \pi^\star)$ | 4.171 | 4.162 | 4.293 | 3.689 | 4.030 | 4.858 | 4.257 | 4.414 | 4.448 | 4.526 | 4.437 | 4.389 |
| | $^1E'$ $(\pi \rightarrow \pi^\star)$ | 5.051 | 5.045 | 5.102 | 4.712 | 4.878 | 5.459 | 5.123 | 5.208 | 5.300 | 5.402 | 5.376 | 5.267 |
| | $^3A_2'$ $(\pi \rightarrow \pi^\star)$ | 3.003 | 2.990 | 2.934 | 2.685 | 2.808 | 3.217 | 2.970 | 3.064 | 3.085 | 3.156 | 3.071 | 3.056 |
| | $^3E''(\pi \rightarrow \pi^\star)$ | 3.747 | 3.736 | 3.635 | 3.429 | 3.525 | 3.835 | 3.678 | 3.778 | 3.780 | 3.854 | 3.755 | 3.756 |
| | $^3A_1''$ $(n \rightarrow \pi^\star)$ | 4.057 | 4.047 | 4.101 | 3.462 | 3.837 | 4.680 | 4.091 | 4.293 | 4.284 | 4.373 | 4.256 | 4.232 |
| | $^3E''$ $(n \rightarrow \pi^\star)$ | 4.064 | 4.055 | 4.140 | 3.566 | 3.893 | 4.675 | 4.118 | 4.310 | 4.302 | 4.383 | 4.257 | 4.228 |
| Naphthalimide | $^1B_2$ $(\pi \rightarrow \pi^\star)$ | 4.390 | 4.389 | 4.401 | 4.141 | 4.245 | 4.598 | 4.411 | 4.487 | 4.529 | 4.603 | 4.598 | 4.587 |
| | $^1B_1$ $(n \rightarrow \pi^\star)$ | 4.074 | 4.059 | 4.358 | 3.738 | 4.001 | 4.920 | 4.341 | 4.543 | 4.574 | 4.678 | 4.612 | 4.410 |
| | $^1A_1$ $(\pi \rightarrow \pi^\star)$ | 4.172 | 4.166 | 4.283 | 4.000 | 4.078 | 4.535 | 4.315 | 4.415 | 4.474 | 4.562 | 4.586 | 4.496 |
| | $^1A_2$ $(n \rightarrow \pi^\star)$ | 4.547 | 4.532 | 4.775 | 4.236 | 4.489 | 5.245 | 4.754 | 4.909 | 4.940 | 5.023 | 4.949 | 4.732 |
| | $^3A_1$ $(\pi \rightarrow \pi^\star)$ | 2.777 | 2.768 | 2.689 | 2.637 | 2.627 | 2.598 | 2.744 | 2.864 | 2.779 | 2.802 | 2.701 | 2.811 |
| | $^3B_2$ $(\pi \rightarrow \pi^\star)$ | 3.694 | 3.684 | 3.644 | 3.500 | 3.535 | 3.680 | 3.688 | 3.789 | 3.765 | 3.813 | 3.739 | 3.791 |
| | $^3B_1$ $(n \rightarrow \pi^\star)$ | 3.836 | 3.820 | 4.009 | 3.474 | 3.710 | 4.484 | 4.011 | 4.257 | 4.211 | 4.308 | 4.178 | 4.074 |
| | $^3B_2$ $(\pi \rightarrow \pi^\star)$ | 4.155 | 4.141 | 4.001 | 3.930 | 3.946 | 3.934 | 4.056 | 4.146 | 4.087 | 4.116 | 4.017 | 4.132 |
| | $^3A_2$ $(n \rightarrow \pi^\star)$ | 4.277 | 4.261 | 4.391 | 3.935 | 4.154 | 4.785 | 4.390 | 4.601 | 4.551 | 5.023 | 4.489 | 4.376 |
| Naphthoquinone | $^1B_1$ $(n \rightarrow \pi^\star)$ | 2.851 | 2.830 | 3.120 | 2.672 | 2.896 | 3.620 | 3.079 | 3.236 | 3.261 | 3.351 | 3.286 | 3.019 |
| | $^1A_2$ $(n \rightarrow \pi^\star)$ | 3.159 | 3.134 | 3.371 | 2.926 | 3.142 | 3.816 | 3.339 | 3.497 | 3.513 | 3.599 | 3.546 | 3.301 |
| | $^1A_1$ $(\pi \rightarrow \pi^\star)$ | 4.044 | 4.043 | 4.281 | 3.763 | 3.929 | 4.771 | 4.292 | 4.531 | 4.587 | 4.752 | 4.749 | 4.635 |
| | $^1B_2$ $(\pi \rightarrow \pi^\star)$ | 3.983 | 3.976 | 4.170 | 3.709 | 3.868 | 4.626 | 4.172 | 4.388 | 4.445 | 4.615 | 4.621 | 4.474 |
| | $^1A_2$ $(n \rightarrow \pi^\star)$ | 5.307 | 5.302 | 5.833 | 4.810 | 5.254 | 7.020 | 5.797 | 6.167 | 6.261 | 6.476 | 6.435 | 6.195 |
| | $^1A_1$ $(\pi \rightarrow \pi^\star)$ | 5.720 | 5.716 | 5.765 | 5.383 | 5.526 | 6.189 | 5.792 | 5.922 | 6.011 | 6.156 | 6.156 | 6.048 |
| | $^1B_2$ $(\pi \rightarrow \pi^\star)$ | 5.454 | 5.447 | 5.587 | 5.168 | 5.321 | 5.880 | 5.584 | 5.707 | 5.797 | 5.925 | 5.941 | 5.802 |
| | $^3B_1$ $(n \rightarrow \pi^\star)$ | 2.471 | 2.451 | 2.631 | 2.246 | 2.437 | 3.062 | 2.617 | 2.852 | 2.779 | 2.866 | 2.726 | 2.582 |
| | $^3A_2$ $(n \rightarrow \pi^\star)$ | 2.768 | 2.743 | 2.870 | 2.493 | 2.675 | 3.251 | 2.866 | 3.101 | 3.019 | 3.105 | 2.974 | 2.858 |
| | $^3B_2$ $(\pi \rightarrow \pi^\star)$ | 3.190 | 3.176 | 3.090 | 3.032 | 3.034 | 2.968 | 3.142 | 3.274 | 3.184 | 3.226 | 3.096 | 3.219 |
| | $^3B_2$ $(\pi \rightarrow \pi^\star)$ | 3.266 | 3.253 | 3.224 | 3.079 | 3.098 | 3.180 | 3.269 | 3.444 | 3.363 | 3.414 | 3.303 | 3.420 |
| | $^3A_1$ $(\pi \rightarrow \pi^\star)$ | 3.368 | 3.361 | 3.480 | 3.136 | 3.236 | 3.758 | 3.510 | 3.722 | 3.715 | 3.837 | 3.782 | 3.758 |
| Phenazine | $^1B_{1u}$ $(n \rightarrow \pi^\star)$ | 3.235 | 3.220 | 3.513 | 3.041 | 3.301 | 4.036 | 3.439 | 3.605 | 3.632 | 3.725 | 3.673 | 3.419 |
| | $^1B_{3u}$ $(\pi \rightarrow \pi^\star)$ | 3.562 | 3.557 | 3.761 | 3.480 | 3.520 | 4.107 | 3.806 | 3.938 | 3.992 | 4.096 | 4.123 | 4.029 |
| | $^1B_{2u}$ $(\pi \rightarrow \pi^\star)$ | 4.140 | 4.139 | 4.132 | 3.957 | 4.020 | 4.249 | 4.146 | 4.189 | 4.216 | 4.255 | 4.257 | 4.292 |
| | $^1B_{1g}$ $(\pi \rightarrow \pi^\star)$ | 4.423 | 4.417 | 4.704 | 4.284 | 4.351 | 5.224 | 4.756 | 4.975 | 5.026 | 5.174 | 5.189 | 5.068 |
| | $^1B_{2g}$ $(n \rightarrow \pi^\star)$ | 5.035 | 5.014 | 5.180 | 4.602 | 4.920 | 5.694 | 5.140 | 5.348 | 5.379 | 5.523 | 5.445 | 5.211 |
| | $^1A_u$ $(\pi \rightarrow \pi^\star)$ | 5.156 | 5.149 | 5.437 | 4.749 | 5.119 | 6.173 | 5.370 | 5.570 | 5.627 | 5.725 | 5.650 | 5.462 |
| | $^3B_{3u}$ $(\pi \rightarrow \pi^\star)$ | 2.326 | 2.318 | 2.290 | 2.250 | 2.218 | 2.223 | 2.347 | 2.476 | 2.395 | 2.429 | 2.344 | 2.447 |
| | $^3B_{1u}$ $(n \rightarrow \pi^\star)$ | 2.832 | 2.815 | 2.974 | 2.599 | 2.809 | 3.379 | 2.935 | 3.174 | 3.096 | 3.185 | 3.056 | 2.896 |
| | $^3B_{2u}$ $(\pi \rightarrow \pi^\star)$ | 3.263 | 3.254 | 3.182 | 3.123 | 3.129 | 3.172 | 3.218 | 3.274 | 3.239 | 3.248 | 3.202 | 3.312 |
| | $^3B_{1g}$ $(\pi \rightarrow \pi^\star)$ | 3.531 | 3.520 | 3.441 | 3.390 | 3.370 | 3.310 | 3.501 | 3.620 | 3.529 | 3.543 | 3.427 | 3.563 |
| Phthalimide | $^1B_1$ $(n \rightarrow \pi^\star)$ | 4.061 | 4.041 | 4.258 | 3.763 | 4.007 | 4.749 | 4.230 | 4.393 | 4.420 | 4.511 | 4.450 | 4.209 |
| | $^1A_1$ $(\pi \rightarrow \pi^\star)$ | 4.966 | 4.964 | 4.960 | 4.631 | 4.783 | 5.178 | 4.958 | 5.056 | 5.103 | 5.196 | 5.188 | 5.172 |
| | $^1A_2$ $(n \rightarrow \pi^\star)$ | 4.695 | 4.673 | 4.843 | 4.407 | 4.629 | 5.251 | 4.820 | 4.955 | 4.980 | 5.055 | 4.982 | 4.737 |
| | $^1B_2$ $(\pi \rightarrow \pi^\star)$ | 4.878 | 4.869 | 4.917 | 4.525 | 4.711 | 5.219 | 4.913 | 5.038 | 5.089 | 5.197 | 5.191 | 5.085 |
| | $^1B_2$ $(\pi \rightarrow \pi^\star)$ | 6.112 | 6.106 | 6.177 | 5.757 | 5.942 | 6.432 | 6.186 | 6.249 | 6.343 | 6.429 | 6.447 | 6.344 |
| | $^1A_2$ $(n \rightarrow \pi^\star)$ | 5.743 | 5.739 | 6.260 | 5.170 | 5.626 | 7.386 | 6.225 | 6.612 | 6.705 | 6.908 | 6.878 | 6.664 |
| | $^1A_1$ $(\pi \rightarrow \pi^\star)$ | 6.604 | 6.592 | 6.588 | 6.207 | 6.386 | 6.881 | 6.607 | 6.667 | 6.777 | 6.888 | 6.892 | 6.757 |
| | $^3B_2$ $(\pi \rightarrow \pi^\star)$ | 3.811 | 3.800 | 3.641 | 3.612 | 3.598 | 3.413 | 3.711 | 3.852 | 3.718 | 3.720 | 3.587 | 3.779 |
| | $^3B_1$ $(n \rightarrow \pi^\star)$ | 3.731 | 3.711 | 3.828 | 3.394 | 3.610 | 4.257 | 3.823 | 4.055 | 3.994 | 4.083 | 3.954 | 3.820 |
| | $^3A_1$ $(\pi \rightarrow \pi^\star)$ | 4.199 | 4.187 | 4.148 | 3.927 | 4.009 | 4.278 | 4.180 | 4.313 | 4.298 | 4.377 | 4.312 | 4.326 |
| | $^3B_2$ $(\pi \rightarrow \pi^\star)$ | 4.432 | 4.417 | 4.383 | 4.103 | 4.231 | 4.510 | 4.403 | 4.539 | 4.525 | 4.597 | 4.508 | 4.514 |
| | $^3A_2$ $(n \rightarrow \pi^\star)$ | 4.345 | 4.324 | 4.389 | 4.017 | 4.206 | 4.737 | 4.391 | 4.600 | 4.532 | 4.606 | 4.462 | 4.330 |
| | $^3B_2$ $(\pi \rightarrow \pi^\star)$ | 4.648 | 4.631 | 4.529 | 4.420 | 4.434 | 4.689 | 4.579 | 4.692 | 4.664 | 4.740 | 4.642 | 4.672 |
| Tolan | $^1B_{2u}$ $(\pi \rightarrow \pi^\star)$ | 4.970 | 4.968 | 5.049 | 4.739 | 4.829 | 5.279 | 5.088 | 5.144 | 5.220 | 5.300 | 5.302 | 5.266 |
| | $^1B_{3g}$ $(\pi \rightarrow \pi^\star)$ | 5.002 | 5.000 | 5.085 | 4.784 | 4.862 | 5.305 | 5.118 | 5.182 | 5.247 | 5.325 | 5.324 | 5.305 |
| | $^1B_{1u}$ $(\pi \rightarrow \pi^\star)$ | 4.468 | 4.457 | 4.560 | 4.366 | 4.392 | 4.719 | 4.602 | 4.648 | 4.722 | 4.788 | 4.820 | 4.772 |
| | $^1A_u$ $(\pi \rightarrow \pi^\star)$ | 4.951 | 4.929 | 5.150 | 4.805 | 4.926 | 5.449 | 5.147 | 5.230 | 5.336 | 5.428 | 5.405 | 5.106 |
| | $^1B_{3u}$ (Ryd) | 5.871 | 5.863 | 5.563 | 5.058 | 5.380 | 5.825 | 5.803 | 5.362 | 6.108 | 6.258 | 6.278 | 5.168 |
| | $^3B_{1u}$ $(\pi \rightarrow \pi^\star)$ | 3.167 | 3.153 | 3.110 | 3.064 | 3.027 | 3.012 | 3.183 | 3.315 | 3.225 | 3.245 | 3.133 | 3.232 |
| | $^3A_g$ $(\pi \rightarrow \pi^\star)$ | 4.242 | 4.231 | 4.006 | 4.084 | 4.004 | 3.671 | 4.099 | 4.216 | 4.061 | 4.037 | 3.883 | 4.127 |

Table S17: VTEs (in eV) computed with TDA-DFT using the aug-cc-pVTZ basis set.

| Compound | State | B2PLYP | PBE0-DH | PBE-QIDH | $\omega$B2PLYP | RSH-0DH | RSX-QIDH | $\omega$B97X-2 | SOS-$\omega$B88PP86 | SOS-$\omega$PBEPP86 | cLH12ct-SsirPW92 | cLH14t-calPBE | cLH20t |
|---|---|---|---|---|---|---|---|---|---|---|---|---|---|
| Anthracene | $^1B_{1u}$ $(\pi \to \pi^\star)$ | 3.573 | 3.670 | 3.767 | 3.939 | 4.038 | 3.972 | 3.702 | 3.778 | 3.732 | 3.602 | 3.490 | 3.601 |
| | $^1B_{2u}$ $(\pi \to \pi^\star)$ | 3.894 | 4.067 | 4.067 | 4.176 | 4.333 | 4.229 | 3.607 | 3.842 | 3.771 | 4.059 | 3.954 | 4.026 |
| | $^1B_{3g}$ $(\pi \to \pi^\star)$ | 4.855 | 5.156 | 5.373 | 5.494 | 5.645 | 5.567 | 4.485 | 5.332 | 5.297 | 5.249 | 5.110 | 5.218 |
| | $^1B_{2g}$ (Ryd) | 4.822 | 5.156 | 5.227 | 5.231 | 5.679 | 5.498 | 5.190 | 5.319 | 5.399 | 5.426 | 5.173 | 5.000 |
| | $^1B_{1u}$ $(\pi \to \pi^\star)$ | 5.181 | 5.422 | 5.544 | 5.615 | 5.948 | 5.817 | 5.422 | 5.595 | 5.613 | 5.437 | 5.199 | 5.278 |
| | $^1B_{3g}$ $(\pi \to \pi^\star)$ | 5.043 | 5.208 | 5.208 | 5.721 | 6.075 | 5.798 | 5.203 | 5.361 | 5.285 | 4.887 | 4.653 | 4.905 |
| | $^1A_g$ $(\pi \to \pi^\star)$ | 5.558 | 5.813 | 5.825 | 5.995 | 6.244 | 6.080 | 5.241 | 5.629 | 5.557 | 5.794 | 5.638 | 5.749 |
| | $^1B_{3u}$ (Ryd) | 5.070 | 5.401 | 5.487 | 5.556 | 5.987 | 5.799 | 5.498 | 5.638 | 5.725 | 5.719 | 5.468 | 5.288 |
| | $^1A_u$ (Ryd) | 5.097 | 5.441 | 5.545 | 5.641 | 6.077 | 5.882 | 5.557 | 5.709 | 5.788 | 5.713 | 5.461 | 5.316 |
| | $^1B_{2u}$ $(\pi \to \pi^\star)$ | 5.474 | 5.694 | 5.651 | 5.767 | 5.965 | 5.821 | 5.129 | 5.581 | 5.528 | 5.742 | 5.644 | 5.701 |
| | $^3B_{1u}$ $(\pi \to \pi^\star)$ | 2.255 | 2.156 | 2.269 | 2.313 | 2.209 | 2.290 | 2.778 | 2.263 | 2.258 | 2.302 | 2.139 | 2.278 |
| | $^3B_{3g}$ $(\pi \to \pi^\star)$ | 3.629 | 3.543 | 3.628 | 3.653 | 3.548 | 3.632 | 4.143 | 3.589 | 3.590 | 3.760 | 3.554 | 3.711 |
| | $^3B_{2u}$ $(\pi \to \pi^\star)$ | 3.694 | 3.702 | 3.795 | 3.858 | 3.865 | 3.883 | 3.907 | 3.701 | 3.671 | 3.733 | 3.600 | 3.711 |
| Anthraquinone | $^1B_{1g}$ $(n \to \pi^\star)$ | 3.067 | 3.277 | 3.359 | 3.504 | 3.682 | 3.589 | 2.519 | 3.303 | 3.261 | 3.093 | 2.984 | 3.163 |
| | $^1A_u$ $(n \to \pi^\star)$ | 3.322 | 3.542 | 3.602 | 3.728 | 3.911 | 3.815 | 2.759 | 3.517 | 3.474 | 3.425 | 3.306 | 3.482 |
| | $^1A_g$ $(\pi \to \pi^\star)$ | 4.101 | 4.356 | 4.422 | 4.666 | 4.910 | 4.734 | 3.806 | 4.301 | 4.226 | 4.217 | 4.037 | 4.220 |
| | $^1B_{2u}$ $(\pi \to \pi^\star)$ | 4.122 | 4.347 | 4.434 | 4.650 | 4.875 | 4.723 | 3.881 | 4.297 | 4.227 | 4.177 | 3.999 | 4.181 |
| | $^1B_{3g}$ $(\pi \to \pi^\star)$ | 4.090 | 4.224 | 4.413 | 4.598 | 4.745 | 4.692 | 4.276 | 4.411 | 4.373 | 4.004 | 3.845 | 4.017 |
| | $^1B_{1u}$ $(\pi \to \pi^\star)$ | 4.961 | 5.122 | 5.260 | 5.417 | 5.549 | 5.482 | 5.165 | 5.214 | 5.170 | 4.974 | 4.796 | 4.971 |
| | $^1B_{2u}$ $(\pi \to \pi^\star)$ | 5.249 | 5.512 | 5.591 | 5.847 | 6.107 | 5.936 | 4.960 | 5.572 | 5.515 | 5.399 | 5.216 | 5.386 |
| | $^3B_{1g}$ $(n \to \pi^\star)$ | 2.728 | 2.833 | 2.963 | 3.083 | 3.166 | 3.148 | 2.428 | 2.971 | 2.950 | 2.760 | 2.576 | 2.822 |
| | $^3A_u$ $(n \to \pi^\star)$ | 2.975 | 3.087 | 3.199 | 3.302 | 3.389 | 3.369 | 2.665 | 3.185 | 3.164 | 3.078 | 2.880 | 3.125 |
| | $^3B_{1u}$ $(\pi \to \pi^\star)$ | 3.394 | 3.282 | 3.419 | 3.454 | 3.334 | 3.433 | 4.028 | 3.414 | 3.417 | 3.412 | 3.214 | 3.365 |
| | $^3B_{3g}$ $(\pi \to \pi^\star)$ | 3.463 | 3.368 | 3.531 | 3.565 | 3.456 | 3.557 | 4.132 | 3.533 | 3.538 | 3.401 | 3.210 | 3.384 |
| | $^3A_g$ $(\pi \to \pi^\star)$ | 3.502 | 3.495 | 3.680 | 3.790 | 3.802 | 3.830 | 3.914 | 3.686 | 3.667 | 3.406 | 3.222 | 3.387 |
| Aza-BODIPY | $^1B_2$ $(\pi \to \pi^\star)$ | 3.008 | 3.150 | 3.029 | 2.958 | 3.035 | 2.967 | 2.652 | 2.733 | 2.661 | 3.249 | 3.180 | 3.232 |
| | $^1B_2$ $(\pi \to \pi^\star)$ | 3.562 | 3.795 | 3.734 | 3.921 | 4.164 | 3.977 | 2.951 | 3.622 | 3.549 | 3.871 | 3.838 | 3.846 |
| | $^1A_1$ $(\pi \to \pi^\star)$ | 3.559 | 3.850 | 3.853 | 4.130 | 4.414 | 4.192 | 2.962 | 3.762 | 3.682 | 3.798 | 3.655 | 3.818 |
| | $^1B_1$ $(n \to \pi^\star)$ | 3.785 | 3.930 | 4.034 | 4.084 | 4.207 | 4.185 | 3.436 | 3.960 | 3.937 | 3.853 | 3.748 | 3.893 |
| | $^3B_2$ $(\pi \to \pi^\star)$ | 1.391 | 1.211 | 1.297 | 1.172 | 1.003 | 1.169 | 1.867 | 1.191 | 1.178 | 1.312 | 1.268 | 1.286 |
| | $^3B_2$ $(\pi \to \pi^\star)$ | 2.724 | 2.749 | 2.877 | 2.959 | 2.991 | 3.006 | 2.880 | 2.849 | 2.832 | 2.752 | 2.591 | 2.747 |
| | $^3A_1$ $(\pi \to \pi^\star)$ | 2.976 | 2.993 | 3.137 | 3.220 | 3.240 | 3.267 | 3.183 | 3.103 | 3.089 | 2.988 | 2.821 | 2.988 |
| | $^3B_1$ $(n \to \pi^\star)$ | 3.267 | 3.287 | 3.426 | 3.426 | 3.433 | 3.493 | 3.237 | 3.400 | 3.399 | 3.365 | 3.180 | 3.390 |
| Azobenzene | $^1B_g$ $(n \to \pi^\star)$ | 2.821 | 2.871 | 2.962 | 2.996 | 3.034 | 3.042 | 2.660 | 2.891 | 2.861 | 2.838 | 2.771 | 2.891 |
| | $^1B_u$ $(\pi \to \pi^\star)$ | 4.016 | 4.156 | 4.257 | 4.378 | 4.518 | 4.461 | 4.131 | 4.244 | 4.209 | 4.090 | 3.978 | 4.085 |
| | $^1A_g$ $(\pi \to \pi^\star)$ | 4.332 | 4.598 | 4.701 | 4.941 | 5.186 | 5.025 | 4.092 | 4.554 | 4.484 | 4.427 | 4.222 | 4.446 |
| | $^1B_u$ $(\pi \to \pi^\star)$ | 4.320 | 4.586 | 4.690 | 4.929 | 5.173 | 5.015 | 4.099 | 4.547 | 4.479 | 4.420 | 4.218 | 4.438 |
| | $^1A_g$ $(\pi \to \pi^\star)$ | 5.106 | 5.337 | 5.569 | 5.784 | 5.948 | 5.894 | 5.535 | 5.577 | 5.549 | 5.184 | 4.974 | 5.192 |
| | $^3B_g$ $(n \to \pi^\star)$ | 2.128 | 2.047 | 2.169 | 2.192 | 2.106 | 2.190 | 2.307 | 2.189 | 2.181 | 2.204 | 2.044 | 2.241 |
| | $^3B_u$ $(\pi \to \pi^\star)$ | 2.740 | 2.639 | 2.797 | 2.833 | 2.733 | 2.833 | 3.459 | 2.818 | 2.821 | 2.729 | 2.556 | 2.707 |
| | $^3A_g$ $(\pi \to \pi^\star)$ | 3.932 | 3.823 | 3.946 | 3.969 | 3.839 | 3.938 | 4.586 | 3.923 | 3.932 | 3.896 | 3.677 | 3.888 |
| | $^3B_u$ $(\pi \to \pi^\star)$ | 4.032 | 4.047 | 4.481 | 4.559 | 4.555 | 4.547 | 4.561 | 4.399 | 4.412 | 3.922 | 3.707 | 3.926 |
| | $^3A_g$ $(\pi \to \pi^\star)$ | 4.054 | 4.096 | 4.291 | 4.428 | 4.476 | 4.482 | 4.367 | 4.268 | 4.250 | 4.059 | 3.846 | 4.039 |
| BODIPY | $^1B_2$ $(\pi \to \pi^\star)$ | 3.201 | 3.369 | 3.231 | 3.216 | 3.328 | 3.232 | 2.773 | 2.960 | 2.886 | 3.518 | 3.467 | 3.486 |
| | $^1B_2$ $(\pi \to \pi^\star)$ | 3.814 | 4.076 | 4.069 | 4.303 | 4.568 | 4.367 | 3.271 | 3.987 | 3.919 | 4.075 | 3.983 | 4.068 |
| | $^1A_1$ $(\pi \to \pi^\star)$ | 3.909 | 4.219 | 4.237 | 4.531 | 4.827 | 4.600 | 3.350 | 4.166 | 4.092 | 4.161 | 4.002 | 4.176 |
| | $^3B_2$ $(\pi \to \pi^\star)$ | 1.854 | 1.734 | 1.834 | 1.769 | 1.662 | 1.785 | 2.232 | 1.758 | 1.745 | 1.805 | 1.733 | 1.780 |
| | $^3B_2$ $(\pi \to \pi^\star)$ | 3.037 | 3.074 | 3.205 | 3.300 | 3.338 | 3.348 | 3.213 | 3.178 | 3.163 | 3.092 | 2.917 | 3.080 |
| | $^3A_1$ $(\pi \to \pi^\star)$ | 3.270 | 3.289 | 3.444 | 3.523 | 3.525 | 3.570 | 3.599 | 3.413 | 3.409 | 3.307 | 3.127 | 3.299 |
| Coumarin | $^1A'$ $(\pi \to \pi^\star)$ | 4.355 | 4.565 | 4.626 | 4.744 | 4.924 | 4.832 | 4.190 | 4.494 | 4.453 | 4.542 | 4.401 | 4.526 |
| | $^1A''$ $(n \to \pi^\star)$ | 4.601 | 4.889 | 5.006 | 5.165 | 5.401 | 5.292 | 4.058 | 4.917 | 4.879 | 4.789 | 4.588 | 4.839 |
| | $^1A'$ $(\pi \to \pi^\star)$ | 4.901 | 5.077 | 5.111 | 5.230 | 5.410 | 5.292 | 4.685 | 4.939 | 4.874 | 5.024 | 4.880 | 5.001 |
| | $^3A'$ $(\pi \to \pi^\star)$ | 3.212 | 3.110 | 3.228 | 3.244 | 3.137 | 3.231 | 3.755 | 3.209 | 3.212 | 3.269 | 3.083 | 3.229 |
| | $^3A'$ $(\pi \to \pi^\star)$ | 4.009 | 3.961 | 4.383 | 4.439 | 4.432 | 4.456 | 4.527 | 4.307 | 4.289 | 3.987 | 3.780 | 3.963 |
| | $^3A''$ $(n \to \pi^\star)$ | 4.336 | 4.510 | 4.667 | 4.788 | 4.925 | 4.894 | 4.041 | 4.639 | 4.622 | 4.503 | 4.245 | 4.536 |
| Cyclazine | $^1A'_2$ $(\pi \to \pi^\star)$ | 1.155 | 1.287 | 1.241 | 1.311 | 1.438 | 1.346 | 0.794 | 1.084 | 1.014 | 1.316 | 1.278 | 1.300 |
| | $^1E'$ $(\pi \to \pi^\star)$ | 3.194 | 3.424 | 3.358 | 3.482 | 3.711 | 3.536 | 2.773 | 3.276 | 3.214 | 3.499 | 3.398 | 3.446 |
| | $^1A''_1$ (Ryd) | 3.151 | 3.471 | 3.498 | 3.463 | 3.903 | 3.729 | 3.374 | 3.566 | 3.637 | 3.742 | 3.534 | 3.353 |
| | $^1E''$ (Ryd) | 3.572 | 3.894 | 3.947 | 3.997 | 4.402 | 4.225 | 3.928 | 4.082 | 4.164 | 4.188 | 4.001 | 3.802 |
| | $^3A'_2$ $(\pi \to \pi^\star)$ | 1.132 | 1.140 | 1.202 | 1.219 | 1.237 | 1.263 | 1.165 | 1.164 | 1.132 | 1.146 | 1.076 | 1.124 |
| | $^3E'$ $(\pi \to \pi^\star)$ | 2.192 | 2.199 | 2.267 | 2.824 | 2.298 | 2.325 | 2.272 | 2.203 | 2.182 | 2.282 | 2.149 | 2.232 |
| | $^3A''_1$ (Ryd) | 3.147 | 3.448 | 3.478 | 3.451 | 3.874 | 3.705 | 3.397 | 3.559 | 3.636 | 3.826 | 3.527 | 3.368 |
| | $^3E''$ (Ryd) | 3.572 | 3.876 | 3.932 | 3.993 | 4.380 | 4.207 | 3.927 | 4.077 | 4.163 | 4.278 | 3.999 | 3.823 |

Table S18: VTEs (in eV) computed with TDA-DFT using the aug-cc-pVTZ basis set.

| Compound | State | B2PLYP | PBE0-DH | PBE-QIDH | $\omega$B2PLYP | RSH-0DH | RSX-QIDH | $\omega$B97X-2 | SOS-$\omega$B88PP86 | SOS-$\omega$PBEPP86 | cLH12ct-SsirPW92 | cLH14t-calPBE | cLH20t |
|---|---|---|---|---|---|---|---|---|---|---|---|---|---|
| Heptazine | $^1A_2'$ $(\pi \rightarrow \pi^\star)$ | 2.794 | 3.122 | 3.059 | 3.199 | 3.500 | 3.307 | 1.958 | 2.853 | 2.773 | 3.168 | 3.033 | 3.130 |
| | $^1A_1''$ $(n \rightarrow \pi^\star)$ | 3.774 | 4.230 | 4.277 | 4.424 | 4.818 | 4.621 | 2.593 | 4.097 | 4.053 | 4.214 | 3.955 | 4.282 |
| | $^1E''$ $(n \rightarrow \pi^\star)$ | 3.862 | 4.259 | 4.300 | 4.460 | 4.804 | 4.623 | 2.744 | 4.141 | 4.091 | 4.252 | 4.019 | 4.307 |
| | $^1E'$ $(\pi \rightarrow \pi^\star)$ | 4.553 | 4.948 | 4.860 | 5.071 | 5.423 | 5.158 | 3.646 | 4.720 | 4.637 | 4.992 | 4.815 | 4.949 |
| | $^3A_2'$ $(\pi \rightarrow \pi^\star)$ | 2.837 | 2.986 | 3.090 | 3.150 | 3.294 | 3.278 | 2.616 | 3.065 | 3.042 | 2.974 | 2.809 | 2.928 |
| | $^3E''(\pi \rightarrow \pi^\star)$ | 3.593 | 3.688 | 3.805 | 3.845 | 3.945 | 3.954 | 3.515 | 3.749 | 3.730 | 3.720 | 3.528 | 3.650 |
| | $^3A_1''$ $(n \rightarrow \pi^\star)$ | 3.757 | 4.111 | 4.220 | 4.335 | 4.641 | 4.521 | 2.863 | 4.109 | 4.087 | 4.120 | 3.839 | 4.189 |
| | $^3E''$ $(n \rightarrow \pi^\star)$ | 3.806 | 4.128 | 4.220 | 4.357 | 4.635 | 4.514 | 2.912 | 4.121 | 4.090 | 4.148 | 3.886 | 4.197 |
| Naphthalimide | $^1B_2$ $(\pi \rightarrow \pi^\star)$ | 4.152 | 4.353 | 4.356 | 4.474 | 4.659 | 4.537 | 3.814 | 4.125 | 4.054 | 4.322 | 4.200 | 4.295 |
| | $^1B_1$ $(n \rightarrow \pi^\star)$ | 3.887 | 4.233 | 4.363 | 4.583 | 4.864 | 4.719 | 3.209 | 4.314 | 4.274 | 4.071 | 3.849 | 4.153 |
| | $^1A_1$ $(\pi \rightarrow \pi^\star)$ | 4.059 | 4.204 | 4.288 | 4.441 | 4.578 | 4.498 | 4.097 | 4.244 | 4.197 | 4.136 | 4.012 | 4.126 |
| | $^1A_2$ $(n \rightarrow \pi^\star)$ | 4.411 | 4.706 | 4.809 | 4.964 | 5.211 | 5.094 | 3.739 | 4.719 | 4.680 | 4.544 | 4.355 | 4.609 |
| | $^3A_1$ $(\pi \rightarrow \pi^\star)$ | 2.762 | 2.680 | 2.804 | 2.880 | 2.748 | 2.833 | 3.280 | 2.788 | 2.786 | 2.803 | 2.629 | 2.774 |
| | $^3B_2$ $(\pi \rightarrow \pi^\star)$ | 3.703 | 3.669 | 3.816 | 3.856 | 3.822 | 3.889 | 4.120 | 3.770 | 3.759 | 3.668 | 3.508 | 3.640 |
| | $^3B_1$ $(n \rightarrow \pi^\star)$ | 3.705 | 3.935 | 4.105 | 4.273 | 4.454 | 4.836 | 3.273 | 4.104 | 4.085 | 3.851 | 3.586 | 3.919 |
| | $^3B_2$ $(\pi \rightarrow \pi^\star)$ | 4.074 | 4.021 | 4.447 | 4.136 | 4.092 | 4.145 | 4.393 | 4.034 | 4.024 | 4.171 | 3.965 | 4.115 |
| | $^3A_2$ $(n \rightarrow \pi^\star)$ | 4.174 | 4.360 | 4.504 | 4.623 | 4.774 | 4.735 | 3.744 | 4.471 | 4.453 | 4.293 | 4.053 | 4.344 |
| Naphthoquinone | $^1B_1$ $(n \rightarrow \pi^\star)$ | 2.865 | 3.050 | 3.158 | 3.311 | 3.469 | 3.391 | 2.399 | 3.126 | 3.087 | 2.876 | 2.767 | 2.960 |
| | $^1A_2$ $(n \rightarrow \pi^\star)$ | 3.079 | 3.294 | 3.386 | 3.534 | 3.715 | 3.622 | 2.600 | 3.330 | 3.290 | 3.166 | 3.036 | 3.236 |
| | $^1A_1$ $(\pi \rightarrow \pi^\star)$ | 3.909 | 4.154 | 4.266 | 4.533 | 4.781 | 4.610 | 3.684 | 4.195 | 4.126 | 3.960 | 3.722 | 3.980 |
| | $^1B_2$ $(\pi \rightarrow \pi^\star)$ | 4.016 | 4.149 | 4.356 | 4.542 | 4.695 | 4.643 | 4.186 | 4.384 | 4.352 | 3.908 | 3.744 | 3.932 |
| | $^1A_2$ $(n \rightarrow \pi^\star)$ | 4.892 | 5.536 | 5.838 | 6.502 | 6.880 | 6.514 | 4.042 | 6.251 | 6.073 | 5.298 | 5.009 | 5.435 |
| | $^1A_1$ $(\pi \rightarrow \pi^\star)$ | 5.409 | 5.683 | 5.713 | 5.931 | 6.210 | 6.025 | 4.980 | 5.610 | 5.550 | 5.647 | 5.484 | 5.611 |
| | $^1B_2$ $(\pi \rightarrow \pi^\star)$ | 5.331 | 5.515 | 5.646 | 5.799 | 5.961 | 5.877 | 5.389 | 5.634 | 5.599 | 5.396 | 5.230 | 5.386 |
| | $^3B_1$ $(n \rightarrow \pi^\star)$ | 2.501 | 2.578 | 2.735 | 2.865 | 2.928 | 2.923 | 2.284 | 2.768 | 2.751 | 2.516 | 2.325 | 2.591 |
| | $^3A_2$ $(n \rightarrow \pi^\star)$ | 2.716 | 2.816 | 2.960 | 3.083 | 3.164 | 3.148 | 2.492 | 2.975 | 2.957 | 2.801 | 2.587 | 2.860 |
| | $^3B_2$ $(\pi \rightarrow \pi^\star)$ | 3.224 | 3.080 | 3.225 | 3.260 | 3.124 | 3.232 | 3.879 | 3.238 | 3.246 | 3.206 | 3.014 | 3.174 |
| | $^3B_2$ $(\pi \rightarrow \pi^\star)$ | 3.337 | 3.241 | 3.424 | 3.465 | 3.363 | 3.464 | 4.013 | 3.443 | 3.450 | 3.281 | 3.075 | 3.257 |
| | $^3A_1$ $(\pi \rightarrow \pi^\star)$ | 3.473 | 3.476 | 3.701 | 3.825 | 3.849 | 3.879 | 3.928 | 3.728 | 3.712 | 3.313 | 3.122 | 3.313 |
| Phenazine | $^1B_{1u}$ $(n \rightarrow \pi^\star)$ | 3.264 | 3.435 | 3.538 | 3.708 | 3.858 | 3.773 | 2.761 | 3.516 | 3.478 | 3.298 | 3.196 | 3.365 |
| | $^1B_{3u}$ $(\pi \rightarrow \pi^\star)$ | 3.534 | 3.651 | 3.767 | 3.972 | 4.093 | 4.015 | 3.661 | 3.776 | 3.725 | 3.543 | 3.419 | 3.547 |
| | $^1B_{2u}$ $(\pi \rightarrow \pi^\star)$ | 3.917 | 4.085 | 4.072 | 4.161 | 4.307 | 4.208 | 3.630 | 3.826 | 3.752 | 4.091 | 3.994 | 4.062 |
| | $^1B_{1g}$ $(\pi \rightarrow \pi^\star)$ | 4.321 | 4.537 | 4.674 | 4.989 | 5.197 | 5.054 | 4.298 | 4.695 | 4.636 | 4.369 | 4.192 | 4.388 |
| | $^1B_{2g}$ $(n \rightarrow \pi^\star)$ | 4.901 | 5.151 | 5.298 | 5.433 | 5.648 | 5.567 | 4.557 | 5.236 | 5.212 | 5.110 | 4.912 | 5.162 |
| | $^1A_u$ $(\pi \rightarrow \pi^\star)$ | 4.901 | 5.318 | 5.345 | 5.621 | 5.983 | 5.745 | 3.636 | 5.279 | 5.224 | 5.221 | 5.017 | 5.282 |
| | $^3B_{3u}$ $(\pi \rightarrow \pi^\star)$ | 2.365 | 2.263 | 2.400 | 2.449 | 2.345 | 2.433 | 2.987 | 2.395 | 2.388 | 2.365 | 2.207 | 2.339 |
| | $^3B_{1u}$ $(n \rightarrow \pi^\star)$ | 2.873 | 2.923 | 3.071 | 3.196 | 3.238 | 3.235 | 2.699 | 3.094 | 3.078 | 2.908 | 2.739 | 2.961 |
| | $^3B_{2u}$ $(\pi \rightarrow \pi^\star)$ | 3.315 | 3.241 | 3.374 | 3.370 | 3.306 | 3.397 | 3.708 | 3.282 | 3.260 | 3.233 | 3.124 | 3.219 |
| | $^3B_{1g}$ $(\pi \rightarrow \pi^\star)$ | 3.514 | 3.422 | 3.541 | 3.577 | 3.476 | 3.557 | 4.045 | 3.505 | 3.503 | 3.549 | 3.357 | 3.524 |
| Phthalimide | $^1B_1$ $(n \rightarrow \pi^\star)$ | 3.941 | 4.193 | 4.292 | 4.448 | 4.666 | 4.560 | 3.344 | 4.219 | 4.178 | 4.075 | 3.906 | 4.113 |
| | $^1A_1$ $(\pi \rightarrow \pi^\star)$ | 4.717 | 4.934 | 4.948 | 5.058 | 5.263 | 5.136 | 4.352 | 4.683 | 4.613 | 4.876 | 4.732 | 4.843 |
| | $^1A_2$ $(n \rightarrow \pi^\star)$ | 4.595 | 4.815 | 4.908 | 5.020 | 5.209 | 5.131 | 4.066 | 4.807 | 4.768 | 4.713 | 4.553 | 4.741 |
| | $^1B_2$ $(\pi \rightarrow \pi^\star)$ | 4.844 | 4.969 | 5.155 | 5.219 | 5.346 | 5.345 | 4.983 | 5.055 | 5.035 | 4.806 | 4.647 | 4.793 |
| | $^1B_2$ $(\pi \rightarrow \pi^\star)$ | 5.797 | 6.086 | 6.102 | 6.247 | 6.514 | 6.341 | 5.236 | 5.972 | 5.922 | 6.064 | 5.875 | 6.028 |
| | $^1A_2$ $(n \rightarrow \pi^\star)$ | 5.373 | 5.985 | 6.334 | 6.830 | 7.238 | 7.086 | 4.958 | 6.552 | 6.572 | 5.730 | 5.395 | 5.858 |
| | $^1A_1$ $(\pi \rightarrow \pi^\star)$ | 6.305 | 6.557 | 6.574 | 6.706 | 6.940 | 6.797 | 5.923 | 6.475 | 6.427 | 6.524 | 6.349 | 6.480 |
| | $^3B_2$ $(\pi \rightarrow \pi^\star)$ | 3.778 | 3.649 | 3.768 | 3.779 | 3.641 | 3.750 | 4.424 | 3.748 | 3.758 | 3.840 | 3.616 | 3.792 |
| | $^3B_1$ $(n \rightarrow \pi^\star)$ | 3.642 | 3.789 | 3.939 | 4.066 | 4.191 | 4.161 | 3.298 | 3.930 | 3.910 | 3.764 | 3.524 | 3.794 |
| | $^3A_1$ $(\pi \rightarrow \pi^\star)$ | 4.217 | 4.199 | 4.356 | 4.402 | 4.408 | 4.451 | 4.531 | 4.291 | 4.276 | 4.151 | 3.968 | 4.114 |
| | $^3B_2$ $(\pi \rightarrow \pi^\star)$ | 4.456 | 4.433 | 4.576 | 4.621 | 4.627 | 4.654 | 4.636 | 4.461 | 4.443 | 4.419 | 4.183 | 4.359 |
| | $^3A_2$ $(n \rightarrow \pi^\star)$ | 4.267 | 4.382 | 4.525 | 4.614 | 4.710 | 4.705 | 3.884 | 4.492 | 4.474 | 4.381 | 4.146 | 4.400 |
| | $^3B_2$ $(\pi \rightarrow \pi^\star)$ | 4.457 | 4.502 | 4.658 | 4.739 | 4.777 | 4.821 | 4.684 | 4.644 | 4.643 | 4.670 | 4.454 | 4.619 |
| Tolan | $^1B_{2u}$ $(\pi \rightarrow \pi^\star)$ | 4.776 | 4.994 | 5.034 | 5.160 | 5.368 | 5.243 | 4.496 | 4.798 | 4.734 | 4.925 | 4.754 | 4.900 |
| | $^1B_{3g}$ $(\pi \rightarrow \pi^\star)$ | 4.808 | 5.026 | 5.061 | 5.188 | 5.393 | 5.267 | 4.506 | 4.813 | 4.746 | 4.957 | 4.789 | 4.937 |
| | $^1B_{1u}$ $(\pi \rightarrow \pi^\star)$ | 4.511 | 4.563 | 4.711 | 4.799 | 4.858 | 4.869 | 4.835 | 4.706 | 4.683 | 4.475 | 4.367 | 4.464 |
| | $^1A_u$ $(\pi \rightarrow \pi^\star)$ | 5.198 | 5.198 | 5.461 | 5.548 | 5.549 | 5.636 | 5.654 | 5.539 | 5.541 | 4.976 | 4.856 | 5.002 |
| | $^1B_{3u}$ (Ryd) | 5.342 | 5.679 | 5.795 | 5.796 | 6.267 | 6.096 | 5.700 | 5.880 | 5.966 | 5.935 | 5.636 | 5.503 |
| | $^3B_{1u}$ $(\pi \rightarrow \pi^\star)$ | 3.212 | 3.097 | 3.249 | 3.297 | 3.179 | 3.280 | 3.856 | 3.255 | 3.262 | 3.217 | 3.019 | 3.193 |
| | $^3A_g$ $(\pi \rightarrow \pi^\star)$ | 4.118 | 3.983 | 4.062 | 4.071 | 3.920 | 4.022 | 4.744 | 4.026 | 4.036 | 4.323 | 4.066 | 4.247 |

### S3.4 BSE/*GW*

Table S19: VTEs (in eV) computed with BSE/$GW$ using the aug-cc-pVTZ basis set.

| Compound | State | BSE/$G_0W_0$@PBE0 | BSE/$G_0W_0$@CAM-B3LYP | BSE/$G_0W_0$@HF | BSE/ev$GW$@PBE0 | BSE/ev$GW$@CAM-B3LYP | BSE/ev$GW$@HF | TDA-BSE/$G_0W_0$@PBE0 | TDA-BSE/$G_0W_0$@CAM-B3LYP | TDA-BSE/$G_0W_0$@HF | TDA-BSE/ev$GW$@PBE0 | TDA-BSE/ev$GW$@CAM-B3LYP | TDA-BSE/ev$GW$@HF |
|---|---|---|---|---|---|---|---|---|---|---|---|---|---|
| Anthracene | $^1B_{1u}$ ($\pi \to \pi^\star$) | 2.930 | 3.237 | 3.717 | 3.211 | 3.305 | 3.656 | 3.214 | 3.517 | 3.962 | 3.487 | 3.582 | 3.903 |
| | $^1B_{2u}$ ($\pi \to \pi^\star$) | 3.467 | 3.742 | 4.429 | 3.719 | 3.798 | 4.369 | 3.498 | 3.779 | 4.479 | 3.760 | 3.838 | 4.418 |
| | $^1B_{3g}$ ($\pi \to \pi^\star$) | 4.443 | 4.789 | 5.429 | 4.797 | 4.872 | 5.344 | 4.666 | 4.927 | 5.592 | 4.929 | 5.042 | 5.502 |
| | $^1B_{2g}$ (Ryd) | 4.597 | 4.883 | 5.772 | 4.802 | 4.930 | 5.748 | 4.598 | 4.884 | 5.773 | 4.804 | 4.932 | 5.749 |
| | $^1B_{1u}$ ($\pi \to \pi^\star$) | 4.692 | 5.071 | 5.976 | 5.023 | 5.135 | 5.940 | 4.737 | 5.114 | 5.988 | 5.085 | 5.181 | 5.952 |
| | $^1B_{3g}$ ($\pi \to \pi^\star$) | 4.410 | 4.923 | 6.113 | 4.924 | 5.041 | 6.043 | 4.442 | 5.043 | 6.165 | 5.048 | 5.129 | 6.100 |
| | $^1A_g$ ($\pi \to \pi^\star$) | 4.941 | 5.430 | 6.495 | 5.370 | 5.516 | 6.415 | 4.964 | 5.457 | 6.533 | 5.397 | 5.544 | 6.455 |
| | $^1B_{3u}$ (Ryd) | 4.829 | 5.152 | 5.846 | 5.026 | 5.198 | 5.820 | 4.831 | 5.153 | 5.847 | 5.028 | 5.199 | 5.820 |
| | $^1A_u$ (Ryd) | 4.913 | 5.230 | 5.491 | 5.123 | 5.279 | 5.466 | 4.915 | 5.231 | 5.492 | 5.124 | 5.280 | 5.467 |
| | $^1B_{2u}$ ($\pi \to \pi^\star$) | 4.764 | 5.013 | 5.655 | 5.056 | 5.080 | 5.597 | 5.218 | 5.434 | 5.959 | 5.496 | 5.499 | 5.900 |
| | $^3B_{1u}$ ($\pi \to \pi^\star$) | 1.537 | 1.707 | 2.300 | 1.605 | 1.711 | 2.288 | 1.771 | 1.988 | 2.519 | 1.944 | 2.025 | 2.484 |
| | $^3B_{3g}$ ($\pi \to \pi^\star$) | 2.808 | 3.072 | 3.947 | 2.997 | 3.100 | 3.921 | 2.970 | 3.261 | 4.099 | 3.215 | 3.306 | 4.059 |
| | $^3B_{2u}$ ($\pi \to \pi^\star$) | 3.035 | 3.297 | 3.831 | 3.262 | 3.345 | 3.771 | 3.077 | 3.343 | 3.886 | 3.316 | 3.394 | 3.823 |
| Anthraquinone | $^1B_{1g}$ ($n \to \pi^\star$) | 2.626 | 3.065 | 4.075 | 3.104 | 3.184 | 3.825 | 2.664 | 3.102 | 4.106 | 3.143 | 3.222 | 3.855 |
| | $^1A_u$ ($n \to \pi^\star$) | 2.843 | 3.298 | 4.260 | 3.351 | 3.421 | 3.992 | 2.879 | 3.331 | 4.288 | 3.386 | 3.455 | 4.019 |
| | $^1A_g$ ($\pi \to \pi^\star$) | 3.722 | 4.078 | 4.630 | 4.121 | 4.176 | 4.511 | 3.823 | 4.181 | 4.740 | 4.225 | 4.279 | 4.619 |
| | $^1B_{2u}$ ($\pi \to \pi^\star$) | 3.743 | 4.093 | 4.668 | 4.119 | 4.184 | 4.558 | 3.809 | 4.161 | 4.745 | 4.187 | 4.253 | 4.633 |
| | $^1B_{3g}$ ($\pi \to \pi^\star$) | 3.631 | 3.991 | 4.586 | 3.973 | 4.076 | 4.480 | 3.731 | 4.096 | 4.698 | 4.072 | 4.180 | 4.593 |
| | $^1B_{1u}$ ($\pi \to \pi^\star$) | 4.406 | 4.767 | 5.260 | 4.816 | 4.864 | 5.137 | 4.659 | 5.014 | 5.457 | 5.069 | 5.111 | 5.336 |
| | $^1B_{2u}$ ($\pi \to \pi^\star$) | 4.844 | 5.195 | 5.936 | 5.233 | 5.287 | 5.825 | 4.990 | 5.349 | 6.100 | 5.388 | 5.444 | 5.988 |
| | $^3B_{1g}$ ($n \to \pi^\star$) | 2.128 | 2.557 | 3.630 | 2.576 | 2.666 | 3.395 | 2.170 | 2.601 | 3.669 | 2.626 | 2.713 | 3.430 |
| | $^3A_u$ ($n \to \pi^\star$) | 2.330 | 2.773 | 3.808 | 2.806 | 2.887 | 3.556 | 2.370 | 2.817 | 3.846 | 2.854 | 2.933 | 3.590 |
| | $^3B_{1u}$ ($\pi \to \pi^\star$) | 2.548 | 2.783 | 3.500 | 2.716 | 2.806 | 3.463 | 2.791 | 3.077 | 3.746 | 3.051 | 3.131 | 3.673 |
| | $^3B_{3g}$ ($\pi \to \pi^\star$) | 2.714 | 2.940 | 3.515 | 2.906 | 2.974 | 3.470 | 2.890 | 3.161 | 3.706 | 3.157 | 3.221 | 3.633 |
| | $^3A_g$ ($\pi \to \pi^\star$) | 2.810 | 3.115 | 3.706 | 3.108 | 3.183 | 3.622 | 2.886 | 3.202 | 3.778 | 3.209 | 3.277 | 3.686 |
| Aza-BODIPY | $^1B_2$ ($\pi \to \pi^\star$) | 2.078 | 2.319 | 2.685 | 2.355 | 2.392 | 2.621 | 2.571 | 2.833 | 3.151 | 2.861 | 2.894 | 3.092 |
| | $^1B_2$ ($\pi \to \pi^\star$) | 2.754 | 3.159 | 3.679 | 3.230 | 3.284 | 3.545 | 3.247 | 3.475 | 3.904 | 3.562 | 3.574 | 3.786 |
| | $^1A_1$ ($\pi \to \pi^\star$) | 2.896 | 3.380 | 3.951 | 3.437 | 3.518 | 3.812 | 3.044 | 3.531 | 4.110 | 3.581 | 3.670 | 3.973 |
| | $^1B_1$ ($n \to \pi^\star$) | 3.260 | 3.626 | 4.502 | 3.666 | 3.740 | 4.287 | 3.325 | 3.691 | 4.551 | 3.733 | 3.805 | 4.335 |
| | $^3B_2$ ($\pi \to \pi^\star$) | 0.296 | 0.315 | 0.663 | | 0.173 | 0.672 | 0.622 | 0.767 | 1.056 | 0.726 | 0.793 | 1.043 |
| | $^3B_2$ ($\pi \to \pi^\star$) | 1.926 | 2.249 | 2.731 | 2.283 | 2.337 | 2.627 | 2.008 | 2.351 | 2.828 | 2.399 | 2.449 | 2.779 |
| | $^3A_1$ ($\pi \to \pi^\star$) | 2.125 | 2.493 | 2.983 | 2.541 | 2.593 | 2.878 | 2.200 | 2.588 | 3.075 | 2.647 | 2.698 | 3.030 |
| | $^3B_1$ ($n \to \pi^\star$) | 2.650 | 2.978 | 3.921 | 3.000 | 3.075 | 3.728 | 2.695 | 3.031 | 3.969 | 3.059 | 3.132 | 3.828 |
| Azobenzene | $^1B_g$ ($n \to \pi^\star$) | 2.238 | 2.624 | 3.715 | 2.638 | 2.717 | 3.553 | 2.353 | 2.729 | 3.784 | 2.744 | 2.821 | 3.623 |
| | $^1B_u$ ($\pi \to \pi^\star$) | 3.519 | 3.832 | 4.390 | 3.863 | 3.914 | 4.320 | 3.762 | 4.053 | 4.561 | 4.091 | 4.132 | 4.493 |
| | $^1A_g$ ($\pi \to \pi^\star$) | 3.955 | 4.372 | 5.136 | 4.402 | 4.475 | 5.052 | 4.011 | 4.428 | 5.222 | 4.459 | 4.532 | 5.139 |
| | $^1B_u$ ($\pi \to \pi^\star$) | 3.955 | 4.360 | 5.132 | 4.387 | 4.463 | 5.048 | 3.999 | 4.417 | 5.219 | 4.443 | 4.520 | 5.136 |
| | $^1A_g$ ($\pi \to \pi^\star$) | 4.611 | 5.073 | 5.779 | 5.091 | 5.179 | 5.695 | 4.776 | 5.251 | 5.963 | 5.263 | 5.359 | 5.879 |
| | $^3B_g$ ($n \to \pi^\star$) | 1.422 | 1.764 | 2.936 | 1.760 | 1.837 | 2.896 | 1.499 | 1.847 | 3.002 | 1.851 | 1.924 | 2.857 |
| | $^3B_u$ ($\pi \to \pi^\star$) | 1.973 | 2.201 | 2.941 | 2.119 | 2.221 | 2.978 | 2.210 | 2.483 | 3.161 | 2.448 | 2.535 | 3.118 |
| | $^3A_g$ ($\pi \to \pi^\star$) | 3.032 | 3.315 | 4.172 | 3.268 | 3.341 | 4.256 | 3.222 | 3.560 | 4.328 | 3.548 | 3.620 | 4.272 |
| | $^3B_u$ ($\pi \to \pi^\star$) | 3.315 | 3.680 | 4.368 | 3.690 | 3.760 | 4.382 | 3.363 | 3.739 | 4.421 | 3.760 | 3.828 | 4.349 |
| | $^3A_g$ ($\pi \to \pi^\star$) | 3.365 | 3.737 | 4.432 | 3.758 | 3.823 | 4.444 | 3.409 | 3.787 | 4.493 | 3.812 | 3.876 | 4.425 |
| BODIPY | $^1B_2$ ($\pi \to \pi^\star$) | 2.458 | 2.675 | 3.017 | 2.730 | 2.748 | 2.931 | 2.869 | 3.061 | 3.335 | 3.121 | 3.122 | 3.256 |
| | $^1B_2$ ($\pi \to \pi^\star$) | 3.156 | 3.555 | 4.081 | 3.632 | 3.684 | 3.919 | 3.445 | 3.777 | 4.266 | 3.857 | 3.897 | 4.110 |
| | $^1A_1$ ($\pi \to \pi^\star$) | 3.311 | 3.776 | 4.351 | 3.844 | 3.916 | 4.185 | 3.460 | 3.931 | 4.511 | 3.990 | 4.072 | 4.346 |
| | $^3B_2$ ($\pi \to \pi^\star$) | 0.935 | 1.074 | 1.419 | 0.993 | 1.087 | 1.381 | 1.098 | 1.281 | 1.629 | 1.260 | 1.326 | 1.568 |
| | $^3B_2$ ($\pi \to \pi^\star$) | 2.287 | 2.589 | 3.087 | 2.626 | 2.679 | 2.966 | 2.372 | 2.695 | 3.188 | 2.749 | 2.795 | 3.054 |
| | $^3A_1$ ($\pi \to \pi^\star$) | 2.473 | 2.811 | 3.334 | 2.850 | 2.908 | 3.213 | 2.556 | 2.915 | 3.430 | 2.972 | 3.024 | 3.296 |
| Coumarin | $^1A'$ ($\pi \to \pi^\star$) | 3.846 | 4.164 | 4.778 | 4.196 | 4.262 | 4.699 | 4.020 | 4.340 | 4.973 | 4.375 | 4.440 | 4.894 |
| | $^1A''$ ($n \to \pi^\star$) | 4.059 | 4.532 | 5.691 | 4.619 | 4.697 | 5.467 | 4.088 | 4.561 | 5.716 | 4.650 | 4.727 | 5.490 |
| | $^1A'$ ($\pi \to \pi^\star$) | 4.352 | 4.671 | 5.308 | 4.726 | 4.774 | 5.225 | 4.537 | 4.844 | 5.470 | 4.898 | 4.944 | 5.391 |
| | $^3A'$ ($\pi \to \pi^\star$) | 2.382 | 2.589 | 3.199 | 2.542 | 2.621 | 3.170 | 2.568 | 2.814 | 3.401 | 2.805 | 2.875 | 3.351 |
| | $^3A'$ ($\pi \to \pi^\star$) | 3.220 | 3.486 | 4.235 | 3.438 | 3.534 | 4.171 | 3.353 | 3.645 | 4.310 | 3.641 | 3.722 | 4.241 |
| | $^3A''$ ($n \to \pi^\star$) | 3.591 | 4.052 | 5.310 | 4.110 | 4.203 | 5.099 | 3.630 | 4.096 | 5.345 | 4.161 | 4.252 | 5.130 |

Table S20: VTEs (in eV) computed with BSE/$GW$ using the aug-cc-pVTZ basis set.

| Compound | State | BSE/$G_0W_0$@PBE0 | BSE/$G_0W_0$@CAM-B3LYP | BSE/$G_0W_0$@HF | BSE/ev$GW$@PBE0 | BSE/ev$GW$@CAM-B3LYP | BSE/ev$GW$@HF | TDA-BSE/$G_0W_0$@PBE0 | TDA-BSE/$G_0W_0$@CAM-B3LYP | TDA-BSE/$G_0W_0$@HF | TDA-BSE/ev$GW$@PBE0 | TDA-BSE/ev$GW$@CAM-B3LYP | TDA-BSE/ev$GW$@HF |
|---|---|---|---|---|---|---|---|---|---|---|---|---|---|
| Cyclazine | $^1A_2'$ ($\pi \rightarrow \pi^\star$) | 0.673 | 0.883 | 1.360 | 0.881 | 0.934 | 1.314 | 0.713 | 0.925 | 1.396 | 0.925 | 0.977 | 1.349 |
| | $^1E'$ ($\pi \rightarrow \pi^\star$) | 2.617 | 2.867 | 4.084 | 2.910 | 2.936 | 4.041 | 2.890 | 3.098 | 4.207 | 3.153 | 3.167 | 4.162 |
| | $^1A_1''$ (Ryd) | 2.862 | 3.116 | 3.777 | 3.020 | 3.153 | 3.749 | 2.864 | 3.118 | 3.777 | 3.022 | 3.155 | 3.750 |
| | $^1E''$ (Ryd) | 3.360 | 3.633 | 4.230 | 3.513 | 3.669 | 4.203 | 3.362 | 3.634 | 4.230 | 3.515 | 3.670 | 4.203 |
| | $^3A_2'$ ($\pi \rightarrow \pi^\star$) | 0.446 | 0.635 | 1.101 | 0.622 | 0.679 | 1.061 | 0.495 | 0.696 | 1.159 | 0.693 | 0.745 | 1.114 |
| | $^3E'$ ($\pi \rightarrow \pi^\star$) | 1.439 | 1.648 | 2.981 | 1.592 | 1.679 | 2.958 | 1.550 | 1.778 | 3.064 | 1.752 | 1.822 | 3.035 |
| | $^3A_1''$ (Ryd) | 2.804 | 3.063 | 3.741 | 2.957 | 3.099 | 3.714 | 2.807 | 3.066 | 3.742 | 2.962 | 3.102 | 3.716 |
| | $^3E''$ (Ryd) | 3.313 | 3.593 | 4.210 | 3.462 | 3.629 | 4.183 | 3.316 | 3.596 | 4.211 | 3.465 | 3.632 | 4.184 |
| Heptazine | $^1A_2'$ ($\pi \rightarrow \pi^\star$) | 2.408 | 2.679 | 3.354 | 2.781 | 2.783 | 3.228 | 2.444 | 2.716 | 3.389 | 2.821 | 2.822 | 3.261 |
| | $^1A_1''$ ($n \rightarrow \pi^\star$) | 3.426 | 3.839 | 4.739 | 4.025 | 4.014 | 4.510 | 3.437 | 3.850 | 4.750 | 4.038 | 4.027 | 4.520 |
| | $^1E''$ ($n \rightarrow \pi^\star$) | 3.534 | 3.933 | 4.796 | 4.101 | 4.098 | 4.578 | 3.546 | 3.945 | 4.807 | 4.114 | 4.110 | 4.588 |
| | $^1E'$ ($\pi \rightarrow \pi^\star$) | 4.066 | 4.389 | 5.366 | 4.500 | 4.506 | 5.236 | 4.284 | 4.609 | 5.542 | 4.721 | 4.728 | 5.410 |
| | $^3A_2'$ ($\pi \rightarrow \pi^\star$) | 2.152 | 2.412 | 3.060 | 2.502 | 2.508 | 2.942 | 2.189 | 2.455 | 3.106 | 2.550 | 2.555 | 2.983 |
| | $^3E''$($\pi \rightarrow \pi^\star$) | 2.826 | 3.091 | 4.172 | 3.141 | 3.172 | 4.073 | 2.914 | 3.190 | 4.241 | 3.256 | 3.280 | 4.137 |
| | $^3A_1''$ ($n \rightarrow \pi^\star$) | 3.272 | 3.677 | 4.594 | 3.845 | 3.845 | 4.370 | 3.288 | 3.696 | 4.612 | 3.866 | 3.865 | 4.386 |
| | $^3E''$ ($n \rightarrow \pi^\star$) | 3.360 | 3.755 | 4.635 | 3.910 | 3.914 | 4.421 | 3.378 | 3.776 | 4.655 | 3.933 | 3.937 | 4.439 |
| Naphthalimide | $^1B_2$ ($\pi \rightarrow \pi^\star$) | 3.699 | 3.990 | 4.550 | 4.009 | 4.064 | 4.472 | 3.758 | 4.053 | 4.636 | 4.075 | 4.129 | 4.556 |
| | $^1B_1$ ($n \rightarrow \pi^\star$) | 3.504 | 3.996 | 5.044 | 4.084 | 4.155 | 4.772 | 3.527 | 4.019 | 5.061 | 4.109 | 4.179 | 4.788 |
| | $^1A_1$ ($\pi \rightarrow \pi^\star$) | 3.454 | 3.759 | 4.217 | 3.772 | 3.841 | 4.132 | 3.706 | 4.004 | 4.443 | 4.019 | 4.084 | 4.360 |
| | $^1A_2$ ($n \rightarrow \pi^\star$) | 3.934 | 4.424 | 5.582 | 4.494 | 4.575 | 5.326 | 3.959 | 4.448 | 5.601 | 4.520 | 4.600 | 5.345 |
| | $^3A_1$ ($\pi \rightarrow \pi^\star$) | 2.033 | 2.224 | 2.751 | 2.161 | 2.246 | 2.720 | 2.232 | 2.466 | 2.957 | 2.443 | 2.516 | 2.902 |
| | $^3B_2$ ($\pi \rightarrow \pi^\star$) | 2.976 | 3.237 | 3.708 | 3.215 | 3.291 | 3.648 | 3.048 | 3.317 | 3.778 | 3.316 | 3.379 | 3.711 |
| | $^3B_1$ ($n \rightarrow \pi^\star$) | 3.116 | 3.596 | 4.762 | 3.658 | 3.743 | 4.503 | 3.151 | 3.634 | 4.789 | 3.702 | 3.784 | 4.529 |
| | $^3B_2$ ($\pi \rightarrow \pi^\star$) | 3.286 | 3.560 | 4.424 | 3.545 | 3.611 | 4.379 | 3.405 | 3.702 | 4.561 | 3.694 | 3.764 | 4.502 |
| | $^3A_2$ ($n \rightarrow \pi^\star$) | 3.504 | 3.985 | 5.265 | 4.029 | 4.125 | 5.023 | 3.537 | 4.021 | 5.292 | 4.070 | 4.163 | 5.049 |
| Naphthoquinone | $^1B_1$ ($n \rightarrow \pi^\star$) | 2.388 | 2.836 | 3.839 | 2.901 | 2.982 | 3.638 | 2.432 | 2.877 | 3.872 | 2.944 | 3.024 | 3.670 |
| | $^1A_2$ ($n \rightarrow \pi^\star$) | 2.556 | 3.030 | 3.973 | 3.117 | 3.187 | 3.751 | 2.596 | 3.067 | 4.003 | 3.157 | 3.226 | 3.781 |
| | $^1A_1$ ($\pi \rightarrow \pi^\star$) | 3.587 | 3.947 | 4.499 | 4.011 | 4.068 | 4.415 | 3.677 | 4.038 | 4.610 | 4.101 | 4.158 | 4.525 |
| | $^1B_2$ ($\pi \rightarrow \pi^\star$) | 3.528 | 3.922 | 4.499 | 3.908 | 4.032 | 4.418 | 3.646 | 4.042 | 4.631 | 4.021 | 4.151 | 4.552 |
| | $^1A_2$ ($n \rightarrow \pi^\star$) | 4.718 | 5.396 | 7.187 | 5.522 | 5.639 | 6.959 | 4.726 | 5.403 | 7.195 | 5.530 | 5.646 | 6.965 |
| | $^1A_1$ ($\pi \rightarrow \pi^\star$) | 4.944 | 5.313 | 6.637 | 5.342 | 5.422 | 6.578 | 5.036 | 5.416 | 6.732 | 5.443 | 5.529 | 6.671 |
| | $^1B_2$ ($\pi \rightarrow \pi^\star$) | 4.711 | 5.100 | 5.652 | 5.173 | 5.229 | 5.554 | 5.086 | 5.474 | 5.984 | 5.541 | 5.599 | 5.890 |
| | $^3B_1$ ($n \rightarrow \pi^\star$) | 1.863 | 2.298 | 3.364 | 2.339 | 2.431 | 3.174 | 1.908 | 2.346 | 3.406 | 2.394 | 2.482 | 3.212 |
| | $^3A_2$ ($n \rightarrow \pi^\star$) | 2.022 | 2.481 | 3.498 | 2.541 | 2.624 | 3.289 | 2.065 | 2.528 | 3.539 | 2.596 | 2.675 | 3.326 |
| | $^3B_2$ ($\pi \rightarrow \pi^\star$) | 2.315 | 2.588 | 3.320 | 2.484 | 2.614 | 3.289 | 2.552 | 2.878 | 3.526 | 2.826 | 2.945 | 3.470 |
| | $^3B_2$ ($\pi \rightarrow \pi^\star$) | 2.608 | 2.854 | 3.432 | 2.820 | 2.903 | 3.394 | 2.775 | 3.051 | 3.626 | 3.060 | 3.127 | 3.572 |
| | $^3A_1$ ($\pi \rightarrow \pi^\star$) | 2.854 | 3.160 | 3.681 | 3.189 | 3.249 | 3.616 | 2.914 | 3.230 | 3.744 | 3.272 | 3.328 | 3.673 |
| Phenazine | $^1B_{1u}$ ($n \rightarrow \pi^\star$) | 2.821 | 3.200 | 4.106 | 3.228 | 3.301 | 3.894 | 2.873 | 3.251 | 4.143 | 3.281 | 3.353 | 3.931 |
| | $^1B_{3u}$ ($\pi \rightarrow \pi^\star$) | 2.887 | 3.229 | 3.707 | 3.201 | 3.306 | 3.629 | 3.132 | 3.476 | 3.937 | 3.441 | 3.552 | 3.861 |
| | $^1B_{2u}$ ($\pi \rightarrow \pi^\star$) | 3.396 | 3.669 | 4.208 | 3.651 | 3.726 | 4.139 | 3.505 | 3.782 | 4.359 | 3.770 | 3.842 | 4.289 |
| | $^1B_{1g}$ ($\pi \rightarrow \pi^\star$) | 3.768 | 4.206 | 4.767 | 4.199 | 4.310 | 4.675 | 3.873 | 4.322 | 4.895 | 4.310 | 4.429 | 4.802 |
| | $^1B_{2g}$ ($n \rightarrow \pi^\star$) | 4.286 | 4.828 | 5.820 | 4.890 | 4.962 | 5.546 | 4.350 | 4.891 | 5.868 | 4.956 | 5.026 | 5.594 |
| | $^1A_u$ ($\pi \rightarrow \pi^\star$) | 4.562 | 4.999 | 6.418 | 5.074 | 5.124 | 6.186 | 4.568 | 5.005 | 6.426 | 5.081 | 5.132 | 6.193 |
| | $^3B_{3u}$ ($\pi \rightarrow \pi^\star$) | 1.614 | 1.790 | 2.321 | 1.723 | 1.804 | 2.302 | 1.837 | 2.068 | 2.302 | 2.044 | 2.114 | 2.506 |
| | $^3B_{1u}$ ($n \rightarrow \pi^\star$) | 2.318 | 2.671 | 3.650 | 2.678 | 2.760 | 3.455 | 2.358 | 2.716 | 3.455 | 2.729 | 2.808 | 3.491 |
| | $^3B_{2u}$ ($\pi \rightarrow \pi^\star$) | 2.505 | 2.747 | 3.151 | 2.697 | 2.787 | 3.100 | 2.572 | 2.825 | 3.100 | 2.787 | 2.872 | 3.177 |
| | $^3B_{1g}$ ($\pi \rightarrow \pi^\star$) | 2.684 | 2.951 | 3.613 | 2.918 | 2.992 | 3.572 | 2.825 | 3.125 | 3.572 | 3.112 | 3.184 | 3.696 |

Table S21: VTEs (in eV) computed with BSE/$GW$ using the aug-cc-pVTZ basis set.

| Compound | State | BSE/$G_0W_0$@PBE0 | BSE/$G_0W_0$@CAM-B3LYP | BSE/$G_0W_0$@HF | BSE/ev$GW$@PBE0 | BSE/ev$GW$@CAM-B3LYP | BSE/ev$GW$@HF | TDA-BSE/$G_0W_0$@PBE0 | TDA-BSE/$G_0W_0$@CAM-B3LYP | TDA-BSE/$G_0W_0$@HF | TDA-BSE/ev$GW$@PBE0 | TDA-BSE/ev$GW$@CAM-B3LYP | TDA-BSE/ev$GW$@HF |
|---|---|---|---|---|---|---|---|---|---|---|---|---|---|
| Phthalimide | $^1B_1$ ($n \rightarrow \pi^\star$) | 3.488 | 3.908 | 4.921 | 3.997 | 4.069 | 4.710 | 3.519 | 3.939 | 4.948 | 4.031 | 4.101 | 4.737 |
| | $^1A_1$ ($\pi \rightarrow \pi^\star$) | 4.288 | 4.581 | 5.222 | 4.636 | 4.683 | 5.151 | 4.346 | 4.641 | 5.325 | 4.699 | 4.744 | 5.255 |
| | $^1A_2$ ($n \rightarrow \pi^\star$) | 4.065 | 4.506 | 5.590 | 4.578 | 4.665 | 5.383 | 4.095 | 4.535 | 5.617 | 4.609 | 4.695 | 5.409 |
| | $^1B_2$ ($\pi \rightarrow \pi^\star$) | 4.232 | 4.588 | 5.328 | 4.574 | 4.690 | 5.250 | 4.355 | 4.718 | 5.500 | 4.697 | 4.820 | 5.419 |
| | $^1B_2$ ($\pi \rightarrow \pi^\star$) | 5.280 | 5.637 | 6.246 | 5.765 | 5.783 | 6.077 | 5.553 | 5.900 | 6.436 | 6.028 | 6.041 | 6.276 |
| | $^1A_2$ ($n \rightarrow \pi^\star$) | 5.299 | 5.912 | 7.319 | 6.087 | 6.168 | 7.076 | 5.302 | 5.916 | 7.326 | 6.091 | 6.172 | 7.082 |
| | $^1A_1$ ($\pi \rightarrow \pi^\star$) | 5.594 | 5.910 | 6.951 | 5.964 | 6.017 | 6.891 | 5.959 | 6.286 | 7.270 | 6.335 | 6.393 | 7.205 |
| | $^3B_2$ ($\pi \rightarrow \pi^\star$) | 3.011 | 3.173 | 3.751 | 3.154 | 3.199 | 3.727 | 3.243 | 3.455 | 3.974 | 3.483 | 3.518 | 3.926 |
| | $^3B_1$ ($n \rightarrow \pi^\star$) | 3.007 | 3.423 | 4.517 | 3.482 | 3.573 | 4.318 | 3.049 | 3.469 | 4.555 | 3.535 | 3.622 | 4.352 |
| | $^3A_1$ ($\pi \rightarrow \pi^\star$) | 3.521 | 3.786 | 4.244 | 3.814 | 3.870 | 4.186 | 3.574 | 3.845 | 4.308 | 3.884 | 3.935 | 4.246 |
| | $^3B_2$ ($\pi \rightarrow \pi^\star$) | 3.458 | 3.842 | 5.119 | 3.800 | 3.941 | 5.093 | 3.587 | 3.980 | 5.233 | 3.966 | 4.090 | 5.202 |
| | $^3A_2$ ($n \rightarrow \pi^\star$) | 3.557 | 3.994 | 5.156 | 4.036 | 4.142 | 4.960 | 3.594 | 4.035 | 5.191 | 4.083 | 4.186 | 4.992 |
| | $^3B_2$ ($\pi \rightarrow \pi^\star$) | 3.797 | 4.059 | 4.853 | 4.071 | 4.135 | 4.723 | 3.877 | 4.149 | 4.967 | 4.167 | 4.234 | 4.825 |
| Tolan | $^1B_{2u}$ ($\pi \rightarrow \pi^\star$) | 4.356 | 4.698 | 5.691 | 4.710 | 4.781 | 5.643 | 4.383 | 4.729 | 5.731 | 4.744 | 4.815 | 5.683 |
| | $^1B_{3g}$ ($\pi \rightarrow \pi^\star$) | 4.379 | 4.724 | 5.718 | 4.735 | 4.808 | 5.669 | 4.407 | 4.756 | 5.763 | 4.770 | 4.843 | 5.714 |
| | $^1B_{1u}$ ($\pi \rightarrow \pi^\star$) | 4.034 | 4.311 | 4.884 | 4.316 | 4.383 | 4.837 | 4.215 | 4.483 | 5.031 | 4.483 | 4.552 | 4.986 |
| | $^1A_u$ ($\pi \rightarrow \pi^\star$) | 4.750 | 5.117 | 5.928 | 5.099 | 5.219 | 5.851 | 4.758 | 5.128 | 5.938 | 5.112 | 5.231 | 5.860 |
| | $^1B_{3u}$ (Ryd) | 5.073 | 5.416 | 6.151 | 5.304 | 5.477 | 6.120 | 5.075 | 5.418 | 6.152 | 5.307 | 5.479 | 6.121 |
| | $^3B_{1u}$ ($\pi \rightarrow \pi^\star$) | 2.456 | 2.680 | 3.487 | 2.563 | 2.694 | 3.473 | 2.699 | 2.958 | 3.681 | 2.898 | 3.003 | 3.652 |
| | $^3A_g$ ($\pi \rightarrow \pi^\star$) | 3.229 | 3.453 | 4.558 | 3.370 | 3.463 | 4.553 | 3.481 | 3.753 | 4.778 | 3.712 | 3.795 | 4.754 |

# S4 Additional wavefunction analyses

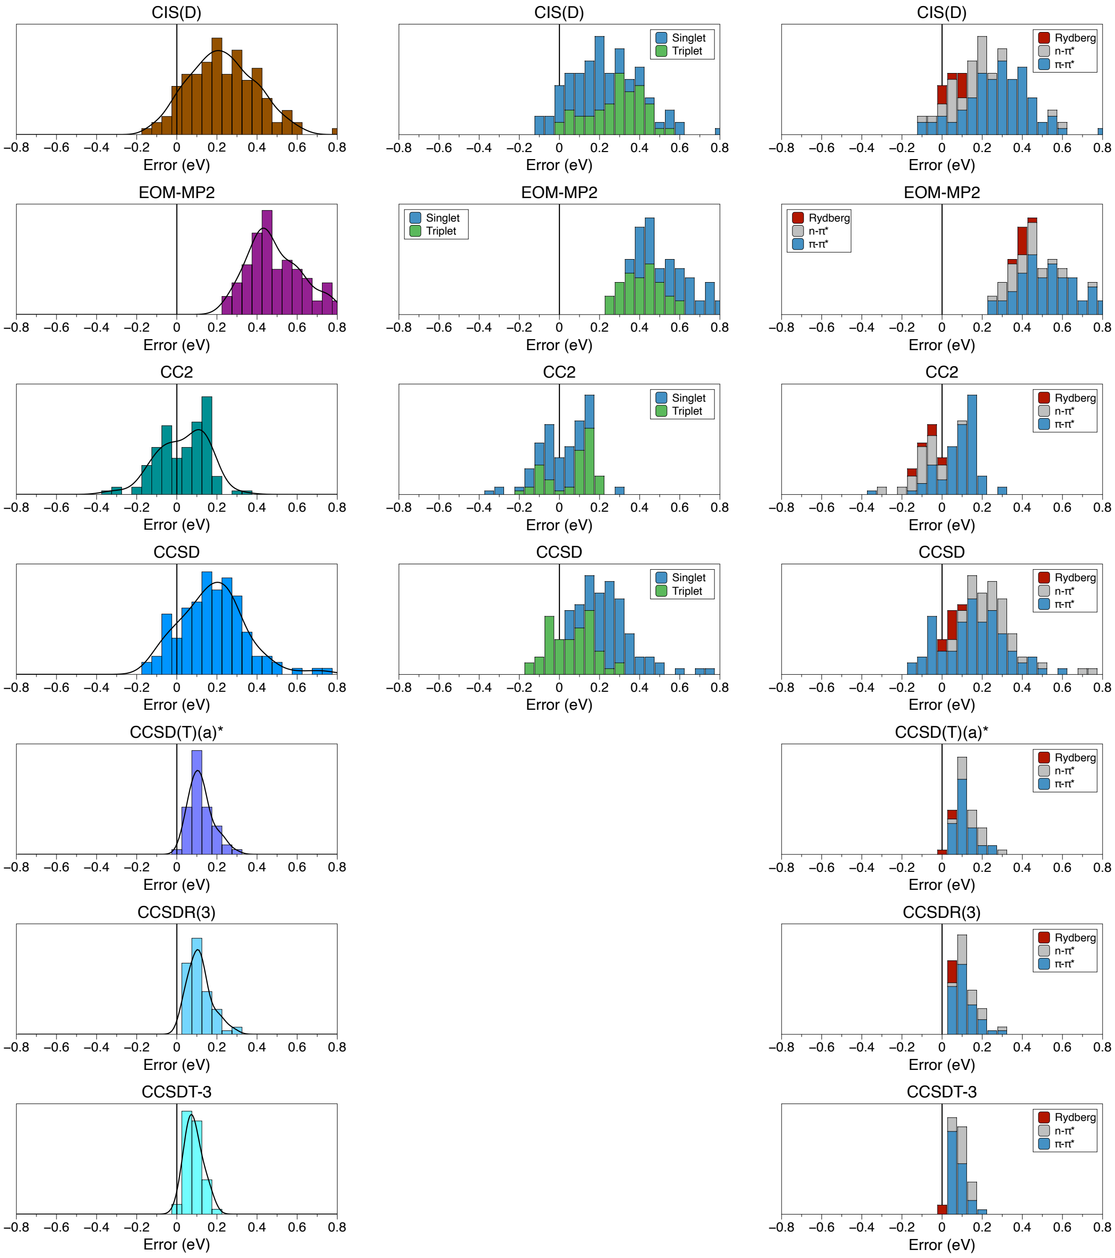


Figure S1: Histograms of the errors as compared to the TBEs for wave function methods considered in the present work. The left panel is equivalent to the histograms given in Figure 3 of the main text. The central panel shows the distribution for the singlet and triplet, whereas the right panel provides the error according to the nature of the ES. For the methods for which only singlet have been computed, the central panel has been omitted.

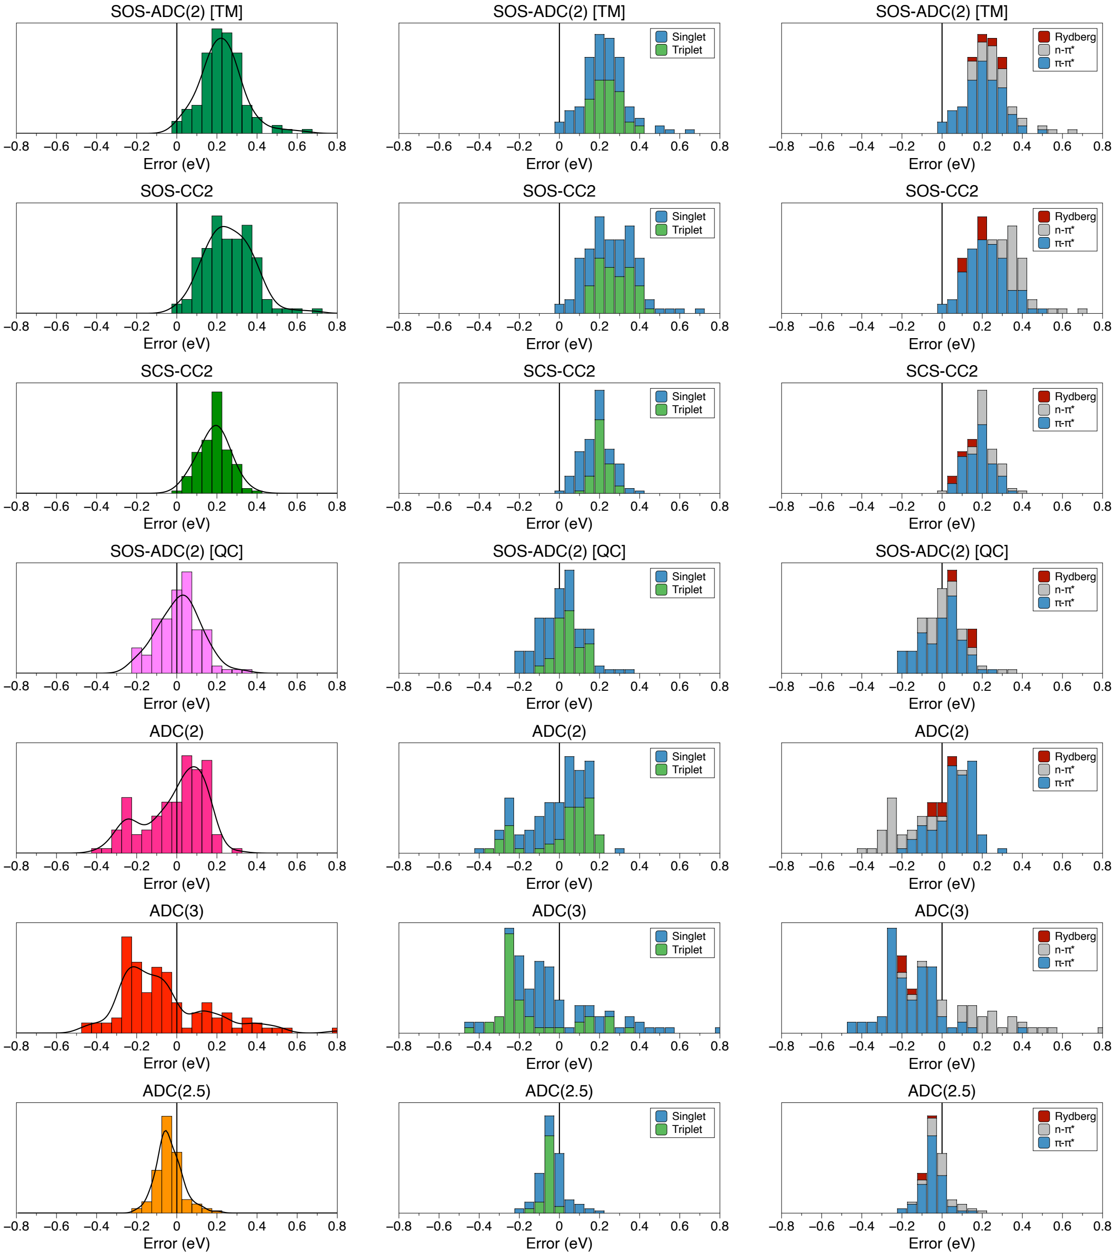


Figure S2: Error patterns for wavefunction approaches. See caption of Fig. S1 for more details.

# S5 Additional TD-DFT data and analyses

## S5.1 Gauge-Invariance

Table S22: Mean variation when including gauge-invariance corrections. All values are in eV.

| | TDA | | | TD-DFT | | |
|---|---|---|---|---|---|---|
| | M06 | M06-2X | M06-SX | M06 | M06-2X | M06-SX |
| All | 0.02 | 0.07 | -0.01 | 0.02 | 0.07 | -0.01 |
| $\pi \rightarrow \pi^\star$ | 0.02 | 0.03 | -0.01 | 0.02 | 0.03 | -0.01 |
| $n \rightarrow \pi^\star$ | 0.01 | 0.17 | -0.02 | 0.01 | 0.18 | -0.02 |
| Rydberg | 0.05 | 0.04 | -0.01 | 0.05 | 0.04 | 0.00 |
| Singlet | 0.02 | 0.06 | -0.01 | 0.02 | 0.07 | -0.01 |
| Triplet | 0.02 | 0.07 | -0.01 | 0.02 | 0.07 | -0.01 |

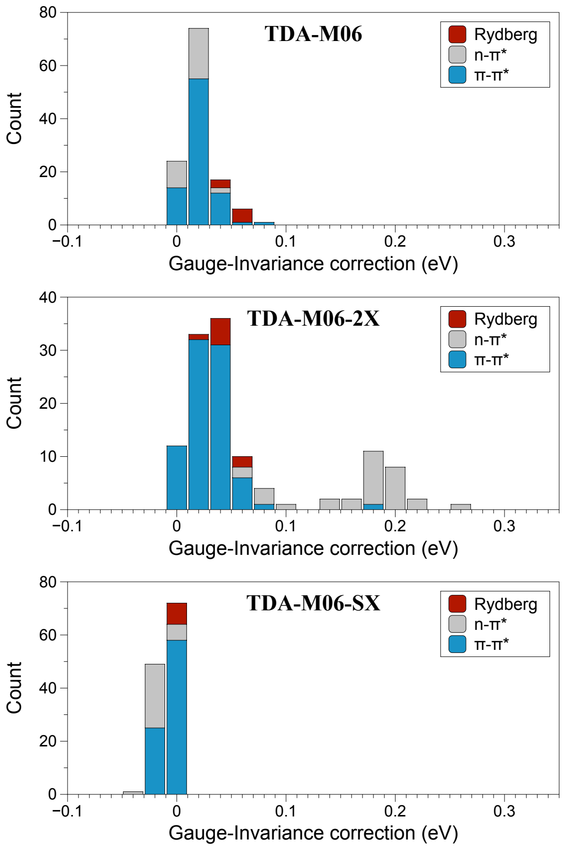


Figure S3: Impact of the gauge invariance corrections for three functionals at the TDA level.

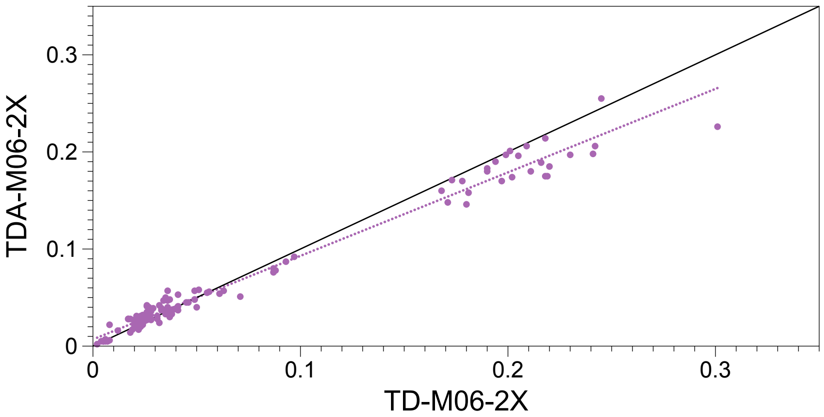


Figure S4: Correlation between the gauge invariance corrections obtained at TD-DFT and TDA levels with the M06-2X functional. All values are in eV. The central black line indicates perfect agreement, whereas the dashed purple line is the result of a linear fit.

## S5.2 TDA *versus* TD-DFT

Table S23: Mean difference between TDA-DFT and TD-DFT transition energies. The vast majority of corrections are positive, hence, the data in this Table essentially provide the TDA (average) upshift. All values are in eV

| | All | Sing. | Trip. | $\pi \rightarrow \pi^\star$ | $n \rightarrow \pi^\star$ | Ryd |
|---|---|---|---|---|---|---|
| TPSSh | 0.10 | 0.09 | 0.12 | 0.14 | 0.03 | 0.01 |
| $\tau$-HCTHhyb | 0.10 | 0.09 | 0.10 | 0.13 | 0.03 | 0.00 |
| B3LYP | 0.10 | 0.09 | 0.11 | 0.14 | 0.03 | 0.00 |
| PBE0 | 0.12 | 0.09 | 0.16 | 0.17 | 0.04 | 0.00 |
| cSCAN0 | 0.13 | 0.10 | 0.29 | 0.19 | 0.03 | 0.00 |
| M06 | 0.11 | 0.10 | 0.13 | 0.15 | 0.03 | 0.01 |
| cM06 | 0.11 | 0.10 | 0.13 | 0.16 | 0.03 | 0.00 |
| SOGGA11-X | 0.14 | 0.10 | 0.19 | 0.19 | 0.05 | 0.00 |
| BMK | 0.12 | 0.11 | 0.13 | 0.16 | 0.05 | 0.00 |
| MN15 | 0.12 | 0.11 | 0.12 | 0.16 | 0.04 | 0.01 |
| M08-HX | 0.11 | 0.11 | 0.11 | 0.14 | 0.06 | 0.01 |
| M06-2X | 0.12 | 0.12 | 0.12 | 0.15 | 0.06 | 0.00 |
| cM06-2X | 0.11 | 0.11 | 0.12 | 0.15 | 0.04 | 0.00 |
| M06-SX | 0.11 | 0.10 | 0.12 | 0.15 | 0.03 | 0.00 |
| cM06-SX | 0.11 | 0.10 | 0.12 | 0.15 | 0.03 | 0.00 |
| CAM-BLYP | 0.15 | 0.11 | 0.20 | 0.20 | 0.04 | 0.00 |
| tCAM-B3LYP | 0.09 | 0.09 | 0.09 | 0.13 | 0.03 | 0.00 |
| mCAM-BYLP | 0.12 | 0.10 | 0.15 | 0.16 | 0.04 | 0.01 |
| rCAM-B3LYP | 0.27 | 0.14 | 0.52 | 0.39 | 0.07 | 0.00 |
| $\omega$B97X-D | 0.14 | 0.11 | 0.18 | 0.19 | 0.04 | 0.00 |
| $\omega$B97M-V | 0.13 | 0.11 | 0.15 | 0.18 | 0.04 | 0.00 |
| $\omega$B97X | 0.17 | 0.12 | 0.25 | 0.24 | 0.04 | 0.00 |
| $\omega$B97 | 0.20 | 0.13 | 0.31 | 0.28 | 0.06 | 0.00 |
| LC-$\omega$PBE | 0.23 | 0.13 | 0.36 | 0.31 | 0.05 | 0.00 |
| M11 | 0.16 | 0.13 | 0.19 | 0.21 | 0.07 | 0.01 |
| B2PLYP | 0.08 | 0.08 | | 0.11 | 0.03 | 0.00 |
| PBE0-DH | 0.10 | 0.10 | | 0.13 | 0.04 | 0.00 |
| PBE-QIDH | 0.10 | 0.10 | | 0.13 | 0.04 | 0.00 |
| $\omega$B2PLYP | 0.12 | 0.12 | | 0.16 | 0.06 | 0.00 |
| RSH-0DH | 0.13 | 0.13 | | 0.18 | 0.06 | 0.00 |
| RSX-QIDH | 0.13 | 0.13 | | 0.16 | 0.07 | 0.00 |
| $\omega$B97X-2 | 0.08 | 0.08 | | 0.11 | 0.02 | 0.00 |
| SOS-wB88PP86 | 0.12 | 0.12 | | 0.16 | 0.06 | 0.00 |
| SOS-wPBEPP86 | 0.12 | 0.12 | | 0.16 | 0.05 | 0.00 |
| cLH12ct-SsirPW92 | 0.09 | 0.10 | 0.08 | 0.13 | 0.03 | 0.00 |
| cLH14t-calPBE | 0.11 | 0.09 | 0.12 | 0.14 | 0.03 | 0.00 |
| cLH20t | 0.10 | 0.10 | 0.10 | 0.13 | 0.03 | 0.00 |

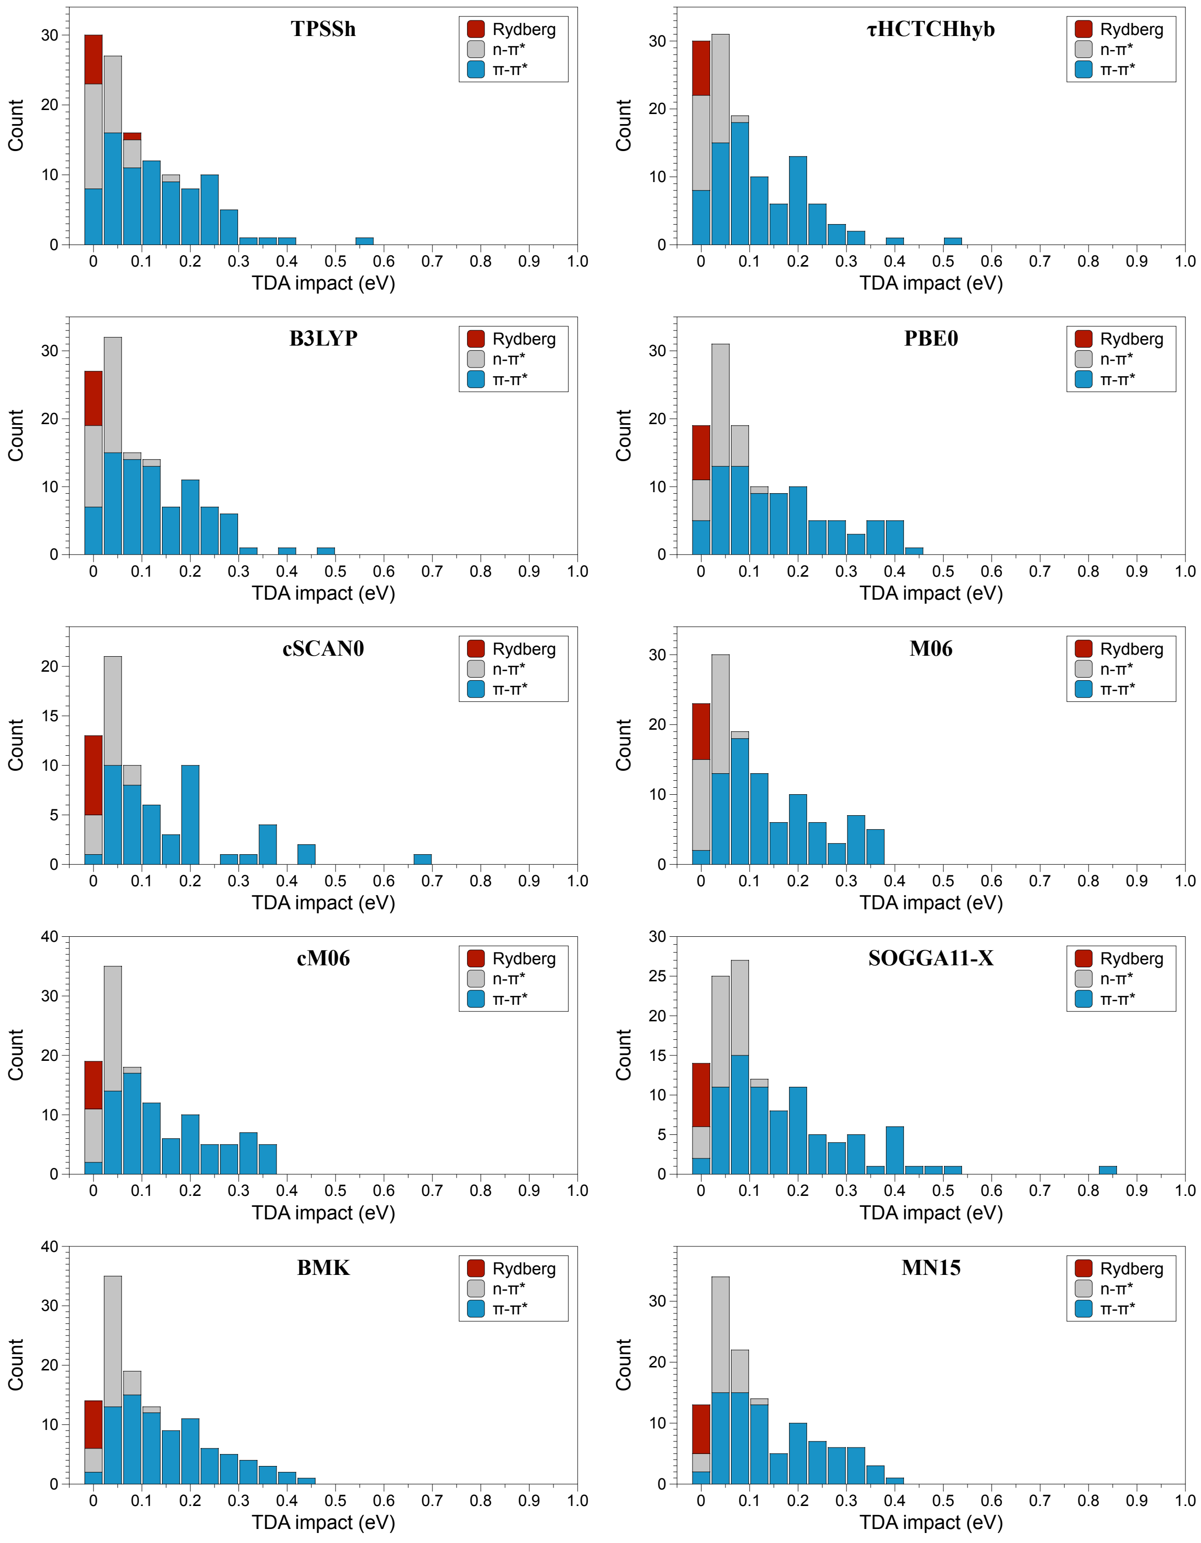


Figure S5: Impact of the TDA (in eV).

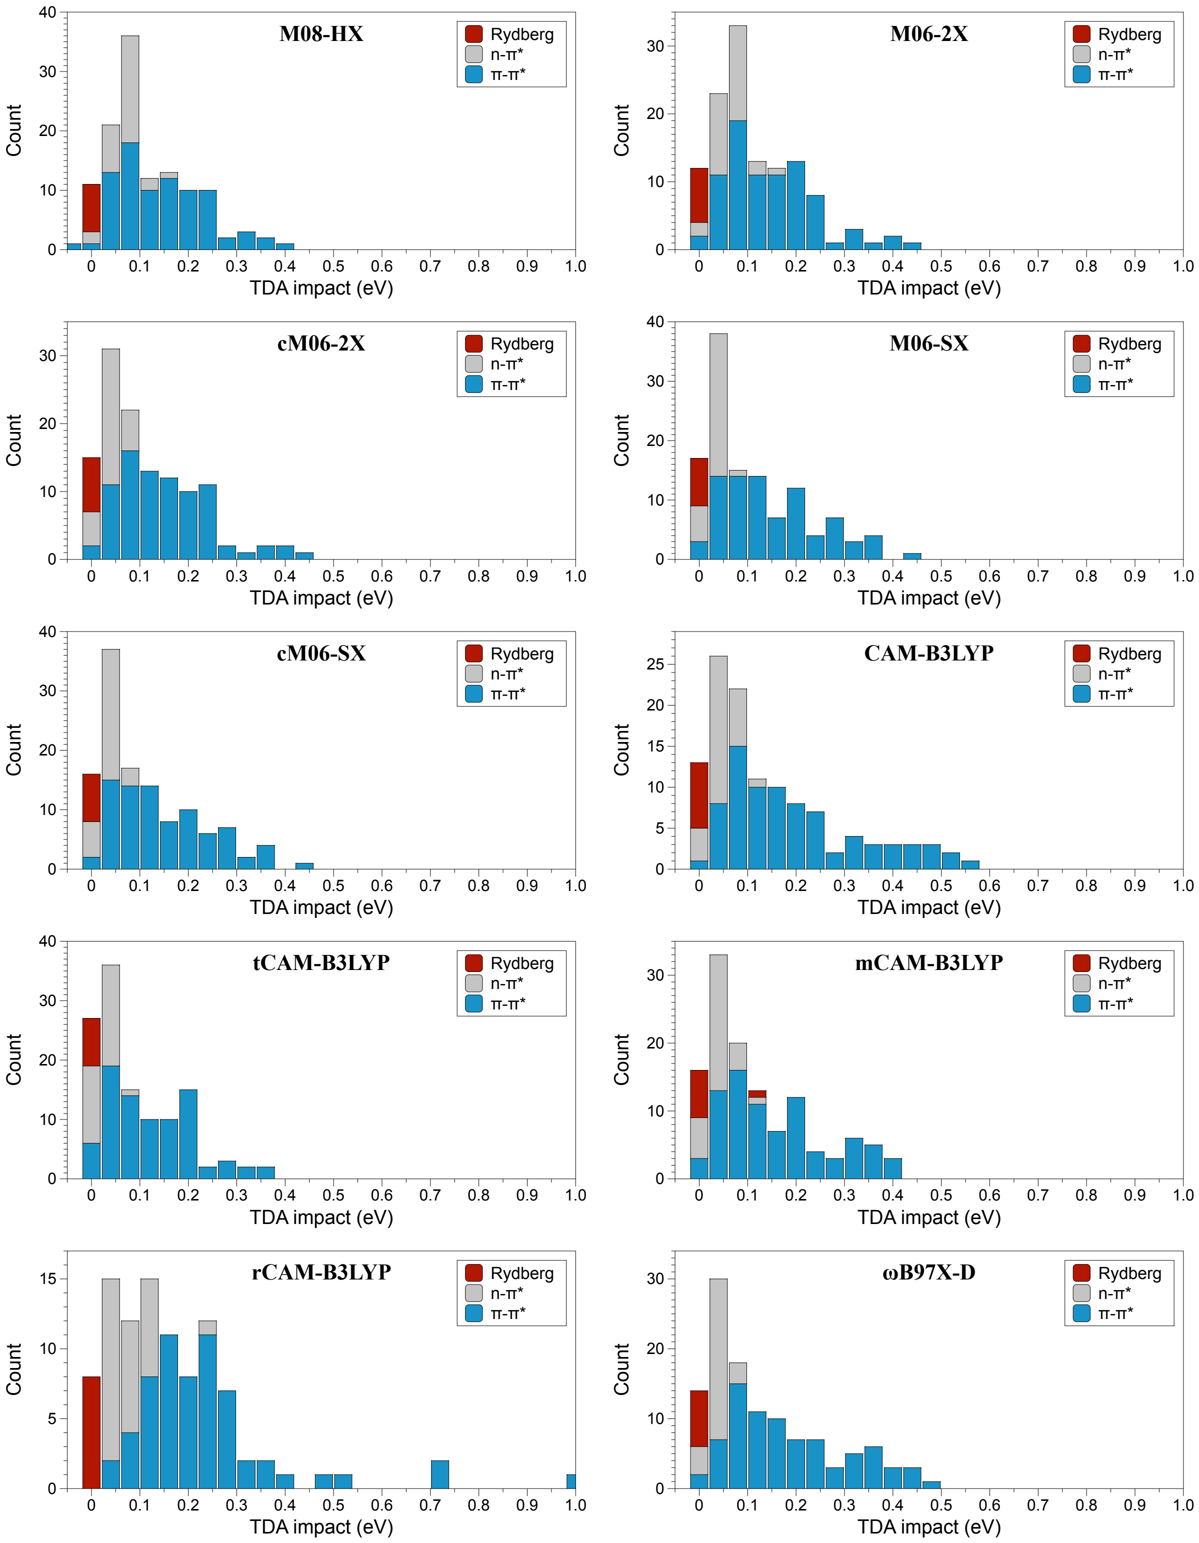


Figure S6: Impact of the TDA (in eV).

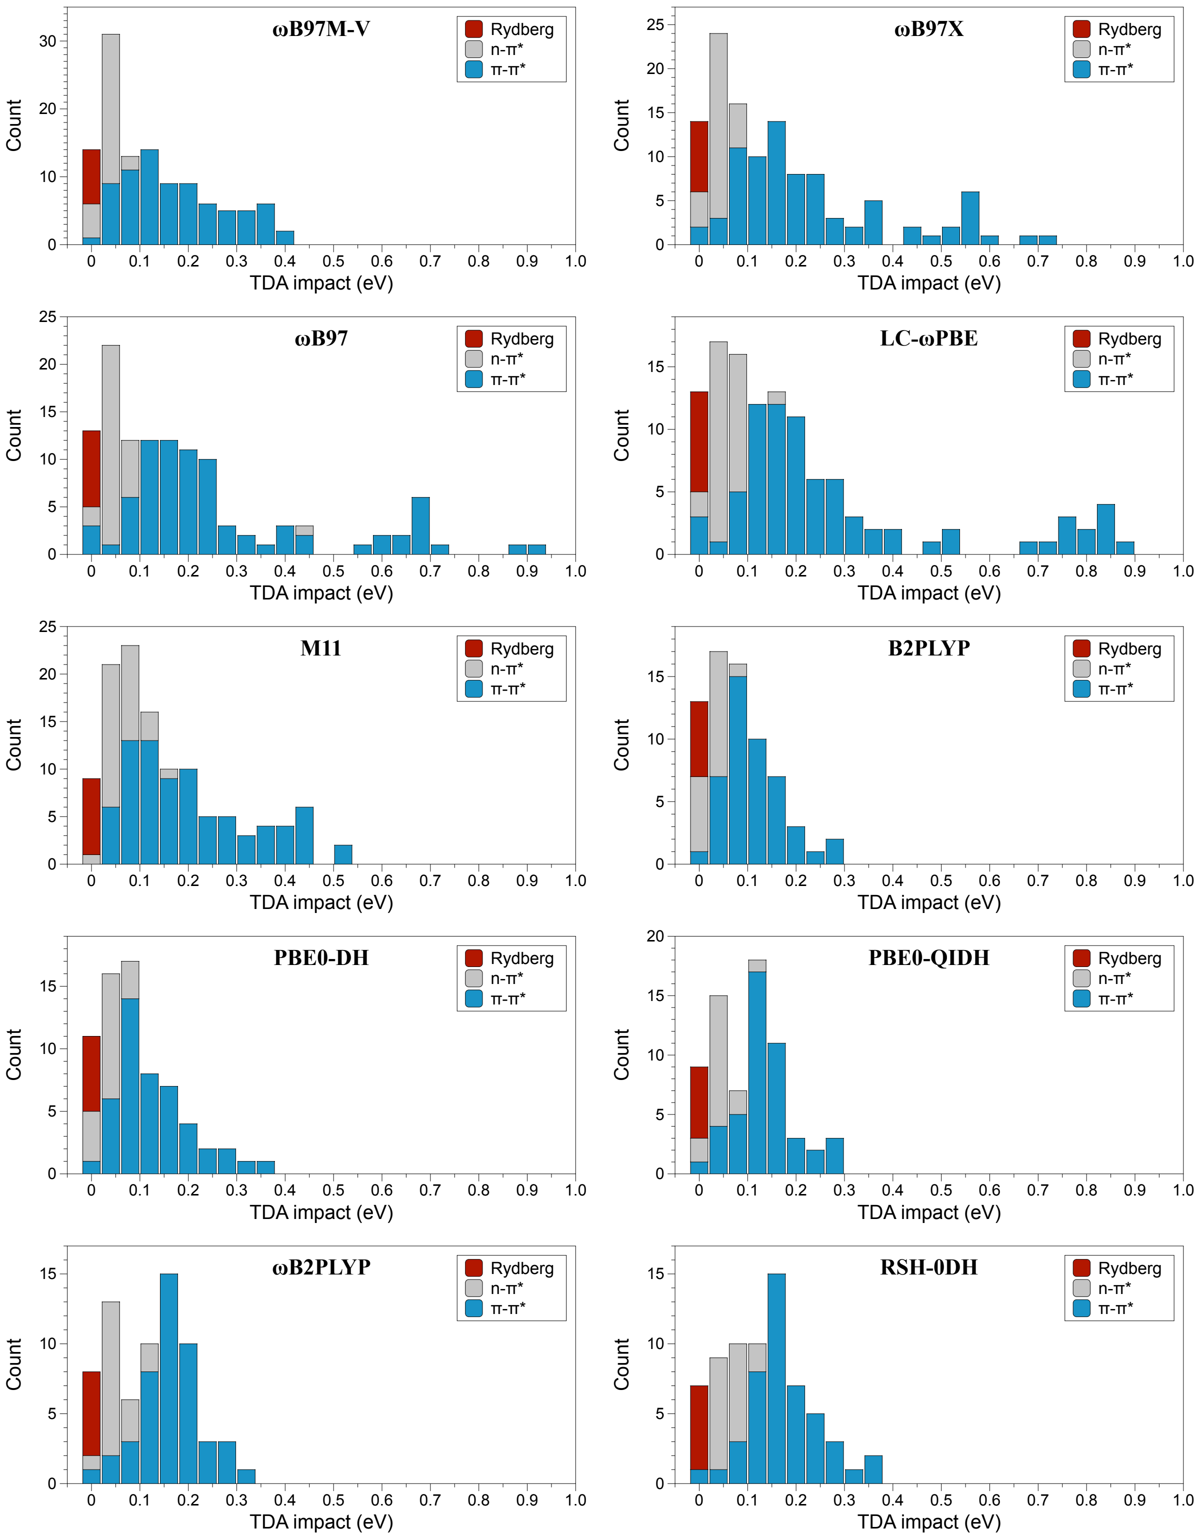


Figure S7: Impact of the TDA (in eV).

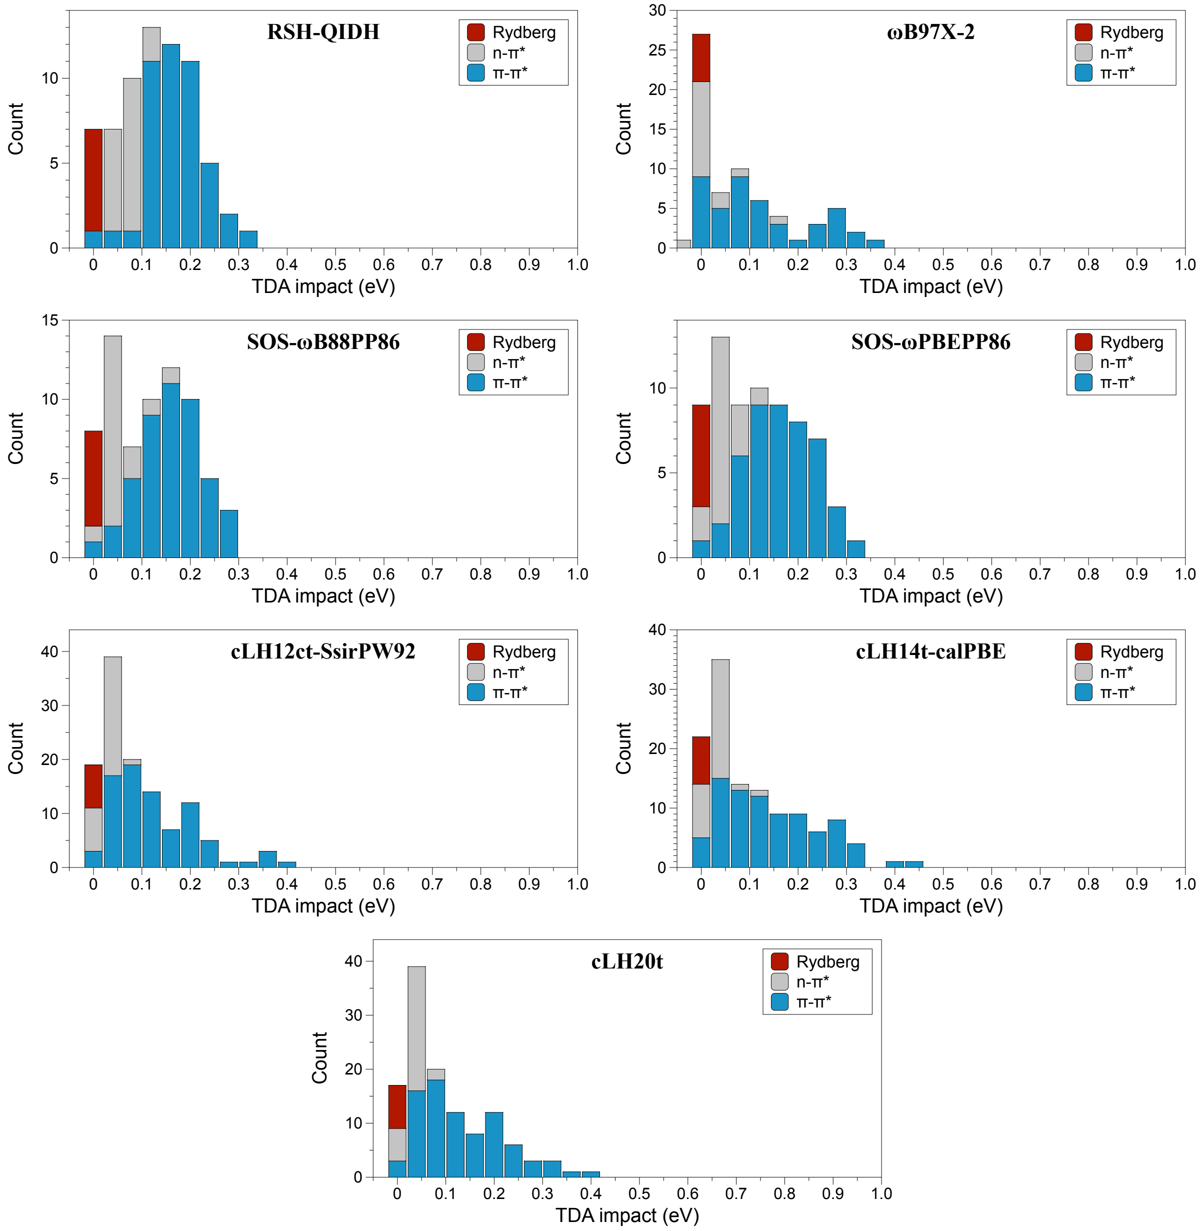


Figure S8: Impact of the TDA (in eV).

## S5.3 Error analysis

Table S24: Statistical analysis for TD-DFT methods. All values are in eV

| | Full set | | | MAE, subsets | | | | | |
|---|---|---|---|---|---|---|---|---|---|
| Method | MSE | MAE | SDE | Singlet | Triplet | $\pi \rightarrow \pi^\star$ | $n \rightarrow \pi^\star$ | Rydberg | $\%T_1 \geq 85\%$ |
| TPSSh | -0.44 | 0.47 | 0.28 | 0.43 | 0.52 | 0.44 | 0.61 | 0.26 | 0.48 |
| $\tau$-HCTHhyb | -0.39 | 0.42 | 0.27 | 0.40 | 0.46 | 0.41 | 0.54 | 0.18 | 0.43 |
| B3LYP | -0.35 | 0.38 | 0.23 | 0.34 | 0.43 | 0.37 | 0.41 | 0.30 | 0.39 |
| PBE0 | -0.28 | 0.34 | 0.26 | 0.25 | 0.45 | 0.35 | 0.34 | 0.15 | 0.35 |
| cSCAN0 | -0.07 | 0.27 | 0.28 | 0.24 | 0.48 | 0.32 | 0.14 | 0.30 | 0.29 |
| M06 | -0.36 | 0.39 | 0.28 | 0.37 | 0.40 | 0.36 | 0.29 | 1.01 | 0.41 |
| cM06 | -0.34 | 0.37 | 0.28 | 0.36 | 0.39 | 0.35 | 0.28 | 0.96 | 0.39 |
| SOGGA11-X | -0.03 | 0.23 | 0.27 | 0.23 | 0.23 | 0.25 | 0.18 | 0.17 | 0.22 |
| BMK | -0.02 | 0.20 | 0.23 | 0.20 | 0.19 | 0.21 | 0.16 | 0.19 | 0.19 |
| MN15 | -0.10 | 0.25 | 0.28 | 0.23 | 0.28 | 0.24 | 0.21 | 0.59 | 0.27 |
| M08-HX | 0.01 | 0.19 | 0.26 | 0.26 | 0.11 | 0.17 | 0.16 | 0.55 | 0.18 |
| M06-2X | 0.03 | 0.18 | 0.22 | 0.21 | 0.12 | 0.18 | 0.18 | 0.10 | 0.15 |
| cM06-2X | 0.09 | 0.17 | 0.21 | 0.24 | 0.09 | 0.18 | 0.18 | 0.09 | 0.14 |
| M06-SX | -0.07 | 0.22 | 0.25 | 0.22 | 0.23 | 0.23 | 0.18 | 0.36 | 0.23 |
| cM06-SX | -0.08 | 0.23 | 0.25 | 0.22 | 0.24 | 0.23 | 0.20 | 0.36 | 0.23 |
| CAM-BLYP | -0.06 | 0.25 | 0.29 | 0.19 | 0.33 | 0.29 | 0.16 | 0.10 | 0.24 |
| tCAM-B3LYP | -0.33 | 0.35 | 0.22 | 0.32 | 0.40 | 0.31 | 0.48 | 0.29 | 0.37 |
| mCAM-B3LYP | -0.23 | 0.28 | 0.23 | 0.21 | 0.38 | 0.31 | 0.24 | 0.19 | 0.30 |
| rCAM-B3LYP | 0.11 | 0.52 | 0.64 | 0.45 | 0.65 | 0.56 | 0.49 | 0.29 | 0.49 |
| $\omega$B97X-D | -0.02 | 0.24 | 0.27 | 0.21 | 0.27 | 0.26 | 0.14 | 0.34 | 0.23 |
| $\omega$B97M-V | 0.07 | 0.21 | 0.25 | 0.26 | 0.14 | 0.23 | 0.20 | 0.10 | 0.18 |
| $\omega$B97X | 0.10 | 0.32 | 0.37 | 0.34 | 0.29 | 0.33 | 0.21 | 0.63 | 0.29 |
| $\omega$B97 | 0.15 | 0.38 | 0.43 | 0.42 | 0.33 | 0.39 | 0.28 | 0.71 | 0.35 |
| LC-$\omega$PBE | 0.08 | 0.42 | 0.51 | 0.41 | 0.45 | 0.46 | 0.26 | 0.70 | 0.40 |
| M11 | 0.02 | 0.28 | 0.33 | 0.31 | 0.23 | 0.29 | 0.21 | 0.36 | 0.25 |
| B2PLYP | -0.18 | 0.20 | 0.15 | 0.20 | | 0.19 | 0.24 | 0.22 | 0.21 |
| PBE0-DH | 0.05 | 0.15 | 0.14 | 0.15 | | 0.18 | 0.07 | 0.11 | 0.14 |
| PBE-QIDH | 0.12 | 0.16 | 0.12 | 0.16 | | 0.15 | 0.17 | 0.19 | 0.13 |
| $\omega$B2PLYP | 0.26 | 0.27 | 0.19 | 0.27 | | 0.25 | 0.34 | 0.22 | 0.21 |
| RSH-0DH | 0.48 | 0.48 | 0.31 | 0.48 | | 0.43 | 0.56 | 0.66 | 0.42 |
| RSX-QIDH | 0.36 | 0.36 | 0.24 | 0.36 | | 0.32 | 0.44 | 0.48 | 0.31 |
| $\omega$B97X-2 | -0.43 | 0.47 | 0.37 | 0.47 | | 0.39 | 0.81 | 0.15 | 0.45 |
| SOS-$\omega$B88PP86 | 0.04 | 0.13 | 0.13 | 0.13 | | 0.11 | 0.13 | 0.30 | 0.11 |
| SOS-$\omega$PBEPP86 | 0.00 | 0.15 | 0.15 | 0.15 | | 0.13 | 0.12 | 0.38 | 0.15 |
| cLH12ct-SsirPW92 | -0.06 | 0.21 | 0.25 | 0.22 | 0.19 | 0.20 | 0.16 | 0.45 | 0.21 |
| cLH14t-calPBE | -0.25 | 0.32 | 0.26 | 0.26 | 0.39 | 0.33 | 0.32 | 0.20 | 0.33 |
| cLH20t | -0.09 | 0.19 | 0.21 | 0.18 | 0.20 | 0.22 | 0.13 | 0.13 | 0.19 |

Table S25: Statistical analysis for TDA-DFT methods. All values are in eV

| Method | MSE | MAE | SDE | Singlet | Triplet | $\pi \rightarrow \pi^\star$ | $n \rightarrow \pi^\star$ | Rydberg | $\%T_1 \geq 85\%$ |
|---|---|---|---|---|---|---|---|---|---|
| | Full set | | | MAE, subsets | | | | | |
| TPSSh | -0.34 | 0.39 | 0.31 | 0.39 | 0.40 | 0.34 | 0.58 | 0.26 | 0.39 |
| $\tau$-HCTHhyb | -0.30 | 0.36 | 0.29 | 0.36 | 0.36 | 0.32 | 0.51 | 0.18 | 0.35 |
| B3LYP | -0.25 | 0.31 | 0.26 | 0.30 | 0.32 | 0.28 | 0.38 | 0.30 | 0.31 |
| PBE0 | -0.16 | 0.26 | 0.25 | 0.24 | 0.29 | 0.25 | 0.30 | 0.15 | 0.25 |
| cSCAN0 | -0.15 | 0.34 | 0.38 | 0.23 | 0.47 | 0.38 | 0.21 | 0.30 | 0.34 |
| M06 | -0.25 | 0.31 | 0.31 | 0.34 | 0.28 | 0.26 | 0.27 | 1.01 | 0.31 |
| cM06 | -0.23 | 0.29 | 0.30 | 0.32 | 0.25 | 0.25 | 0.25 | 0.96 | 0.30 |
| SOGGA11-X | 0.11 | 0.20 | 0.24 | 0.28 | 0.10 | 0.21 | 0.17 | 0.17 | 0.17 |
| BMK | 0.10 | 0.19 | 0.23 | 0.24 | 0.11 | 0.20 | 0.14 | 0.20 | 0.16 |
| MN15 | 0.02 | 0.20 | 0.26 | 0.24 | 0.16 | 0.18 | 0.16 | 0.59 | 0.19 |
| M08-HX | 0.12 | 0.23 | 0.27 | 0.32 | 0.12 | 0.23 | 0.15 | 0.55 | 0.20 |
| M06-2X | 0.14 | 0.21 | 0.23 | 0.28 | 0.11 | 0.23 | 0.16 | 0.10 | 0.17 |
| cM06-2X | 0.21 | 0.23 | 0.20 | 0.32 | 0.12 | 0.25 | 0.21 | 0.09 | 0.19 |
| M06-SX | 0.04 | 0.19 | 0.25 | 0.23 | 0.13 | 0.19 | 0.15 | 0.37 | 0.17 |
| cM06-SX | 0.03 | 0.19 | 0.25 | 0.23 | 0.14 | 0.19 | 0.17 | 0.36 | 0.18 |
| CAM-BLYP | 0.08 | 0.19 | 0.23 | 0.24 | 0.13 | 0.22 | 0.15 | 0.10 | 0.16 |
| tCAM-B3LYP | -0.23 | 0.29 | 0.25 | 0.28 | 0.30 | 0.23 | 0.45 | 0.29 | 0.29 |
| mCAM-B3LYP | -0.11 | 0.21 | 0.22 | 0.20 | 0.23 | 0.22 | 0.21 | 0.17 | 0.20 |
| rCAM-B3LYP | 0.33 | 0.42 | 0.39 | 0.58 | 0.22 | 0.40 | 0.52 | 0.29 | 0.36 |
| $\omega$B97X-D | 0.11 | 0.20 | 0.23 | 0.27 | 0.11 | 0.22 | 0.14 | 0.34 | 0.17 |
| $\omega$B97M-V | 0.21 | 0.24 | 0.23 | 0.35 | 0.09 | 0.26 | 0.22 | 0.10 | 0.18 |
| $\omega$B97X | 0.26 | 0.30 | 0.28 | 0.45 | 0.10 | 0.29 | 0.23 | 0.63 | 0.24 |
| $\omega$B97 | 0.34 | 0.37 | 0.31 | 0.54 | 0.14 | 0.35 | 0.32 | 0.72 | 0.31 |
| LC-$\omega$PBE | 0.29 | 0.36 | 0.35 | 0.53 | 0.14 | 0.36 | 0.26 | 0.71 | 0.30 |
| M11 | 0.17 | 0.28 | 0.32 | 0.41 | 0.11 | 0.30 | 0.20 | 0.36 | 0.22 |
| B2PLYP | -0.11 | 0.15 | 0.16 | 0.17 | 0.13 | 0.12 | 0.24 | 0.18 | 0.14 |
| PBE0-DH | 0.04 | 0.16 | 0.20 | 0.18 | 0.13 | 0.18 | 0.12 | 0.15 | 0.15 |
| PBE-QIDH | 0.14 | 0.16 | 0.15 | 0.23 | 0.08 | 0.17 | 0.14 | 0.21 | 0.13 |
| $\omega$B2PLYP | 0.26 | 0.27 | 0.21 | 0.38 | 0.12 | 0.27 | 0.27 | 0.24 | 0.22 |
| RSH-0DH | 0.39 | 0.43 | 0.34 | 0.61 | 0.19 | 0.40 | 0.45 | 0.67 | 0.37 |
| RSX-QIDH | 0.34 | 0.35 | 0.24 | 0.48 | 0.17 | 0.32 | 0.39 | 0.49 | 0.30 |
| $\omega$B97X-2 | -0.16 | 0.42 | 0.50 | 0.41 | 0.43 | 0.33 | 0.71 | 0.17 | 0.40 |
| SOS-$\omega$B88PP86 | 0.09 | 0.12 | 0.15 | 0.16 | 0.07 | 0.10 | 0.12 | 0.33 | 0.09 |
| SOS-$\omega$PBEPP86 | 0.07 | 0.10 | 0.15 | 0.13 | 0.07 | 0.08 | 0.10 | 0.41 | 0.08 |
| cLH12ct-SsirPW92 | 0.03 | 0.19 | 0.25 | 0.23 | 0.14 | 0.18 | 0.14 | 0.45 | 0.17 |
| cLH14t-calPBE | -0.14 | 0.25 | 0.26 | 0.24 | 0.27 | 0.25 | 0.29 | 0.20 | 0.25 |
| cLH20t | 0.01 | 0.15 | 0.21 | 0.19 | 0.11 | 0.18 | 0.11 | 0.13 | 0.14 |

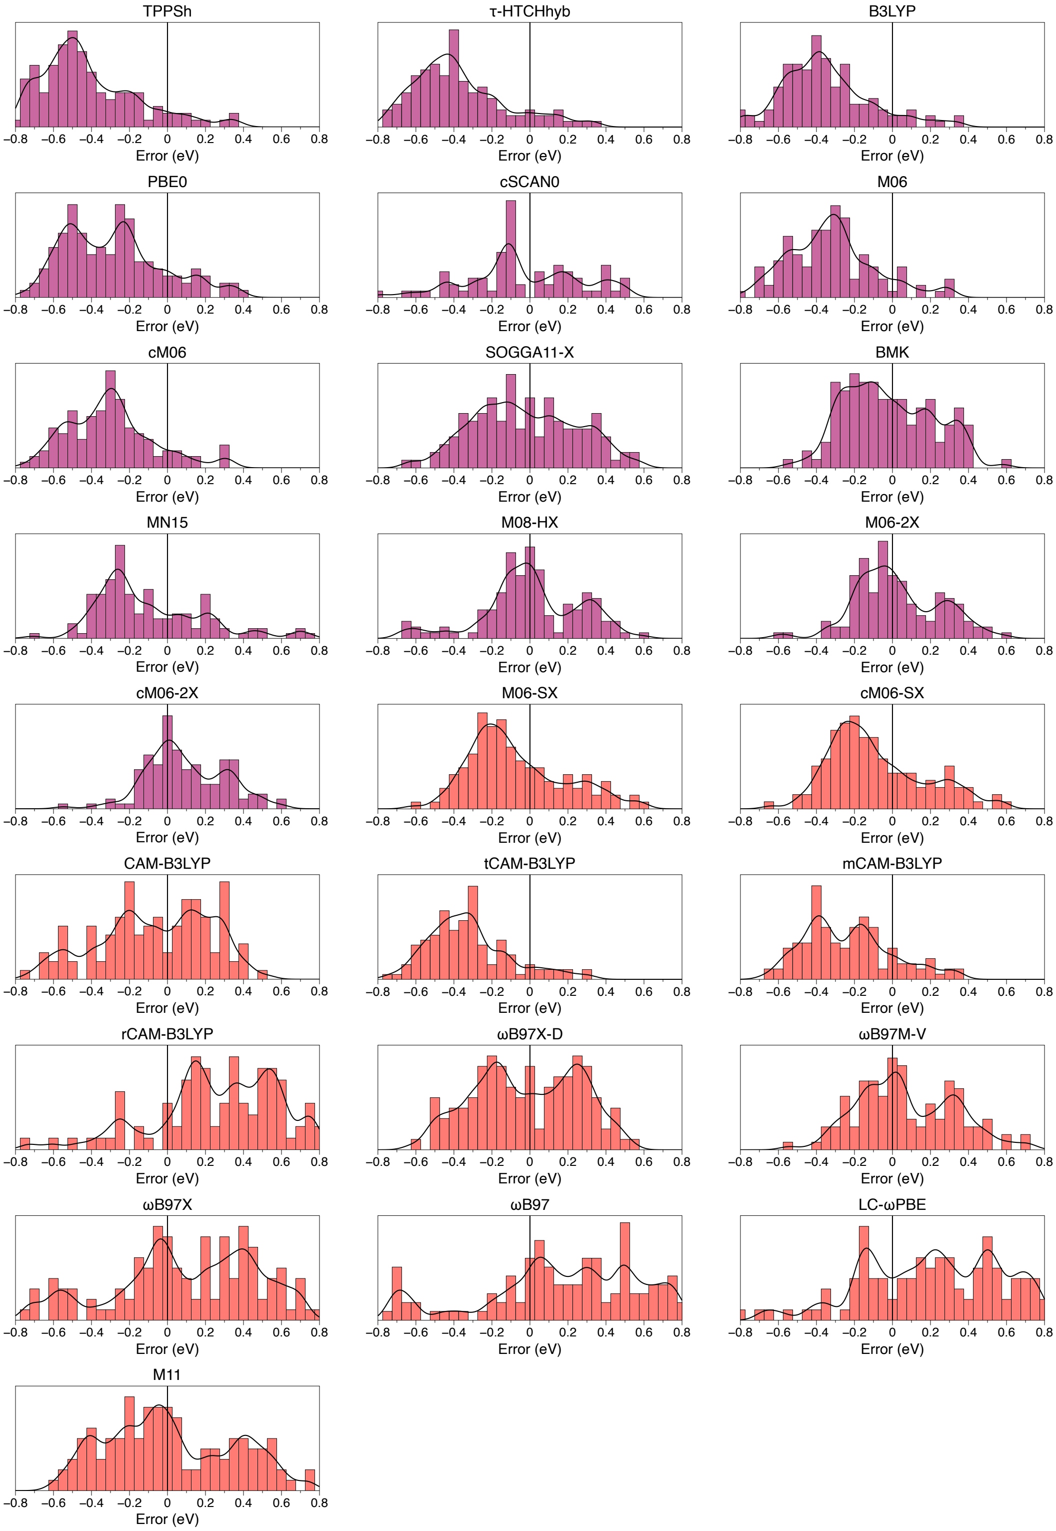


Figure S9: Histograms of the errors as compared to the TBEs for global and range-separated hybrids in TD-DFT.

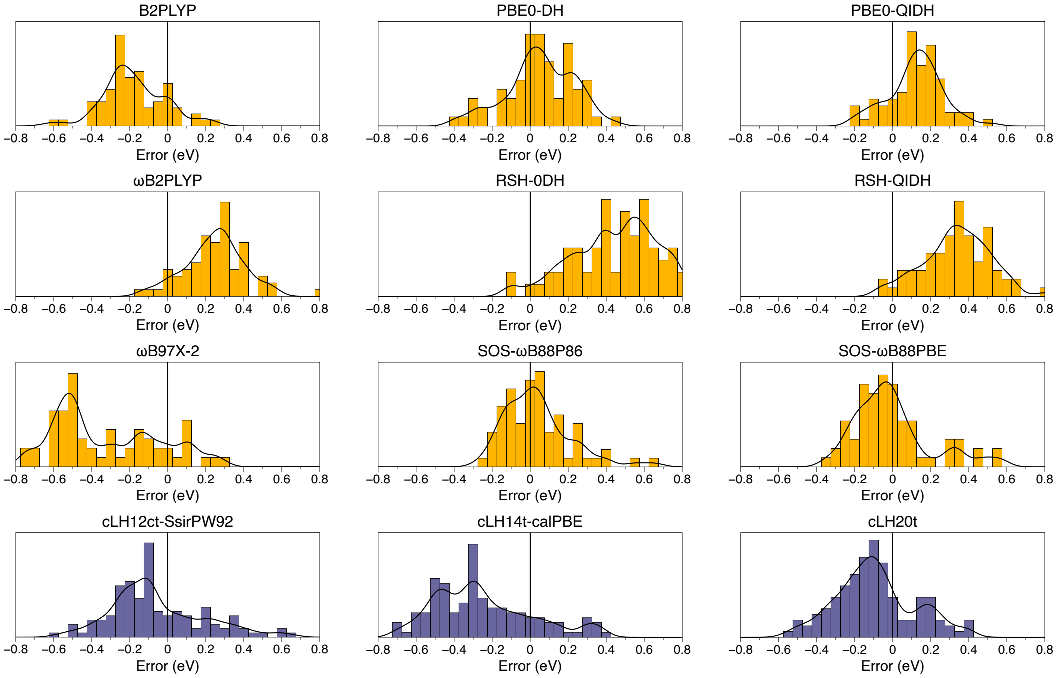


Figure S10: Histograms of the errors as compared to the TBEs for double and local hybrids in TD-DFT.

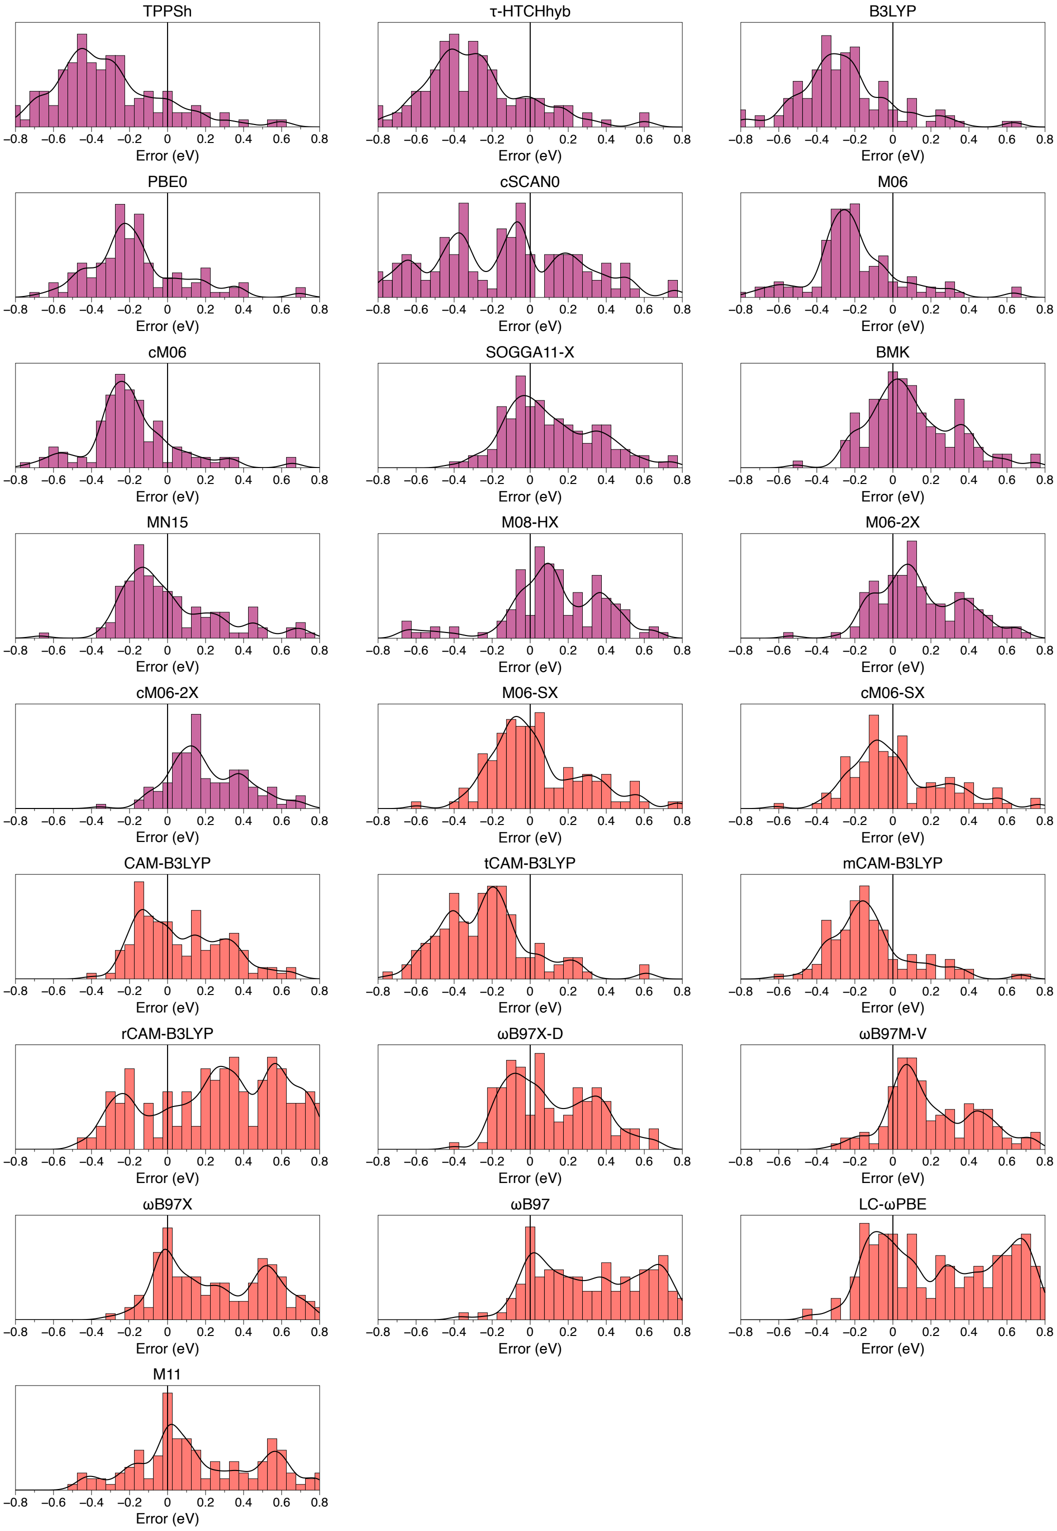


Figure S11: Histograms of the errors as compared to the TBEs for global and range-separated hybrids in TDA-DFT.

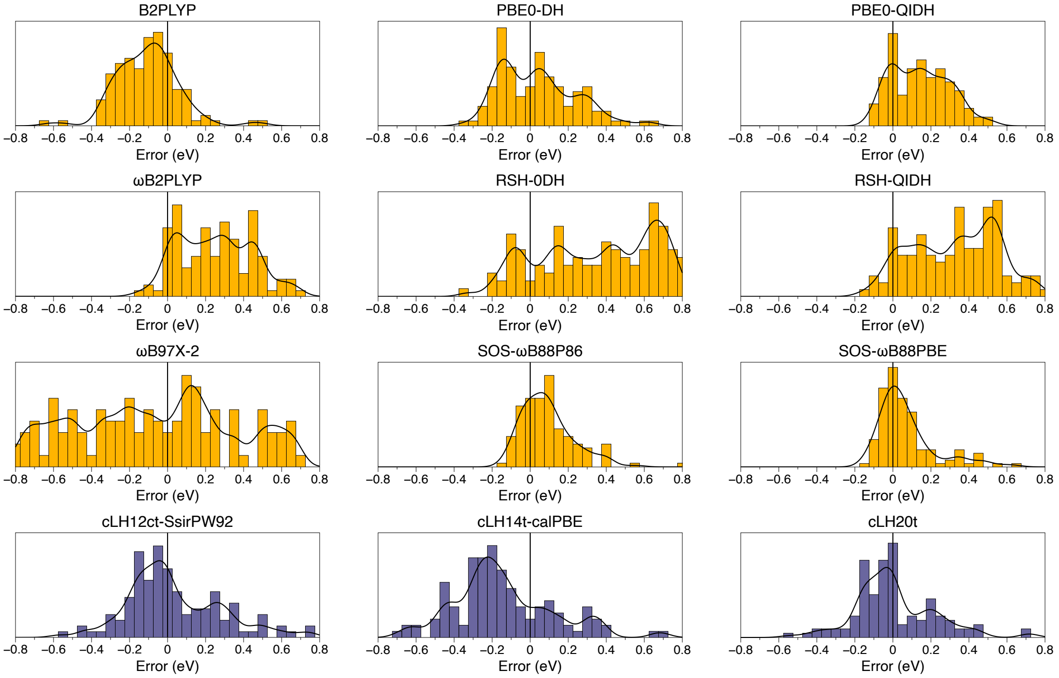


Figure S12: Histograms of the errors as compared to the TBEs for double and local hybrids in TDA-DFT.

# S6 Additional BSE/$GW$ data and analyses

## S6.1 $G_0W_0$ *vs* ev$GW$

Table S26: Mean difference between the transition energies determined starting with ev$GW$ instead of $G_0W_0$ in BSE calculations. All values are in eV

| | All | Sing. | Trip. | $\pi \rightarrow \pi^\star$ | $n \rightarrow \pi^\star$ | Ryd |
|---|---|---|---|---|---|---|
| BSE/$GW$@PBE0 | 0.36 | 0.40 | 0.29 | 0.31 | 0.52 | 0.18 |
| BSE/$GW$@CAM-B3LYP | 0.09 | 0.11 | 0.07 | 0.07 | 0.14 | 0.04 |
| BSE/$GW$@HF | -0.10 | -0.12 | -0.09 | -0.07 | -0.22 | -0.03 |
| TDA-BSE/$GW$@PBE0 | 0.37 | 0.40 | 0.33 | 0.33 | 0.52 | 0.18 |
| TDA-BSE/$GW$@CAM-B3LYP | 0.10 | 0.11 | 0.08 | 0.08 | 0.15 | 0.04 |
| TDA-BSE/$GW$@HF | -0.10 | -0.12 | -0.09 | -0.07 | -0.21 | -0.03 |

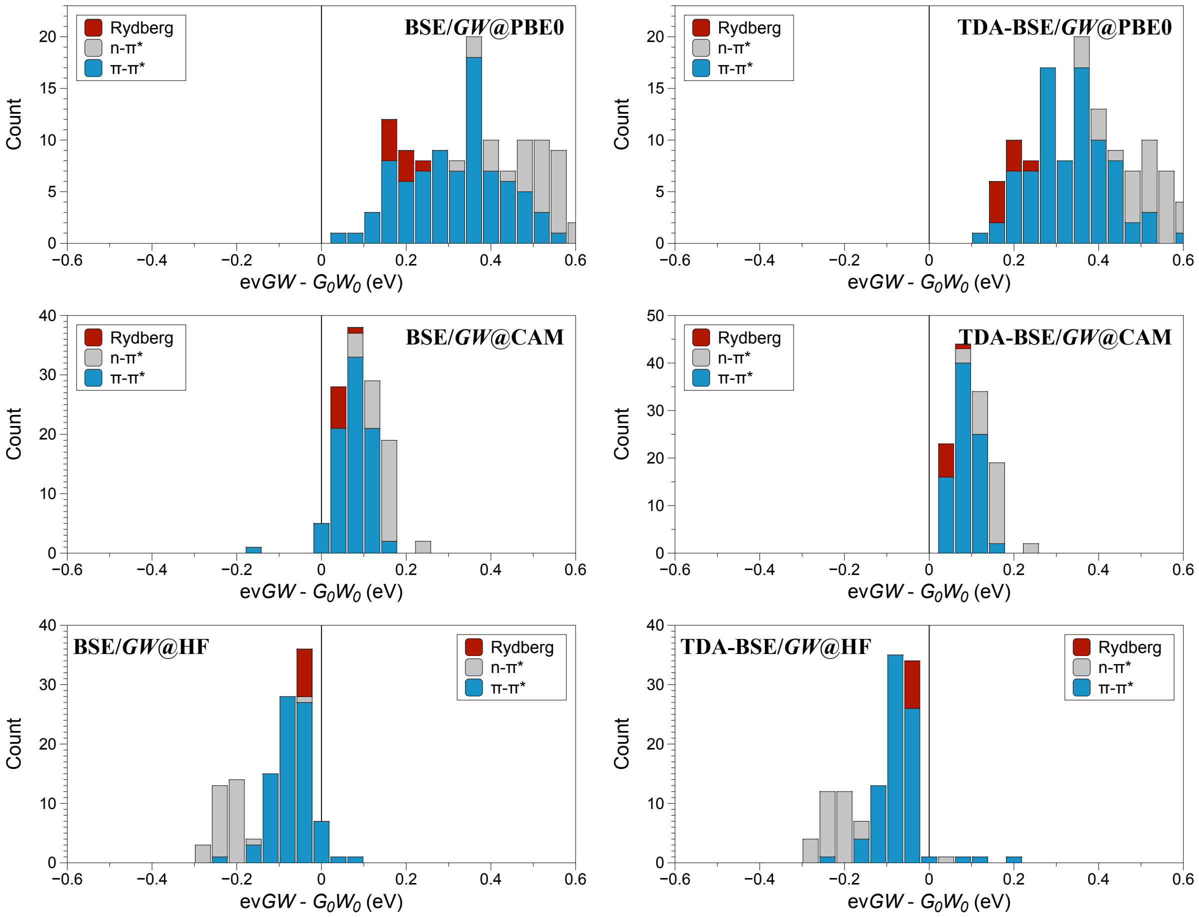


Figure S13: Difference between ev$GW$ and $G_0W_0$ transition energies (in eV).

## S6.2 TDA *versus* full-BSE

Table S27: Mean difference between TDA-BSE and full BSE transition energies. All corrections are positive, hence, the data in this Table therefore provide the TDA (average) upshift. All values are in eV

| | All | Sing. | Trip. | $\pi \to \pi^\star$ | $n \to \pi^\star$ | Ryd |
|---|---|---|---|---|---|---|
| BSE/$G_0W_0$@PBE0 | 0.11 | 0.12 | 0.11 | 0.15 | 0.04 | 0.00 |
| BSE/$G_0W_0$@CAM-B3LYP | 0.12 | 0.12 | 0.13 | 0.16 | 0.04 | 0.00 |
| BSE/$G_0W_0$@HF | 0.10 | 0.11 | 0.09 | 0.14 | 0.02 | 0.00 |
| BSE/ev$GW$@PBE0 | 0.13 | 0.12 | 0.14 | 0.17 | 0.04 | 0.00 |
| BSE/ev$GW$@CAM-B3LYP | 0.13 | 0.12 | 0.15 | 0.17 | 0.04 | 0.00 |
| BSE/ev$GW$@HF | 0.10 | 0.11 | 0.09 | 0.14 | 0.03 | 0.00 |

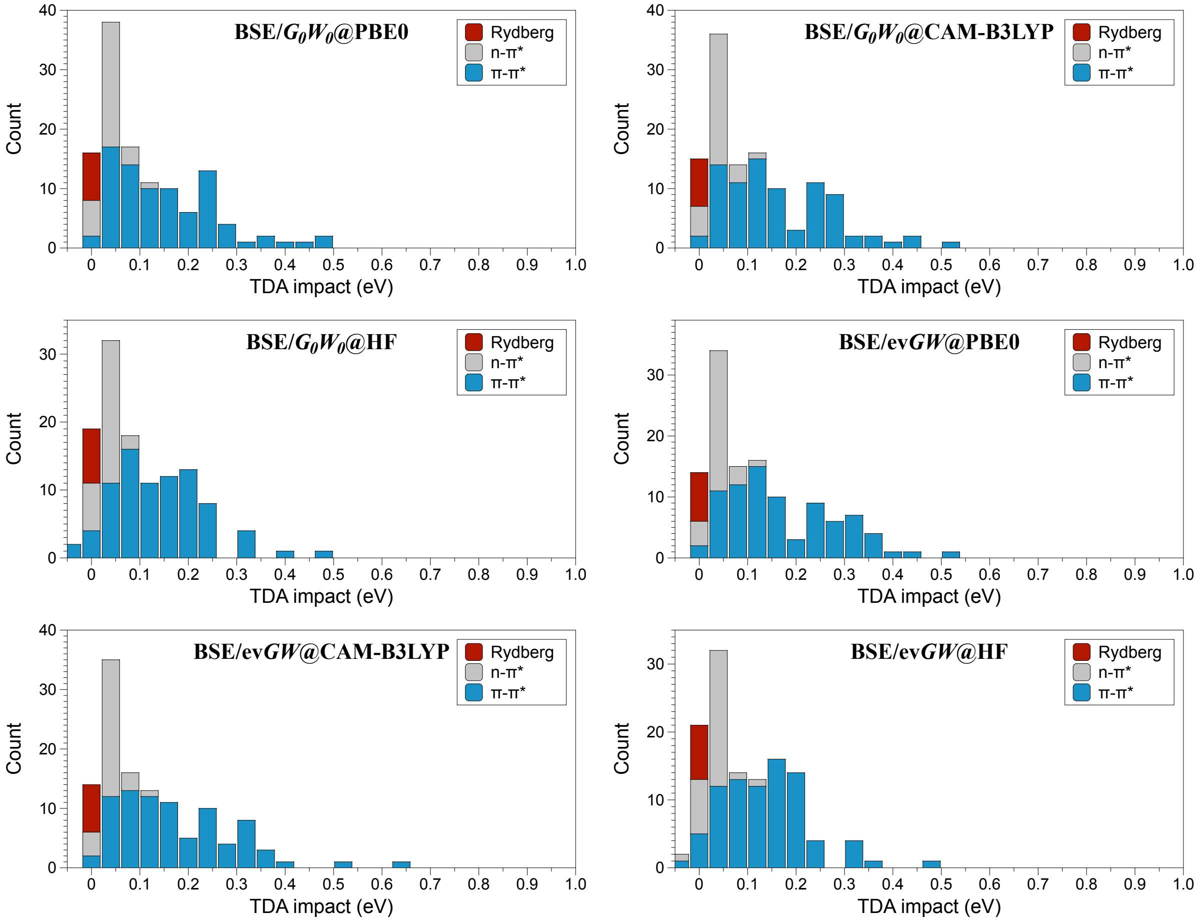


Figure S14: Impact of the TDA (in eV).

## S6.3 Starting point dependency

Table S28: Mean signed difference when using CAM-B3LYP instead of PBE0 as (starting) XCF. The vast majority of corrections are positive. TDA is not applied. All values are in eV

| | All | Sing. | Trip. | $\pi \to \pi^\star$ | $n \to \pi^\star$ | Ryd |
|---|---|---|---|---|---|---|
| BSE/$G_0W_0$ | 0.34 | 0.37 | 0.30 | 0.32 | 0.44 | 0.29 |
| BSE/ev$GW$ | 0.08 | 0.08 | 0.08 | 0.07 | 0.07 | 0.02 |
| TD-DFT | 0.22 | 0.27 | 0.14 | 0.18 | 0.34 | 0.14 |

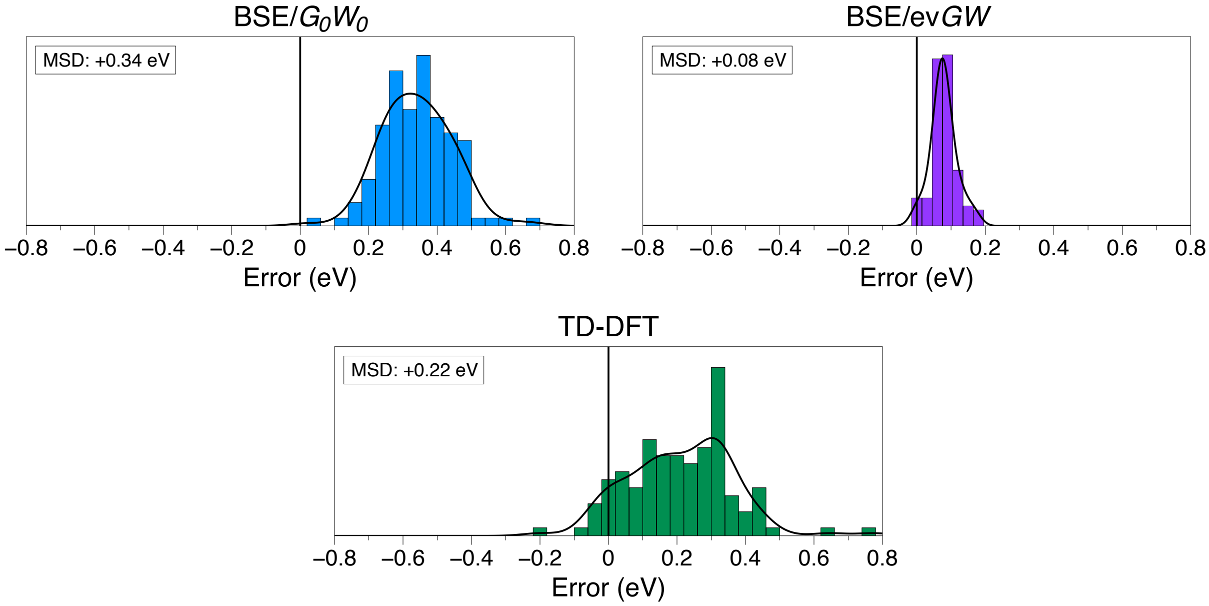


Figure S15: Impact of the using CAM-B3LYP instead of PBE0 as (starting) XCF (in eV). All calculations in 'full' (TDA not applied).

## S6.4 Error analysis

Table S29: Statistical analysis for BSE/$GW$ methods. All values are in eV

| | Full set | | | MAE, subsets | | | | | |
|---|---|---|---|---|---|---|---|---|---|
| Method | MSE | MAE | SDE | Singlet | Triplet | $\pi \rightarrow \pi^\star$ | $n \rightarrow \pi^\star$ | Rydberg | $\%T_1 \geq 85\%$ |
| | | | | Full-BSE | | | | | |
| BSE/$G_0W_0$@PBE0 | -0.69 | 0.69 | 0.20 | 0.57 | 0.84 | 0.69 | 0.76 | 0.43 | 0.71 |
| BSE/$G_0W_0$@CAM-B3LYP | -0.35 | 0.35 | 0.22 | 0.20 | 0.54 | 0.39 | 0.31 | 0.14 | 0.38 |
| BSE/$G_0W_0$@HF | 0.43 | 0.46 | 0.38 | 0.59 | 0.30 | 0.35 | 0.76 | 0.50 | 0.42 |
| BSE/ev$GW$@PBE0 | -0.33 | 0.34 | 0.24 | 0.18 | 0.54 | 0.38 | 0.26 | 0.25 | 0.37 |
| BSE/ev$GW$@CAM-B3LYP | -0.26 | 0.28 | 0.25 | 0.13 | 0.48 | 0.33 | 0.20 | 0.10 | 0.31 |
| BSE/ev$GW$@HF | 0.33 | 0.38 | 0.35 | 0.47 | 0.26 | 0.31 | 0.54 | 0.47 | 0.35 |
| | | | | TDA-BSE | | | | | |
| BSE/$G_0W_0$@PBE0 | -0.58 | 0.58 | 0.22 | 0.46 | 0.73 | 0.54 | 0.72 | 0.43 | 0.60 |
| BSE/$G_0W_0$@CAM-B3LYP | -0.23 | 0.25 | 0.20 | 0.13 | 0.42 | 0.25 | 0.28 | 0.14 | 0.28 |
| BSE/$G_0W_0$@HF | 0.53 | 0.55 | 0.35 | 0.69 | 0.36 | 0.46 | 0.78 | 0.50 | 0.50 |
| BSE/ev$GW$@PBE0 | -0.21 | 0.25 | 0.22 | 0.13 | 0.40 | 0.26 | 0.22 | 0.25 | 0.27 |
| BSE/ev$GW$@CAM-B3LYP | -0.13 | 0.20 | 0.21 | 0.11 | 0.33 | 0.23 | 0.17 | 0.10 | 0.21 |
| BSE/ev$GW$@HF | 0.43 | 0.45 | 0.31 | 0.57 | 0.28 | 0.40 | 0.57 | 0.47 | 0.41 |

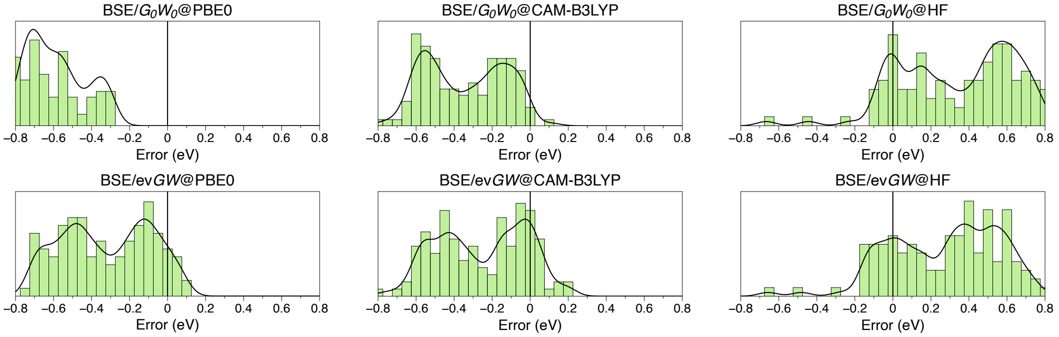


Figure S16: Histograms of the errors as compared to the TBE for full BSE/$GW$.

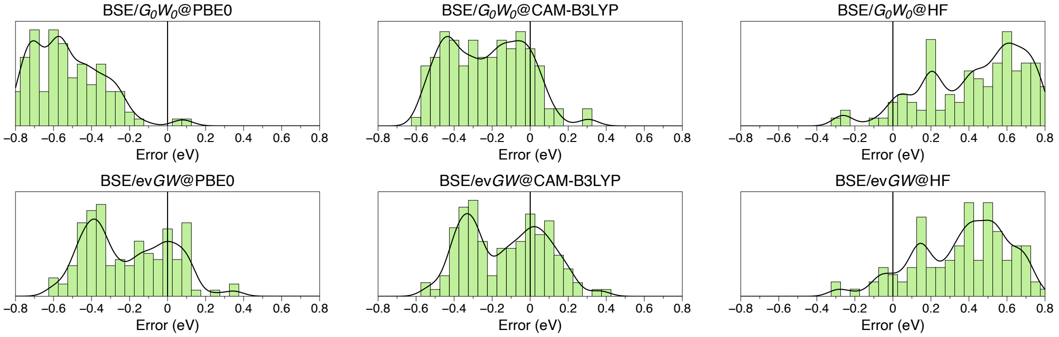


Figure S17: Histograms of the errors as compared to the TBE for TDA-BSE/$GW$

# S7 Geometries

Below, we provide the cartesian coordinates of the compounds investigated in this study. These are provided in atomic units (bohr) and have been obtained at the CCSD(T)/cc-pVTZ level (frozen-core approximation applied).

## S7.1 Anthracene

| | | | |
|---|---|---|---|
| C | 0.00000000 | 2.63580732 | 0.00000000 |
| C | 0.00000000 | -2.63580732 | 0.00000000 |
| C | -2.29791519 | 1.34956852 | 0.00000000 |
| C | 2.29791519 | 1.34956852 | 0.00000000 |
| C | -2.29791519 | -1.34956852 | 0.00000000 |
| C | 2.29791519 | -1.34956852 | 0.00000000 |
| C | -4.65745777 | 2.64726588 | 0.00000000 |
| C | 4.65745777 | 2.64726588 | 0.00000000 |
| C | -4.65745777 | -2.64726588 | 0.00000000 |
| C | 4.65745777 | -2.64726588 | 0.00000000 |
| C | -6.88218555 | 1.34593157 | 0.00000000 |
| C | 6.88218555 | 1.34593157 | 0.00000000 |
| C | -6.88218555 | -1.34593157 | 0.00000000 |
| C | 6.88218555 | -1.34593157 | 0.00000000 |
| H | 0.00000000 | 4.67946059 | 0.00000000 |
| H | 0.00000000 | -4.67946059 | 0.00000000 |
| H | -4.64776022 | 4.68790486 | 0.00000000 |
| H | 4.64776022 | 4.68790486 | 0.00000000 |
| H | -4.64776022 | -4.68790486 | 0.00000000 |
| H | 4.64776022 | -4.68790486 | 0.00000000 |
| H | -8.65488616 | 2.34873329 | 0.00000000 |
| H | 8.65488616 | 2.34873329 | 0.00000000 |
| H | -8.65488616 | -2.34873329 | 0.00000000 |
| H | 8.65488616 | -2.34873329 | 0.00000000 |

## S7.2 Anthraquinone

| | | | |
|---|---|---|---|
| C | 0.00000000 | 2.77266798 | 0.00000000 |
| C | 0.00000000 | -2.77266798 | 0.00000000 |
| C | -2.39604276 | 1.31893403 | 0.00000000 |
| C | 2.39604276 | 1.31893403 | 0.00000000 |
| C | -2.39604276 | -1.31893403 | 0.00000000 |
| C | 2.39604276 | -1.31893403 | 0.00000000 |
| C | -4.67770721 | 2.63091924 | 0.00000000 |
| C | 4.67770721 | 2.63091924 | 0.00000000 |
| C | -4.67770721 | -2.63091924 | 0.00000000 |
| C | 4.67770721 | -2.63091924 | 0.00000000 |
| C | -6.94595480 | 1.31915183 | 0.00000000 |
| C | 6.94595480 | 1.31915183 | 0.00000000 |
| C | -6.94595480 | -1.31915183 | 0.00000000 |
| C | 6.94595480 | -1.31915183 | 0.00000000 |
| O | 0.00000000 | 5.07701524 | 0.00000000 |
| O | 0.00000000 | -5.07701524 | 0.00000000 |
| H | -4.62532501 | 4.66594073 | 0.00000000 |
| H | 4.62532501 | 4.66594073 | 0.00000000 |
| H | -4.62532501 | -4.66594073 | 0.00000000 |
| H | 4.62532501 | -4.66594073 | 0.00000000 |
| H | -8.70925236 | 2.33764025 | 0.00000000 |
| H | 8.70925236 | 2.33764025 | 0.00000000 |
| H | -8.70925236 | -2.33764025 | 0.00000000 |
| H | 8.70925236 | -2.33764025 | 0.00000000 |

## S7.3 Aza-BODIPY

| | | | |
|---|---|---|---|
| B | 0.00000000 | 0.00000000 | 2.31704487 |
| C | 0.00000000 | 2.14450306 | -2.14127722 |
| C | 0.00000000 | -2.14450306 | -2.14127722 |
| C | 0.00000000 | 4.63460750 | -3.14651377 |
| C | 0.00000000 | -4.63460750 | -3.14651377 |
| C | 0.00000000 | 6.26996103 | -1.12023173 |
| C | 0.00000000 | -6.26996103 | -1.12023173 |
| C | 0.00000000 | 4.75475012 | 1.08608078 |
| C | 0.00000000 | -4.75475012 | 1.08608078 |
| N | 0.00000000 | 0.00000000 | -3.41527163 |
| N | 0.00000000 | 2.31056089 | 0.47890837 |
| N | 0.00000000 | -2.31056089 | 0.47890837 |
| F | -2.14709422 | 0.00000000 | 3.76825470 |
| F | 2.14709422 | 0.00000000 | 3.76825470 |
| H | 0.00000000 | 5.07027917 | -5.12686203 |
| H | 0.00000000 | -5.07027917 | -5.12686203 |
| H | 0.00000000 | 8.29623621 | -1.15574338 |
| H | 0.00000000 | -8.29623621 | -1.15574338 |
| H | 0.00000000 | 5.33784503 | 3.03195696 |
| H | 0.00000000 | -5.33784503 | 3.03195696 |

## S7.4 Azobenzene

| | | | |
|---|---|---|---|
| N | 0.70983759 | 0.94706332 | 0.00000000 |
| N | -0.70983759 | -0.94706332 | 0.00000000 |
| C | 3.32897155 | 0.35325415 | 0.00000000 |
| C | -3.32897155 | -0.35325415 | 0.00000000 |
| C | 4.95331207 | 2.41934773 | 0.00000000 |
| C | -4.95331207 | -2.41934773 | 0.00000000 |
| C | 4.29774859 | -2.10116089 | 0.00000000 |
| C | -4.29774859 | 2.10116089 | 0.00000000 |
| C | 7.55507717 | 2.05070219 | 0.00000000 |
| C | -7.55507717 | -2.05070219 | 0.00000000 |
| C | 6.89206075 | -2.45941610 | 0.00000000 |
| C | -6.89206075 | 2.45941610 | 0.00000000 |
| C | 8.52712206 | -0.38973890 | 0.00000000 |
| C | -8.52712206 | 0.38973890 | 0.00000000 |
| H | 4.14639892 | 4.28913452 | 0.00000000 |
| H | -4.14639892 | -4.28913452 | 0.00000000 |
| H | 3.00966091 | -3.67317406 | 0.00000000 |
| H | -3.00966091 | 3.67317406 | 0.00000000 |
| H | 8.81009192 | 3.65424541 | 0.00000000 |
| H | -8.81009192 | -3.65424541 | 0.00000000 |
| H | 7.65006326 | -4.35029611 | 0.00000000 |
| H | -7.65006326 | 4.35029611 | 0.00000000 |
| H | 10.54199682 | -0.68600884 | 0.00000000 |
| H | -10.54199682 | 0.68600884 | 0.00000000 |

## S7.5 BODIPY

| | | | |
|---|---|---|---|
| C | 0.00000000 | 0.00000000 | -3.45756235 |
| C | 0.00000000 | 2.28455780 | -2.18740413 |
| C | 0.00000000 | -2.28455780 | -2.18740413 |
| C | 0.00000000 | 4.79788592 | -3.09298460 |
| C | 0.00000000 | -4.79788592 | -3.09298460 |
| C | 0.00000000 | 6.36180283 | -0.99687598 |
| C | 0.00000000 | -6.36180283 | -0.99687598 |
| C | 0.00000000 | 4.76869637 | 1.13918303 |
| C | 0.00000000 | -4.76869637 | 1.13918303 |
| B | 0.00000000 | 0.00000000 | 2.22139632 |
| F | -2.14645956 | 0.00000000 | 3.68028136 |
| F | 2.14645956 | 0.00000000 | 3.68028136 |
| N | 0.00000000 | 2.34821228 | 0.42497916 |
| N | 0.00000000 | -2.34821228 | 0.42497916 |
| H | 0.00000000 | 5.33956943 | -5.04999407 |
| H | 0.00000000 | -5.33956943 | -5.04999407 |
| H | 0.00000000 | 8.38849882 | -0.96278552 |
| H | 0.00000000 | -8.38849882 | -0.96278552 |
| H | 0.00000000 | 5.26355675 | 3.10891537 |
| H | 0.00000000 | -5.26355675 | 3.10891537 |
| H | 0.00000000 | 0.00000000 | -5.49610864 |

## S7.6 Coumarin

| | | | |
|---|---|---|---|
| C | -4.94880904 | -1.94740654 | 0.00000000 |
| C | -2.47093848 | -2.79532569 | 0.00000000 |
| C | -0.51937217 | -1.03691944 | 0.00000000 |
| C | -1.01215298 | 1.55096378 | 0.00000000 |
| C | -3.52597295 | 2.36676114 | 0.00000000 |
| C | -5.48705921 | 0.63898323 | 0.00000000 |
| C | 1.12079288 | 3.23364340 | 0.00000000 |
| C | 3.48627701 | 2.30671360 | 0.00000000 |
| C | 3.97501526 | -0.40562242 | 0.00000000 |
| O | 1.88373948 | -1.96225124 | 0.00000000 |
| O | 6.03004743 | -1.37035420 | 0.00000000 |
| H | -6.46892150 | -3.30170531 | 0.00000000 |
| H | -2.01507343 | -4.77869214 | 0.00000000 |
| H | -3.90920136 | 4.37002329 | 0.00000000 |
| H | -7.41766766 | 1.28158133 | 0.00000000 |
| H | 0.79237605 | 5.24728088 | 0.00000000 |
| H | 5.13342919 | 3.49535270 | 0.00000000 |

## S7.7 Cyclazine

| | | | |
|---|---|---|---|
| N | 0.00000000 | 0.00000000 | 0.00000000 |
| C | 0.00000000 | -2.29619838 | 1.32571075 |
| C | 0.00000000 | -4.57380843 | -2.64068953 |
| C | 0.00000000 | 0.00000000 | -2.65142150 |
| C | 0.00000000 | 4.57380843 | -2.64068953 |
| C | 0.00000000 | 2.29619838 | 1.32571075 |
| C | 0.00000000 | 0.00000000 | 5.28137906 |
| C | 0.00000000 | -4.57334297 | -0.03501138 |
| C | 0.00000000 | 2.31699223 | -3.94312550 |
| C | 0.00000000 | 2.25635074 | 3.97813688 |
| C | 0.00000000 | -2.25635074 | 3.97813688 |
| C | 0.00000000 | -2.31699223 | -3.94312550 |
| C | 0.00000000 | 4.57334297 | -0.03501138 |
| H | 0.00000000 | 6.33829394 | -3.65941571 |
| H | 0.00000000 | 0.00000000 | 7.31883143 |
| H | 0.00000000 | -6.33829394 | -3.65941571 |
| H | 0.00000000 | -6.29930356 | 1.03947702 |
| H | 0.00000000 | 2.24943827 | -5.97509542 |
| H | 0.00000000 | 4.04986529 | 4.93561840 |
| H | 0.00000000 | -4.04986529 | 4.93561840 |
| H | 0.00000000 | -2.24943827 | -5.97509542 |
| H | 0.00000000 | 6.29930356 | 1.03947702 |

## S7.8 Heptazine

| | | | |
|---|---|---|---|
| C | 0.00000000 | -2.28707566 | 1.32044375 |
| C | 0.00000000 | -4.25961422 | -2.45928942 |
| C | 0.00000000 | 0.00000000 | -2.64088750 |
| C | 0.00000000 | 4.25961422 | -2.45928942 |
| C | 0.00000000 | 2.28707566 | 1.32044375 |
| C | 0.00000000 | 0.00000000 | 4.91857884 |
| N | 0.00000000 | 0.00000000 | 0.00000000 |
| N | 0.00000000 | -4.45372767 | 0.04447145 |
| N | 0.00000000 | 2.18835043 | -3.87927703 |
| N | 0.00000000 | 2.26537724 | 3.83480558 |
| N | 0.00000000 | -2.26537724 | 3.83480558 |
| N | 0.00000000 | -2.18835043 | -3.87927703 |
| N | 0.00000000 | 4.45372767 | 0.04447145 |
| H | 0.00000000 | 6.02612802 | -3.47918663 |
| H | 0.00000000 | 0.00000000 | 6.95837327 |
| H | 0.00000000 | -6.02612802 | -3.47918663 |

## S7.9 Naphthalimide

| | | | |
|---|---|---|---|
| C | 0.00000000 | 0.00000000 | 0.88414254 |
| C | 0.00000000 | 0.00000000 | 3.55510034 |
| C | 2.35632602 | 0.00000000 | -3.21426958 |
| C | -2.35632602 | 0.00000000 | -3.21426958 |
| C | 2.32275215 | 0.00000000 | -0.42671489 |
| C | -2.32275215 | 0.00000000 | -0.42671489 |
| C | 4.57007817 | 0.00000000 | 0.87369931 |
| C | -4.57007817 | 0.00000000 | 0.87369931 |
| C | 4.58083177 | 0.00000000 | 3.53384218 |
| C | -4.58083177 | 0.00000000 | 3.53384218 |
| C | 2.33984212 | 0.00000000 | 4.84532412 |
| C | -2.33984212 | 0.00000000 | 4.84532412 |
| N | 0.00000000 | 0.00000000 | -4.35793673 |
| O | 4.27090495 | 0.00000000 | -4.47823176 |
| O | -4.27090495 | 0.00000000 | -4.47823176 |
| H | 0.00000000 | 0.00000000 | -6.26502060 |
| H | 6.30814973 | 0.00000000 | -0.18744497 |
| H | -6.30814973 | 0.00000000 | -0.18744497 |
| H | 6.35338009 | 0.00000000 | 4.53440153 |
| H | -6.35338009 | 0.00000000 | 4.53440153 |
| H | 2.33715237 | 0.00000000 | 6.88533156 |
| H | -2.33715237 | 0.00000000 | 6.88533156 |

### S7.10 Naphthoquinone

| | | | |
|---|---|---|---|
| C | 0.00000000 | 1.31868219 | 5.07583353 |
| C | 0.00000000 | -1.31868219 | 5.07583353 |
| C | 0.00000000 | 2.63328396 | 2.80719633 |
| C | 0.00000000 | -2.63328396 | 2.80719633 |
| C | 0.00000000 | 1.31896773 | 0.52975242 |
| C | 0.00000000 | -1.31896773 | 0.52975242 |
| C | 0.00000000 | 2.74649968 | -1.88121997 |
| C | 0.00000000 | -2.74649968 | -1.88121997 |
| C | 0.00000000 | 1.26627836 | -4.24808471 |
| C | 0.00000000 | -1.26627836 | -4.24808471 |
| O | 0.00000000 | 5.05039066 | -1.94176133 |
| O | 0.00000000 | -5.05039066 | -1.94176133 |
| H | 0.00000000 | 2.33629038 | 6.83936996 |
| H | 0.00000000 | -2.33629038 | 6.83936996 |
| H | 0.00000000 | 4.66861735 | 2.75798976 |
| H | 0.00000000 | -4.66861735 | 2.75798976 |
| H | 0.00000000 | 2.35501749 | -5.96917497 |
| H | 0.00000000 | -2.35501749 | -5.96917497 |

## S7.11 Phenazine

| | | | |
|---|---|---|---|
| N | 0.00000000 | 2.68425897 | 0.00000000 |
| N | 0.00000000 | -2.68425897 | 0.00000000 |
| C | -2.14725285 | 1.35123660 | 0.00000000 |
| C | 2.14725285 | 1.35123660 | 0.00000000 |
| C | -2.14725285 | -1.35123660 | 0.00000000 |
| C | 2.14725285 | -1.35123660 | 0.00000000 |
| C | -4.49864069 | 2.66174043 | 0.00000000 |
| C | 4.49864069 | 2.66174043 | 0.00000000 |
| C | -4.49864069 | -2.66174043 | 0.00000000 |
| C | 4.49864069 | -2.66174043 | 0.00000000 |
| C | -6.71414814 | 1.34756473 | 0.00000000 |
| C | 6.71414814 | 1.34756473 | 0.00000000 |
| C | -6.71414814 | -1.34756473 | 0.00000000 |
| C | 6.71414814 | -1.34756473 | 0.00000000 |
| H | -4.44549427 | 4.69771133 | 0.00000000 |
| H | 4.44549427 | 4.69771133 | 0.00000000 |
| H | -4.44549427 | -4.69771133 | 0.00000000 |
| H | 4.44549427 | -4.69771133 | 0.00000000 |
| H | -8.49075377 | 2.34322156 | 0.00000000 |
| H | 8.49075377 | 2.34322156 | 0.00000000 |
| H | -8.49075377 | -2.34322156 | 0.00000000 |
| H | 8.49075377 | -2.34322156 | 0.00000000 |

## S7.12 Phthalimide

| | | | |
|---|---|---|---|
| C | 0.00000000 | 2.20210348 | 2.25054900 |
| C | 0.00000000 | -2.20210348 | 2.25054900 |
| C | 0.00000000 | 1.31050301 | -0.41254468 |
| C | 0.00000000 | -1.31050301 | -0.41254468 |
| C | 0.00000000 | 2.68001925 | -2.63336829 |
| C | 0.00000000 | -2.68001925 | -2.63336829 |
| C | 0.00000000 | 1.32018039 | -4.89183006 |
| C | 0.00000000 | -1.32018039 | -4.89183006 |
| N | 0.00000000 | 0.00000000 | 3.69708218 |
| O | 0.00000000 | 4.33361053 | 3.05657131 |
| O | 0.00000000 | -4.33361053 | 3.05657131 |
| H | 0.00000000 | 0.00000000 | 5.59565443 |
| H | 0.00000000 | 4.71538263 | -2.60774609 |
| H | 0.00000000 | -4.71538263 | -2.60774609 |
| H | 0.00000000 | 2.31561890 | -6.66791824 |
| H | 0.00000000 | -2.31561890 | -6.66791824 |

## S7.13 Tolan

| | | | |
|---|---|---|---|
| C | -1.14632202 | 0.00000000 | 0.00000000 |
| C | 1.14632202 | 0.00000000 | 0.00000000 |
| C | -3.83802475 | 0.00000000 | 0.00000000 |
| C | 3.83802475 | 0.00000000 | 0.00000000 |
| C | -5.17616712 | -2.27953873 | 0.00000000 |
| C | -5.17616712 | 2.27953873 | 0.00000000 |
| C | 5.17616712 | 2.27953873 | 0.00000000 |
| C | 5.17616712 | -2.27953873 | 0.00000000 |
| C | -7.79943938 | -2.27513115 | 0.00000000 |
| C | -7.79943938 | 2.27513115 | 0.00000000 |
| C | 7.79943938 | 2.27513115 | 0.00000000 |
| C | 7.79943938 | -2.27513115 | 0.00000000 |
| C | -9.12002539 | 0.00000000 | 0.00000000 |
| C | 9.12002539 | 0.00000000 | 0.00000000 |
| H | -4.14659821 | -4.03713330 | 0.00000000 |
| H | -4.14659821 | 4.03713330 | 0.00000000 |
| H | 4.14659821 | 4.03713330 | 0.00000000 |
| H | 4.14659821 | -4.03713330 | 0.00000000 |
| H | -8.81141954 | -4.04290254 | 0.00000000 |
| H | -8.81141954 | 4.04290254 | 0.00000000 |
| H | 8.81141954 | 4.04290254 | 0.00000000 |
| H | 8.81141954 | -4.04290254 | 0.00000000 |
| H | -11.15613663 | 0.00000000 | 0.00000000 |
| H | 11.15613663 | 0.00000000 | 0.00000000 |
